# Supplementary material for: Exploring Content Based Image Retrieval for Highly Imbalanced Melanoma Data using Style Transfer, Semantic Image Segmentation and Ensemble Learning
Source: arXiv:2110.06331 ancillary file (2021-10-12)

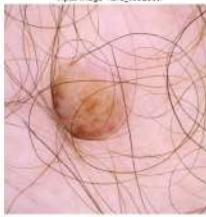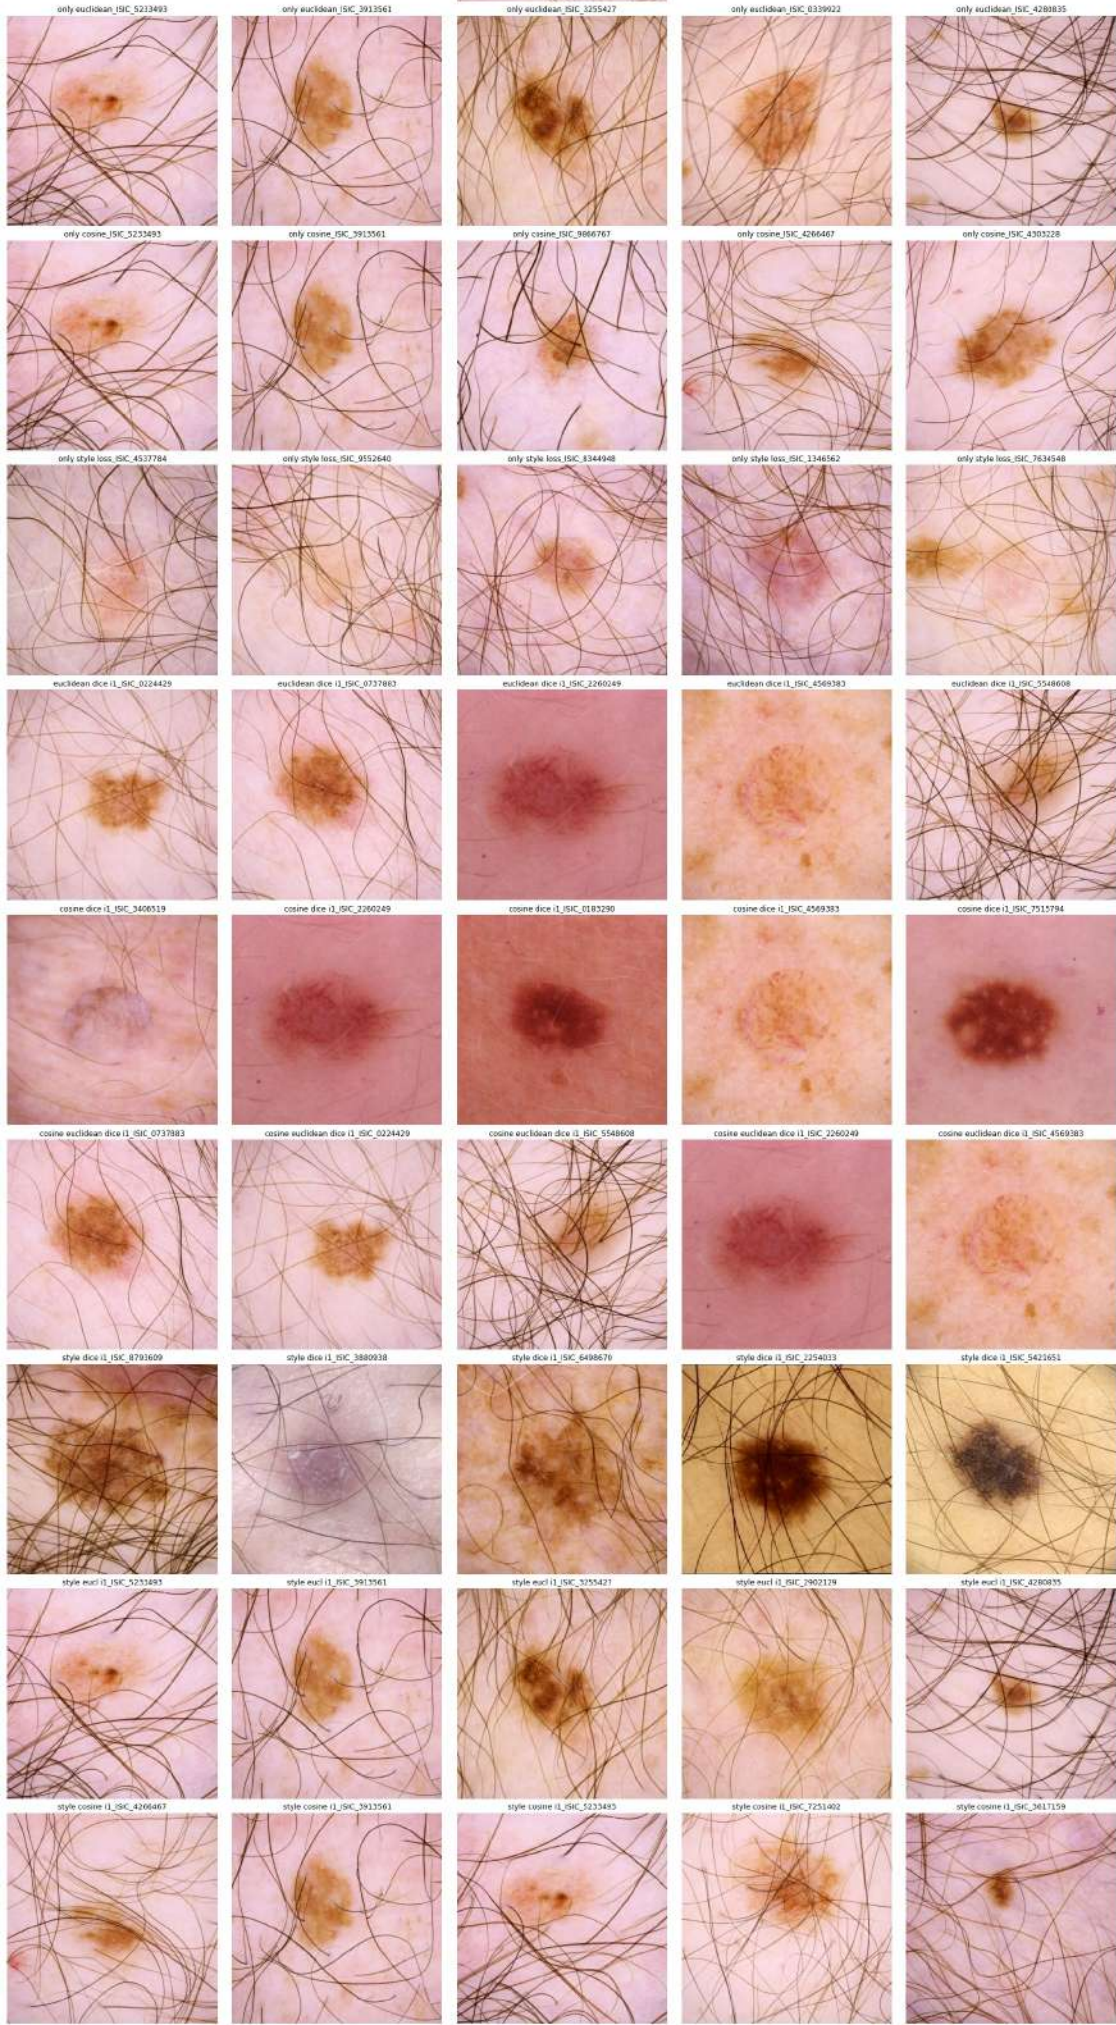

Input image - ISIC\_0052349

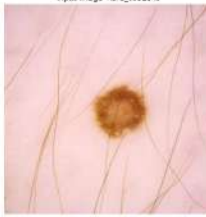

only euclidean\_ISIC\_3022527

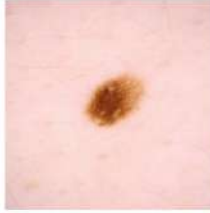

only euclidean\_ISIC\_4768236

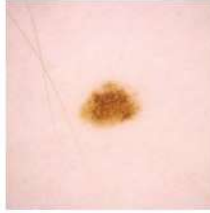

only euclidean\_ISIC\_2331415

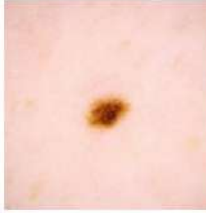

only euclidean\_ISIC\_9879041

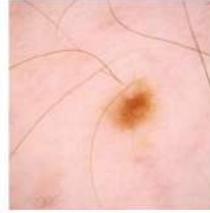

only euclidean\_ISIC\_4307871

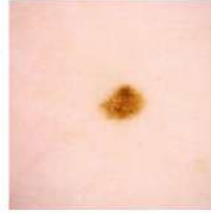

only cosine\_ISIC\_4768236

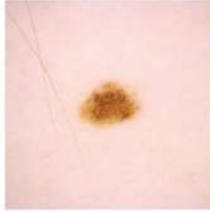

only cosine\_ISIC\_0256715

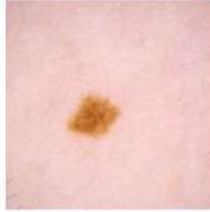

only cosine\_ISIC\_7026849

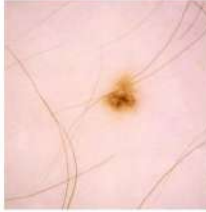

only cosine\_ISIC\_2331415

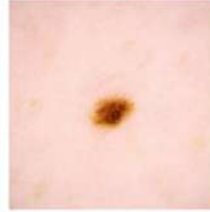

only cosine\_ISIC\_3022527

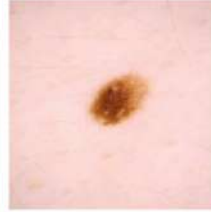

only style loss\_ISIC\_8754690

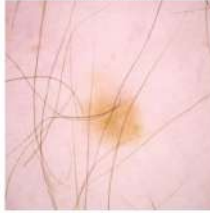

only style loss\_ISIC\_6287600

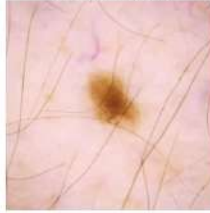

only style loss\_ISIC\_3623368

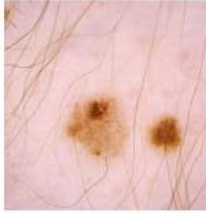

only style loss\_ISIC\_2964397

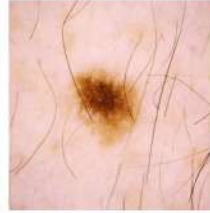

only style loss\_ISIC\_3281246

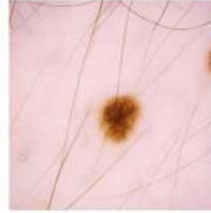

euclidean dice l1\_ISIC\_4578709

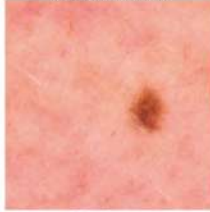

euclidean dice l1\_ISIC\_0324255

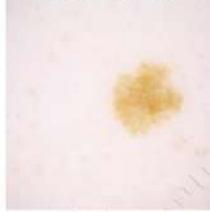

euclidean dice l1\_ISIC\_3622629

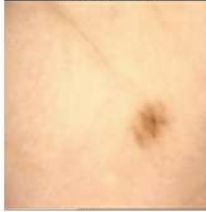

euclidean dice l1\_ISIC\_7661236

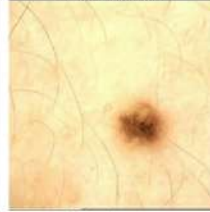

euclidean dice l1\_ISIC\_2681497

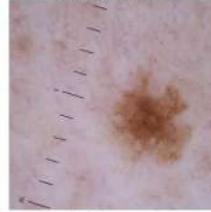

cosine dice l1\_ISIC\_2681497

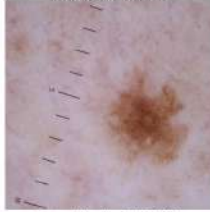

cosine dice l1\_ISIC\_4578709

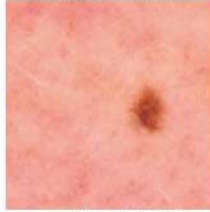

cosine dice l1\_ISIC\_0737951

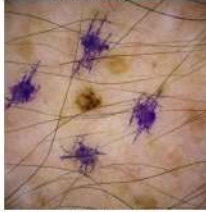

cosine dice l1\_ISIC\_8904170

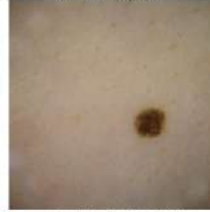

cosine dice l1\_ISIC\_2550948

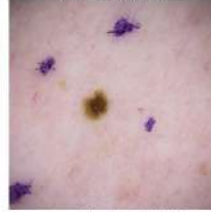

cosine euclidean dice l1\_ISIC\_4578709

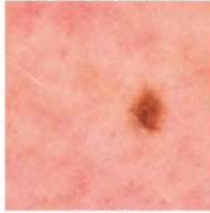

cosine euclidean dice l1\_ISIC\_0324255

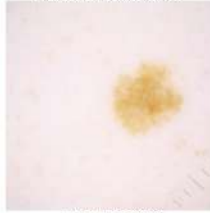

cosine euclidean dice l1\_ISIC\_3622629

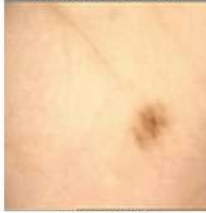

cosine euclidean dice l1\_ISIC\_7661236

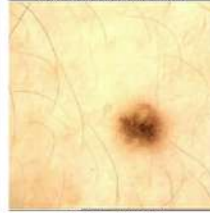

cosine euclidean dice l1\_ISIC\_4629020

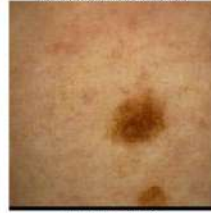

style dice l1\_ISIC\_8451738

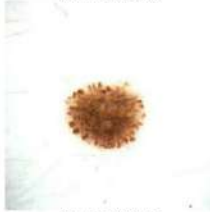

style dice l1\_ISIC\_2681497

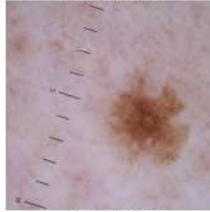

style dice l1\_ISIC\_0737951

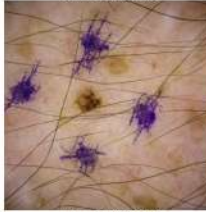

style dice l1\_ISIC\_8966170

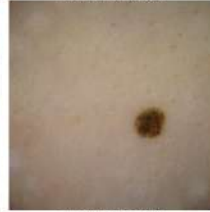

style dice l1\_ISIC\_6516658

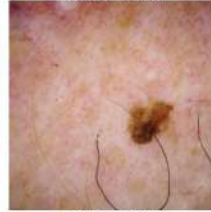

style eucl l1\_ISIC\_9191776

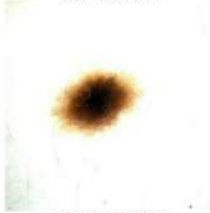

style eucl l1\_ISIC\_3022527

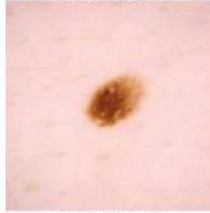

style eucl l1\_ISIC\_4768236

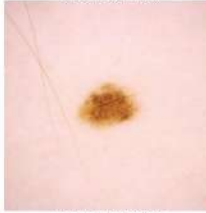

style eucl l1\_ISIC\_2331415

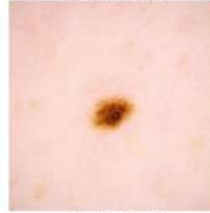

style eucl l1\_ISIC\_9879041

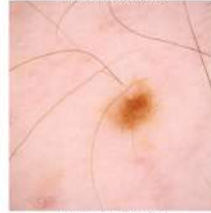

style cosine l1\_ISIC\_7926849

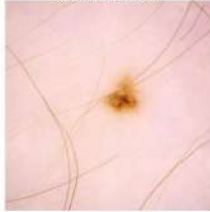

style cosine l1\_ISIC\_1438269

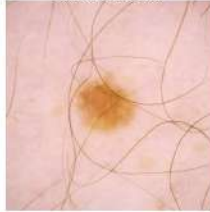

style cosine l1\_ISIC\_5612435

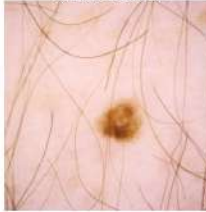

style cosine l1\_ISIC\_4768236

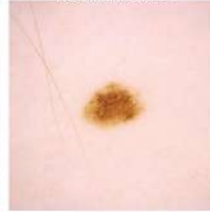

style cosine l1\_ISIC\_9879041

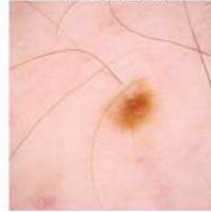

Input image - ISIC\_0258533

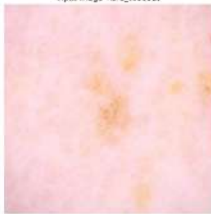

only euclidean\_ISIC\_7053159

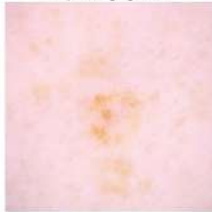

only euclidean\_ISIC\_0484163

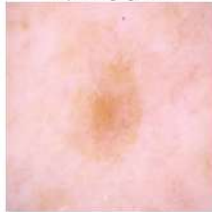

only euclidean\_ISIC\_4452104

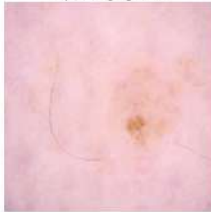

only euclidean\_ISIC\_8843217

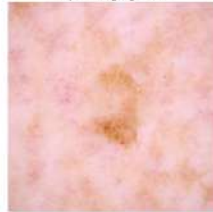

only euclidean\_ISIC\_6296647

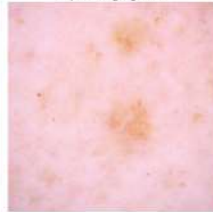

only cosine\_ISIC\_7053159

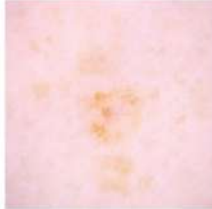

only cosine\_ISIC\_5557588

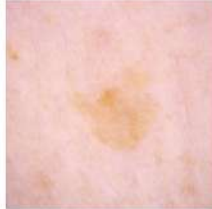

only cosine\_ISIC\_6347649

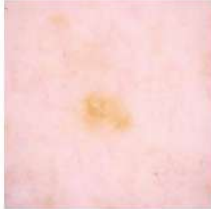

only cosine\_ISIC\_0422061

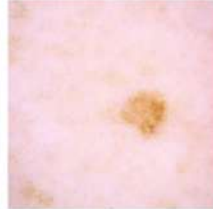

only cosine\_ISIC\_2346202

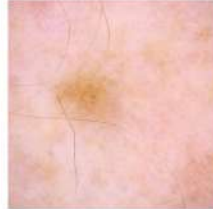

only style loss\_ISIC\_7053159

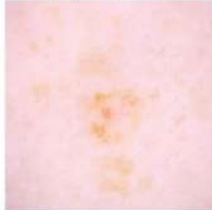

only style loss\_ISIC\_6268034

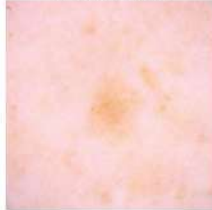

only style loss\_ISIC\_6263662

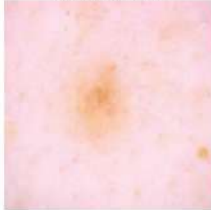

only style loss\_ISIC\_2978327

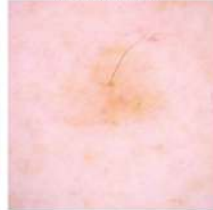

only style loss\_ISIC\_6341036

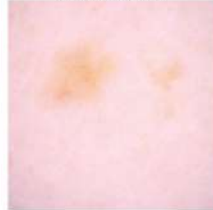

euclidean dice l1\_ISIC\_0484163

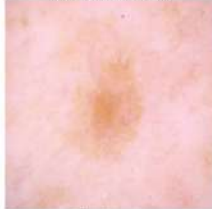

euclidean dice l1\_ISIC\_7725628

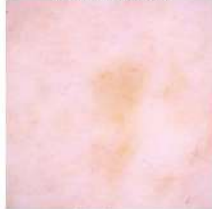

euclidean dice l1\_ISIC\_0963211

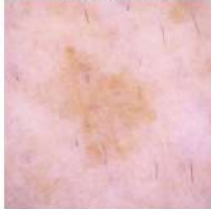

euclidean dice l1\_ISIC\_8280776

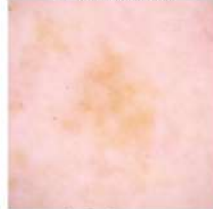

euclidean dice l1\_ISIC\_5721613

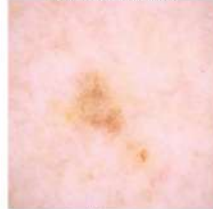

cosine dice l1\_ISIC\_0484163

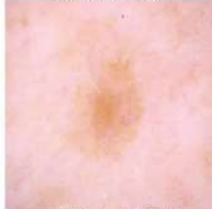

cosine dice l1\_ISIC\_7725628

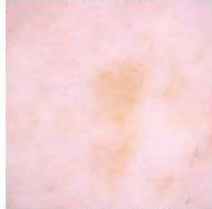

cosine dice l1\_ISIC\_0026682

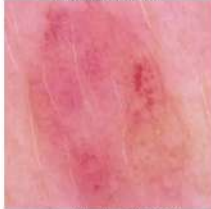

cosine dice l1\_ISIC\_2381102

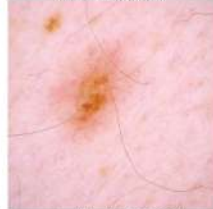

cosine dice l1\_ISIC\_844072

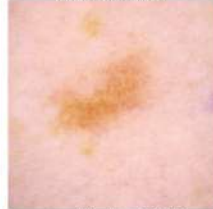

cosine euclidean dice l1\_ISIC\_0484163

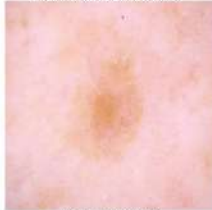

cosine euclidean dice l1\_ISIC\_7725628

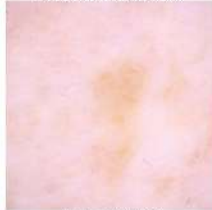

cosine euclidean dice l1\_ISIC\_0963211

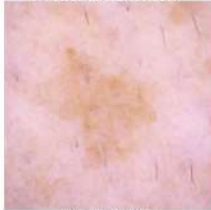

cosine euclidean dice l1\_ISIC\_8280776

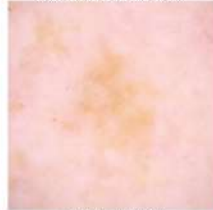

cosine euclidean dice l1\_ISIC\_5721613

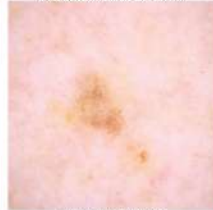

style dice l1\_ISIC\_2605118

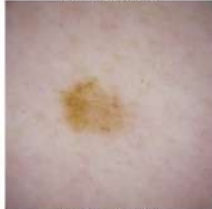

style dice l1\_ISIC\_0061959

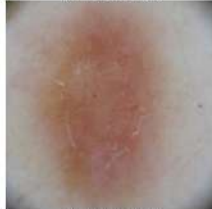

style dice l1\_ISIC\_6127167

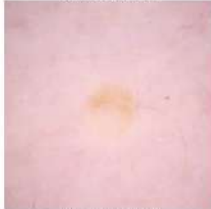

style dice l1\_ISIC\_1996538

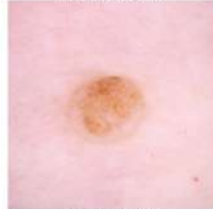

style dice l1\_ISIC\_0069867

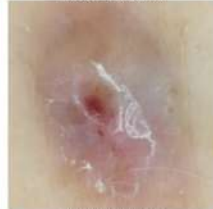

style eucl l1\_ISIC\_7053159

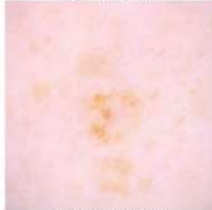

style eucl l1\_ISIC\_0484163

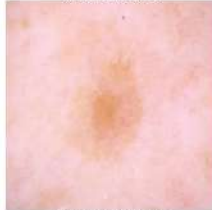

style eucl l1\_ISIC\_4452104

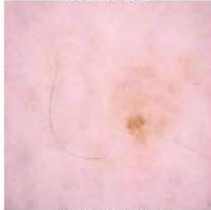

style eucl l1\_ISIC\_8843217

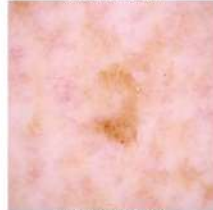

style eucl l1\_ISIC\_6296647

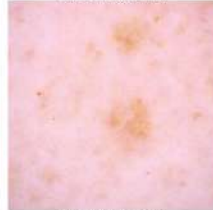

style cosine l1\_ISIC\_7053159

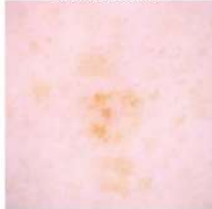

style cosine l1\_ISIC\_0484163

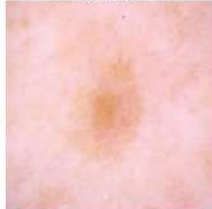

style cosine l1\_ISIC\_6347649

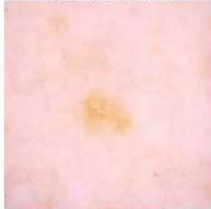

style cosine l1\_ISIC\_0422061

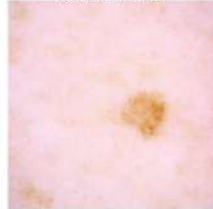

style cosine l1\_ISIC\_2346202

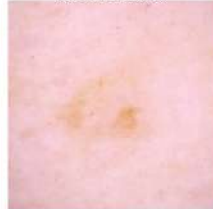

input image - ISIC\_0073333

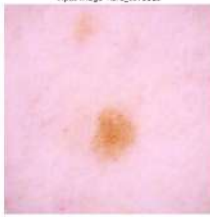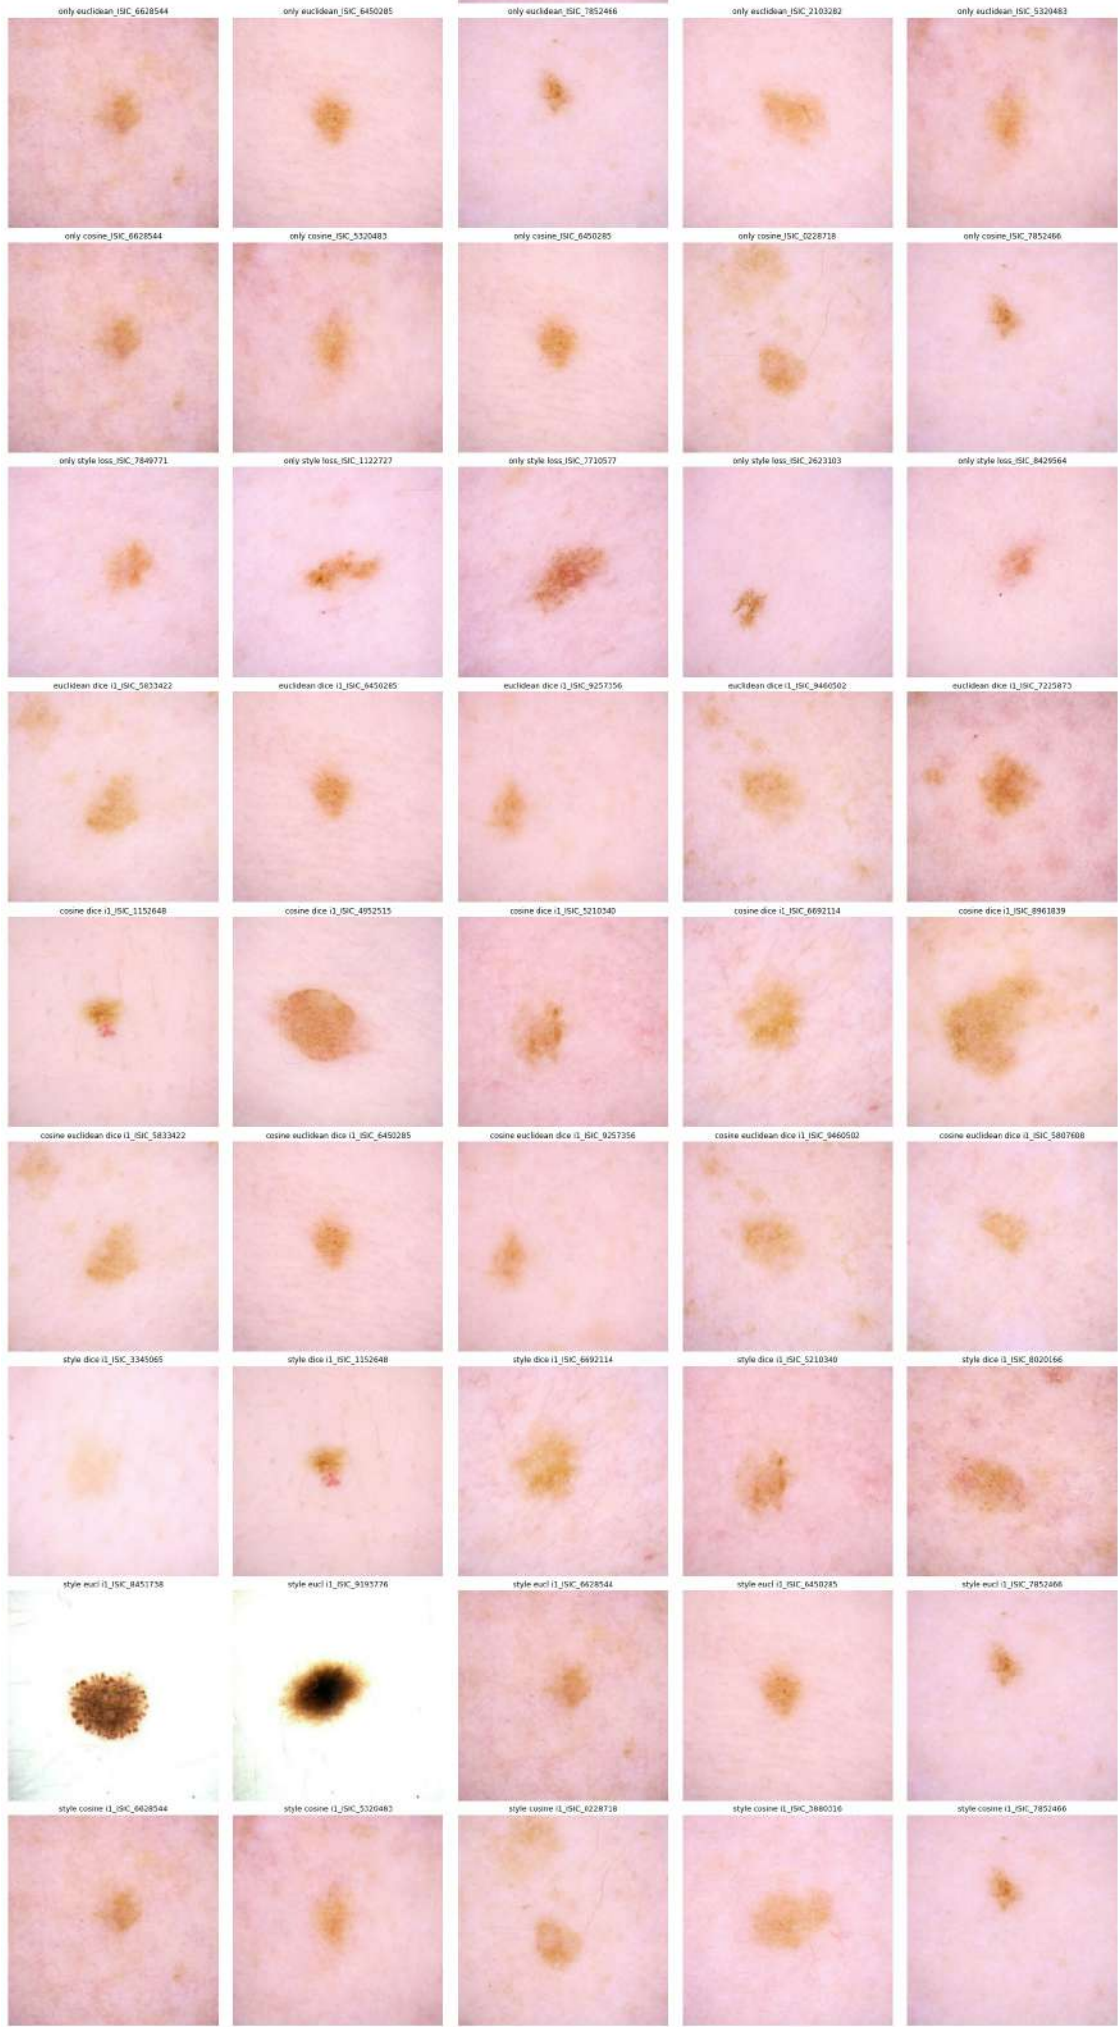

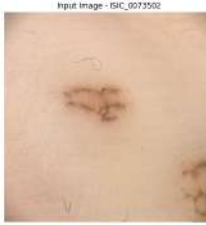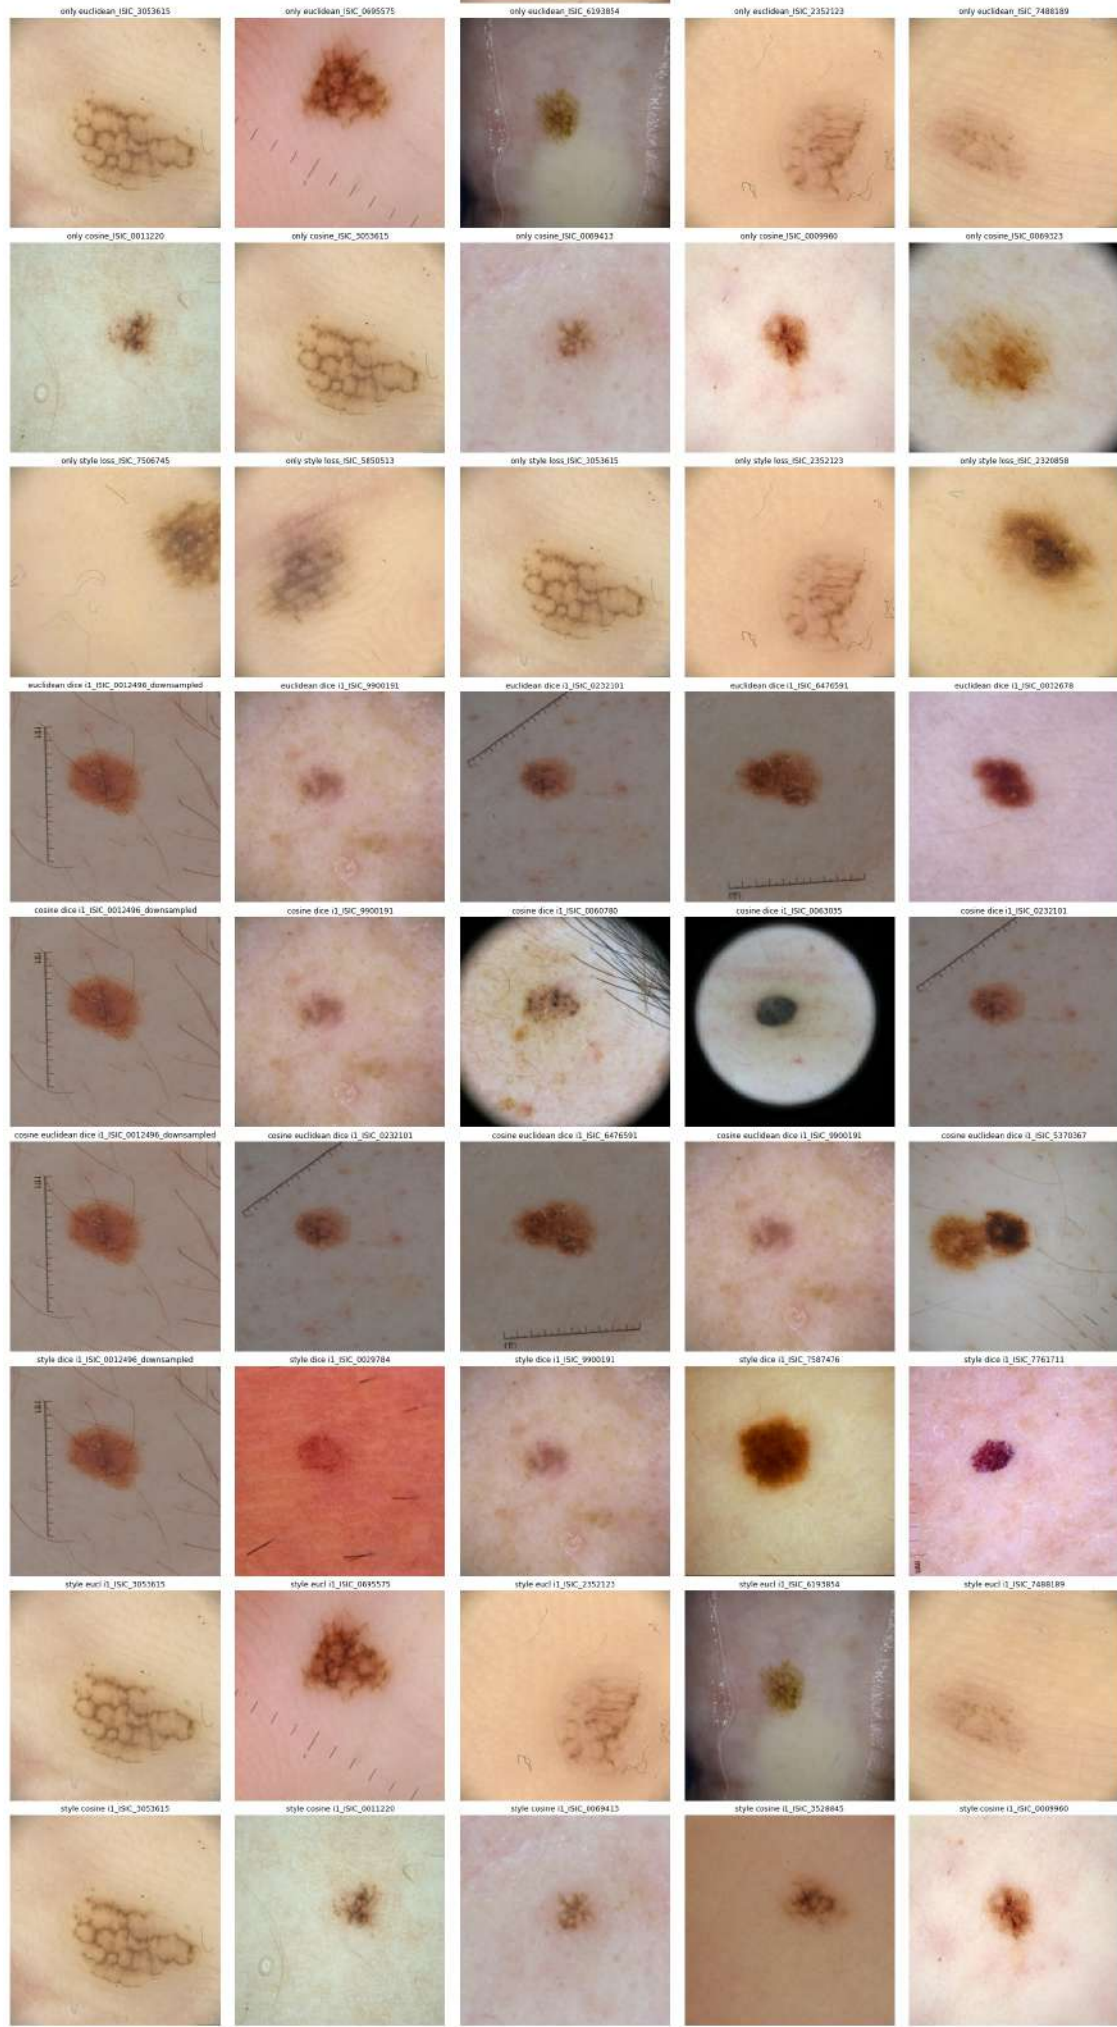

input image - ISIC\_0089350

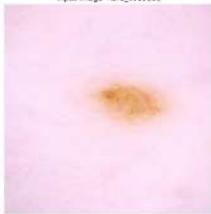

only euclidean\_ISIC\_5055747

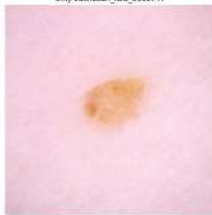

only euclidean\_ISIC\_7628560

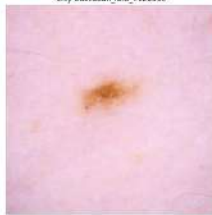

only euclidean\_ISIC\_2286273

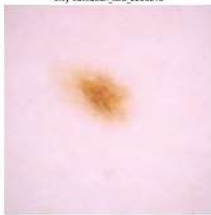

only euclidean\_ISIC\_0744870

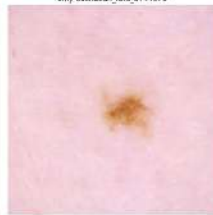

only euclidean\_ISIC\_3384884

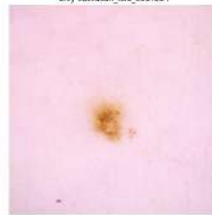

only cosine\_ISIC\_3384884

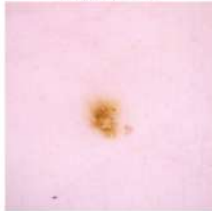

only cosine\_ISIC\_5005747

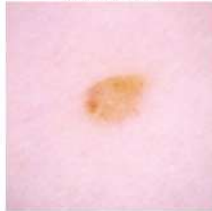

only cosine\_ISIC\_2286273

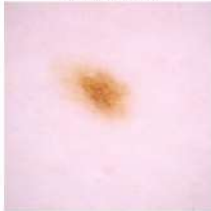

only cosine\_ISIC\_7628560

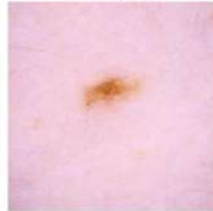

only cosine\_ISIC\_0561295

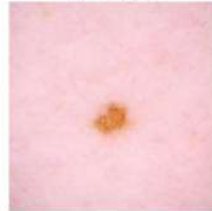

only style loss\_ISIC\_3106638

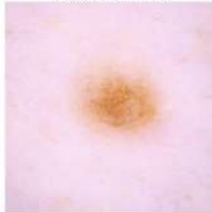

only style loss\_ISIC\_0608330

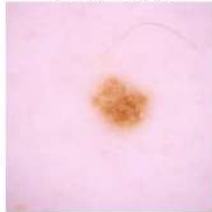

only style loss\_ISIC\_3106783

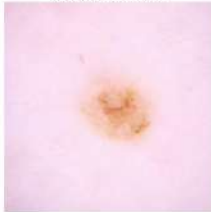

only style loss\_ISIC\_9318528

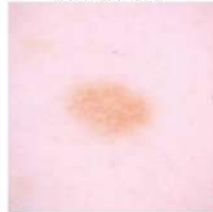

only style loss\_ISIC\_2286273

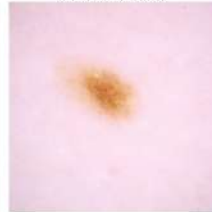

euclidean dice l1\_ISIC\_3587688

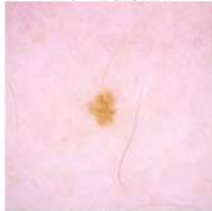

euclidean dice l1\_ISIC\_7051906

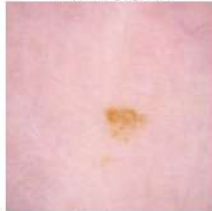

euclidean dice l1\_ISIC\_7766238

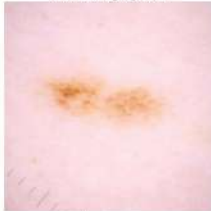

euclidean dice l1\_ISIC\_8700156

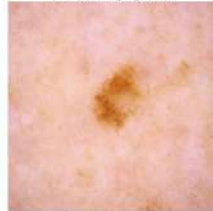

euclidean dice l1\_ISIC\_6042051

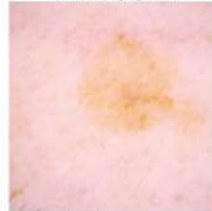

cosine dice l1\_ISIC\_1654007

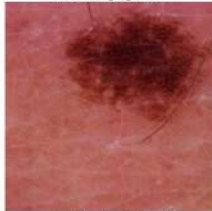

cosine dice l1\_ISIC\_9854060

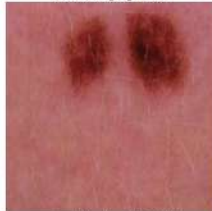

cosine dice l1\_ISIC\_0026943

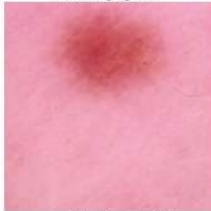

cosine dice l1\_ISIC\_3838110

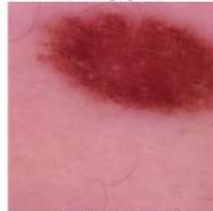

cosine dice l1\_ISIC\_6042051

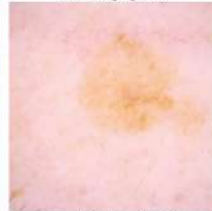

cosine euclidean dice l1\_ISIC\_3587688

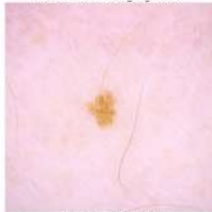

cosine euclidean dice l1\_ISIC\_7051906

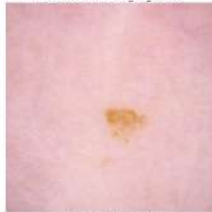

cosine euclidean dice l1\_ISIC\_7766238

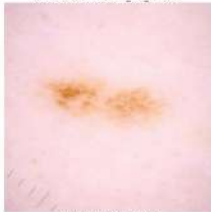

cosine euclidean dice l1\_ISIC\_8700156

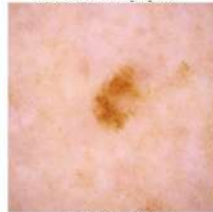

cosine euclidean dice l1\_ISIC\_4826018

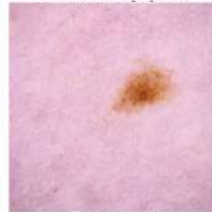

style dice l1\_ISIC\_1654007

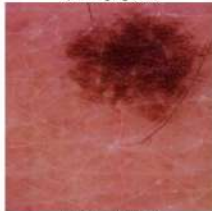

style dice l1\_ISIC\_9854060

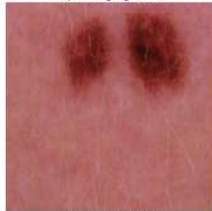

style dice l1\_ISIC\_5651246

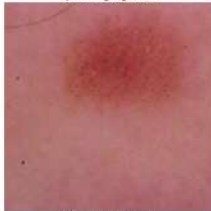

style dice l1\_ISIC\_3838110

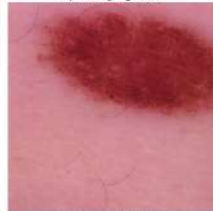

style dice l1\_ISIC\_3169421

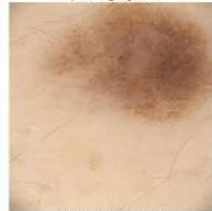

style eucl l1\_ISIC\_8451738

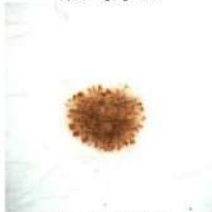

style eucl l1\_ISIC\_9193776

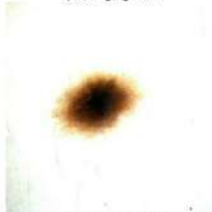

style eucl l1\_ISIC\_5005747

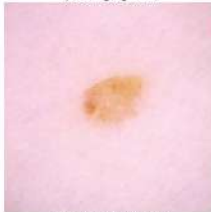

style eucl l1\_ISIC\_2286273

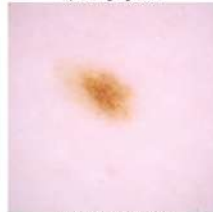

style eucl l1\_ISIC\_7628560

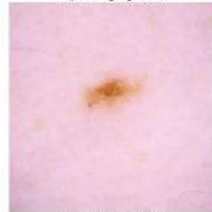

style cosine l1\_ISIC\_3384884

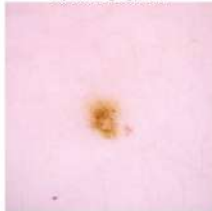

style cosine l1\_ISIC\_2286273

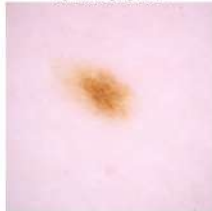

style cosine l1\_ISIC\_6444330

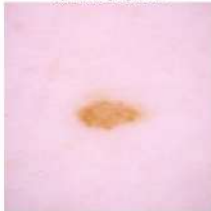

style cosine l1\_ISIC\_8218609

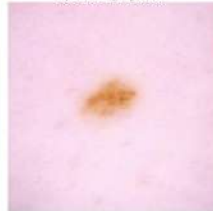

style cosine l1\_ISIC\_7628560

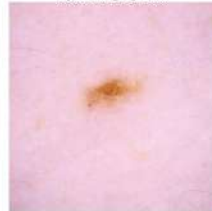



Input image - ISIC\_008836

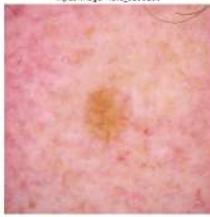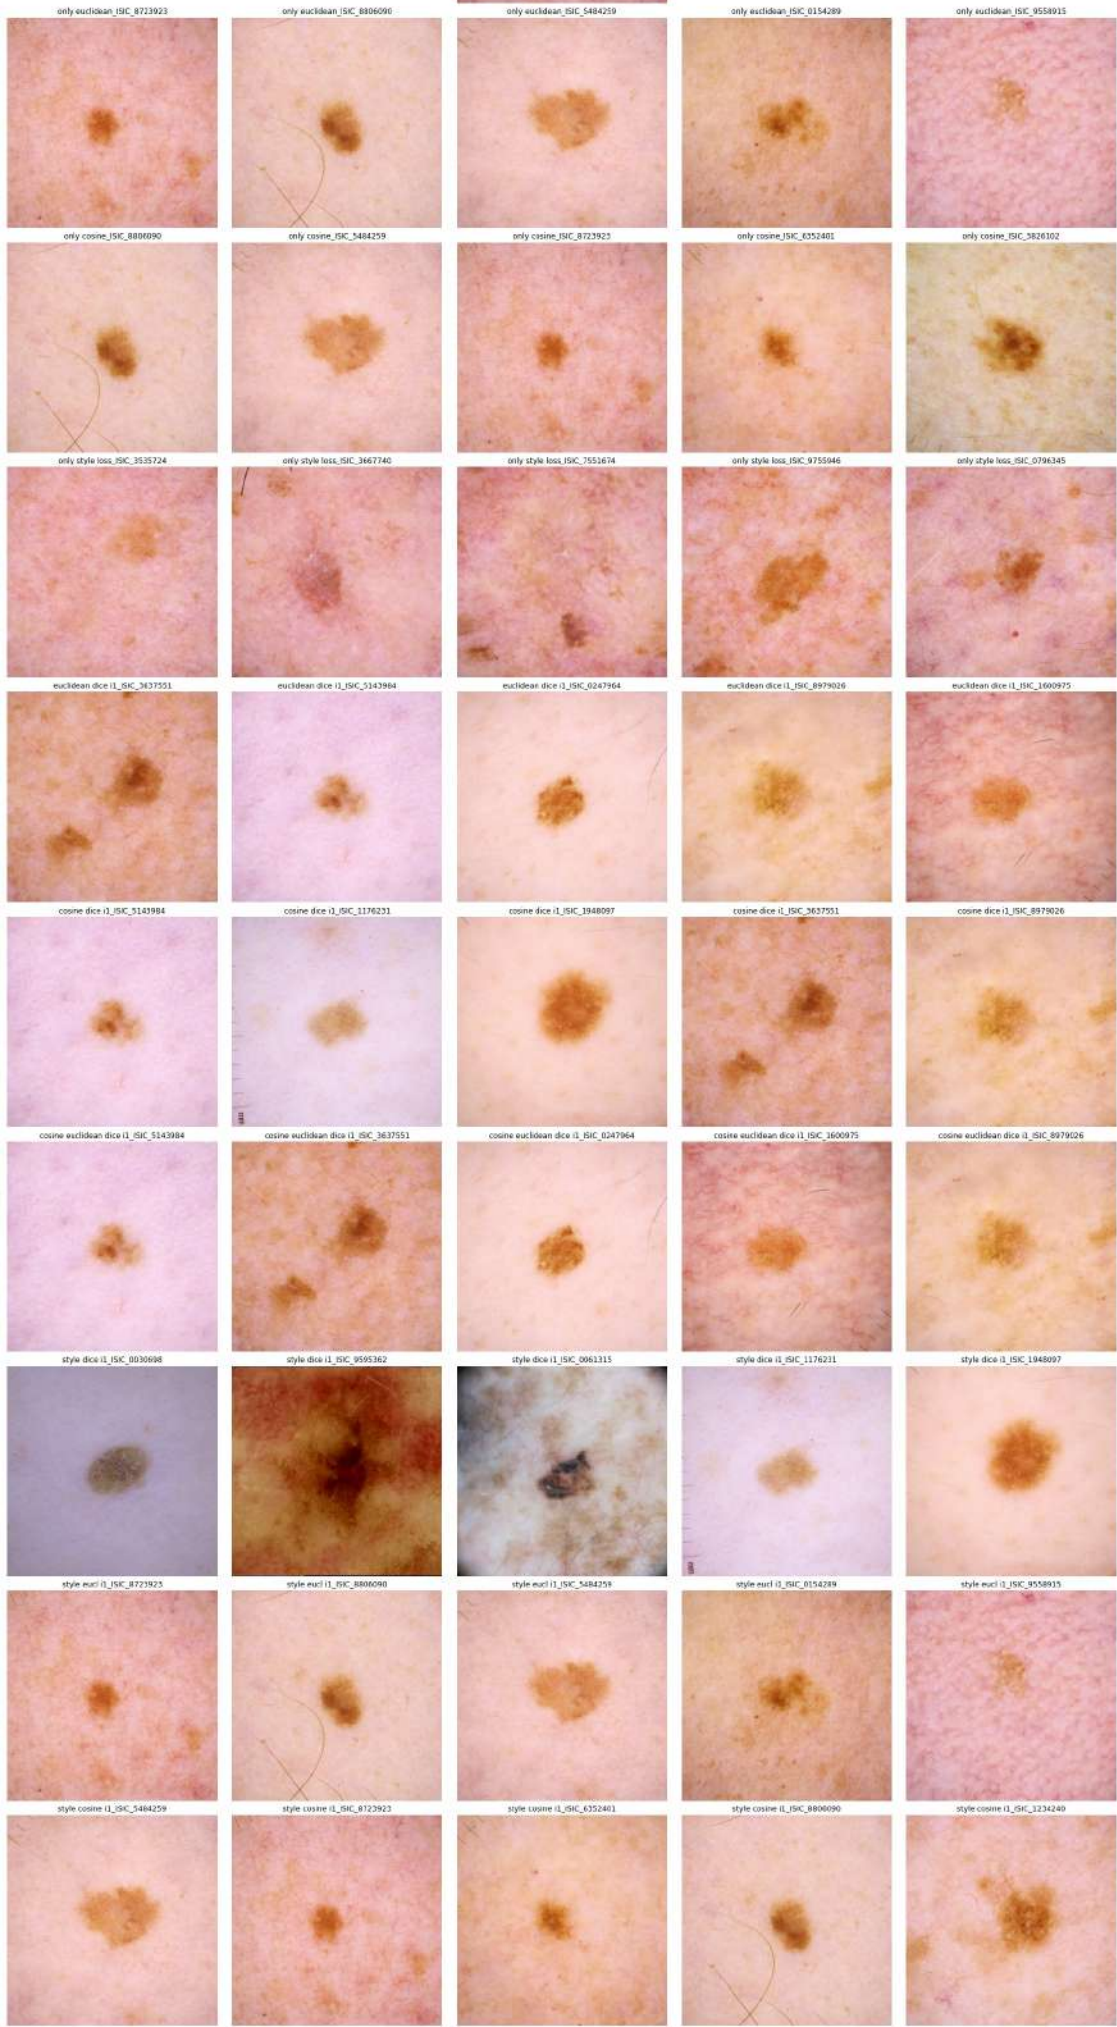

Input image - ISIC\_015798

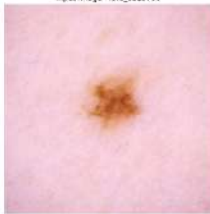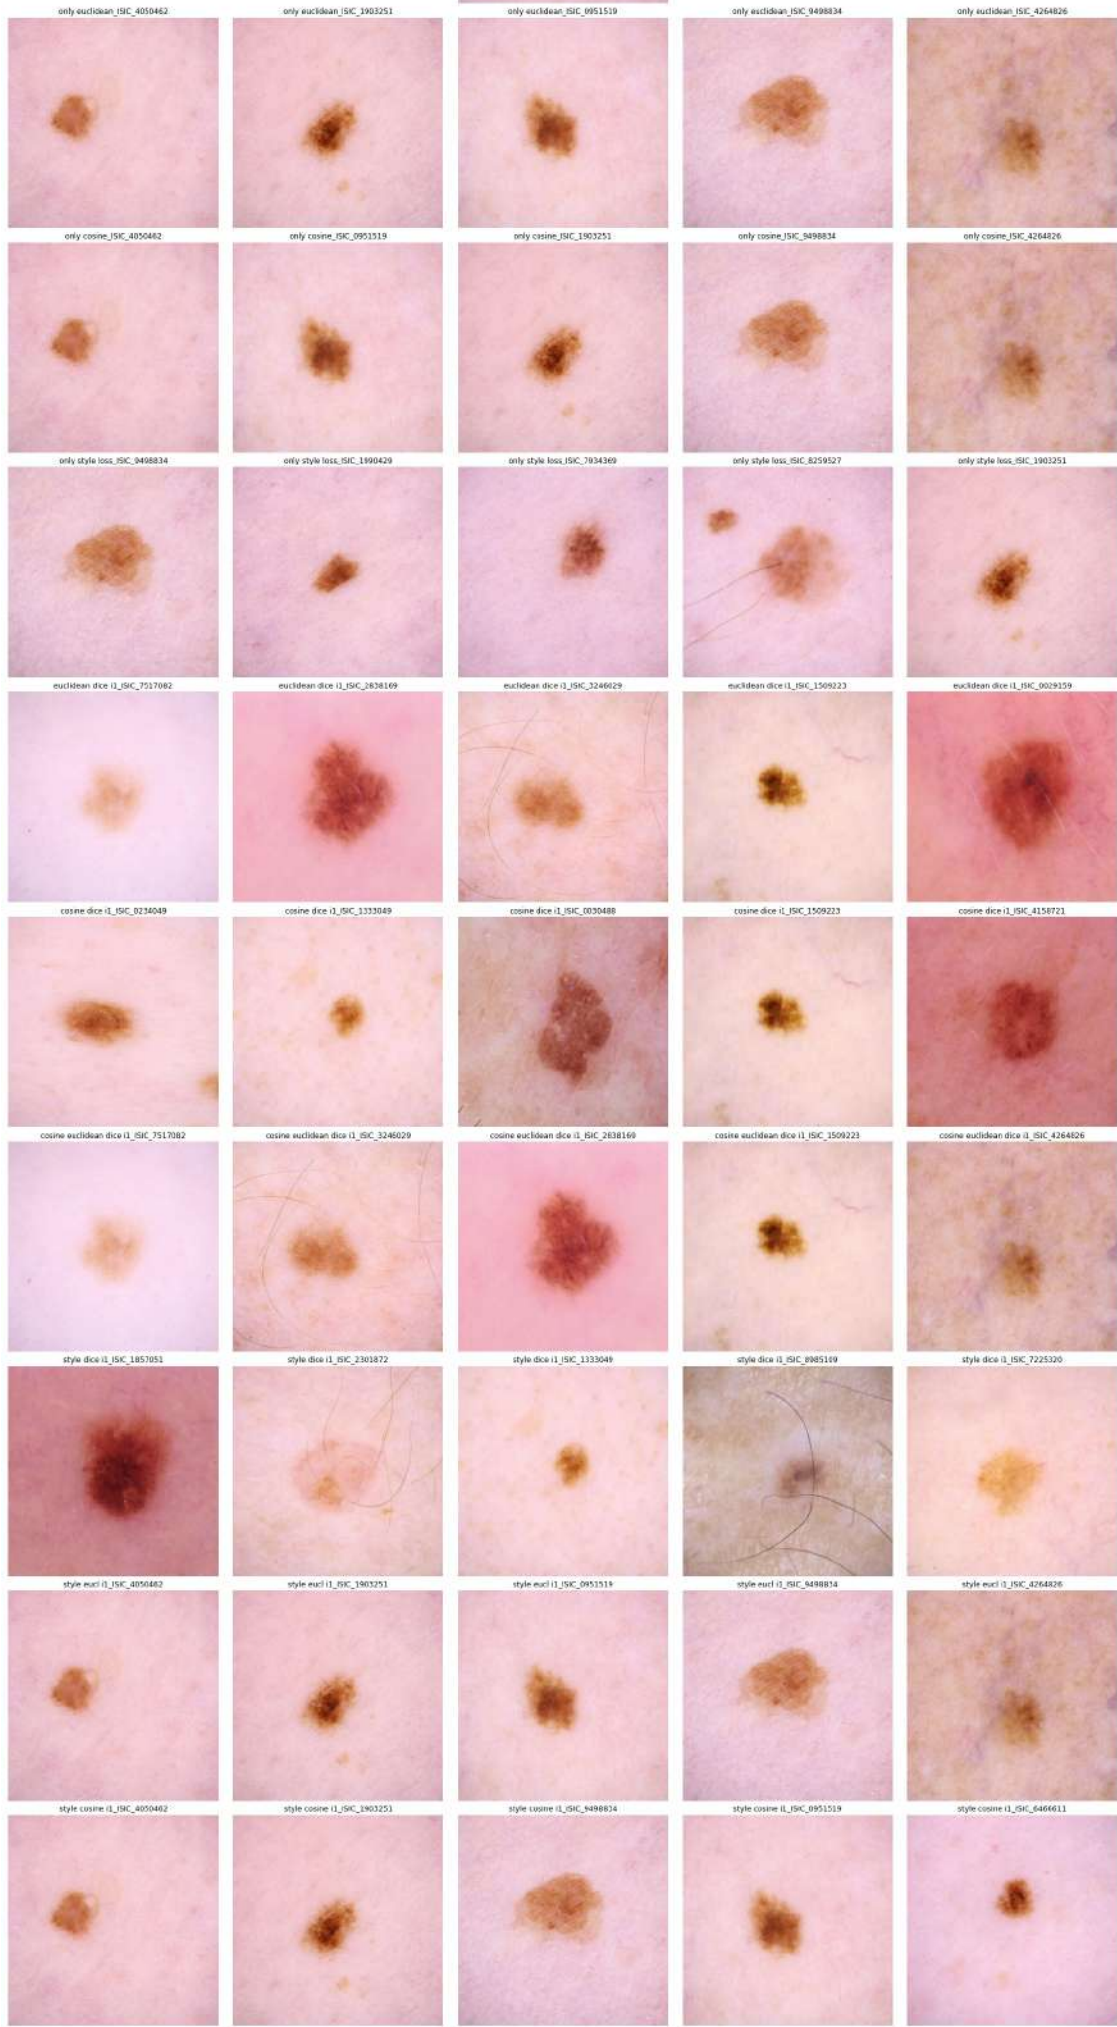

Input image - JSC\_0343109

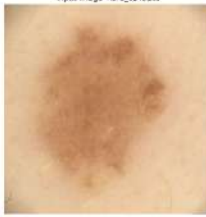

only euclidean\_JSC\_0352620

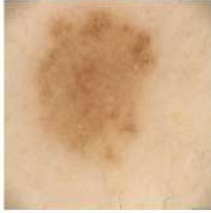

only euclidean\_JSC\_5969279

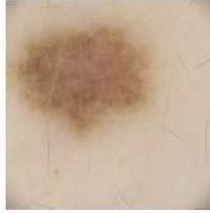

only euclidean\_JSC\_7590061

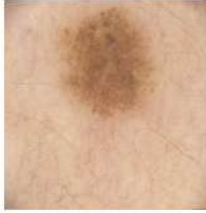

only euclidean\_JSC\_4771022

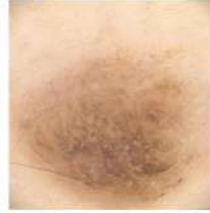

only euclidean\_JSC\_4111105

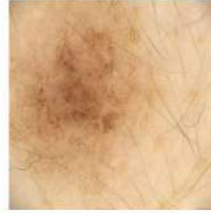

only cosine\_JSC\_0352620

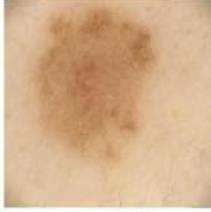

only cosine\_JSC\_5969279

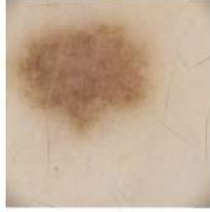

only cosine\_JSC\_7590061

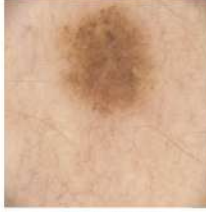

only cosine\_JSC\_4771022

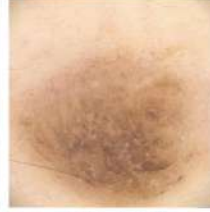

only cosine\_JSC\_4111105

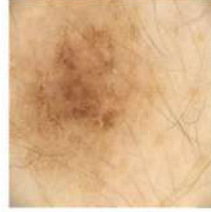

only style loss\_JSC\_0352620

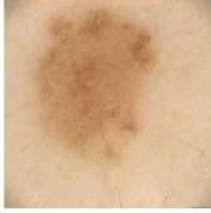

only style loss\_JSC\_2569931

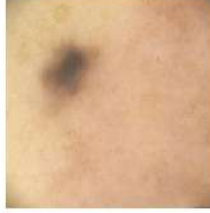

only style loss\_JSC\_8424990

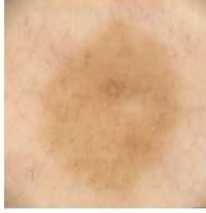

only style loss\_JSC\_1398977

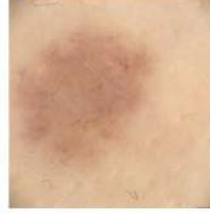

only style loss\_JSC\_6256102

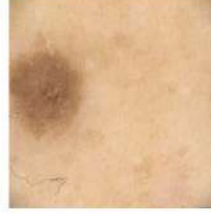

euclidean dice l1\_JSC\_4334767

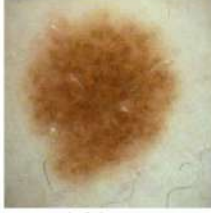

euclidean dice l2\_JSC\_5511088

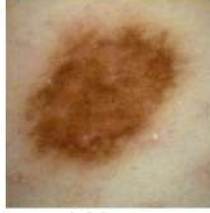

euclidean dice l1\_JSC\_8551617

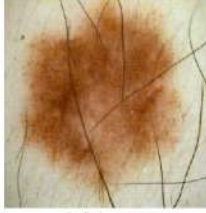

euclidean dice l1\_JSC\_0352620

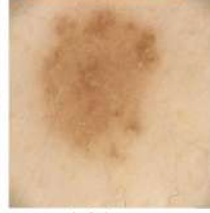

euclidean dice l1\_JSC\_2267335

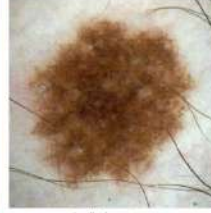

cosine dice l1\_JSC\_4334767

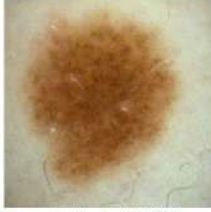

cosine dice l1\_JSC\_5511088

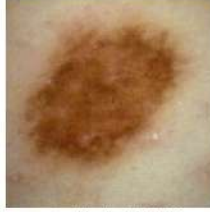

cosine dice l1\_JSC\_2267335

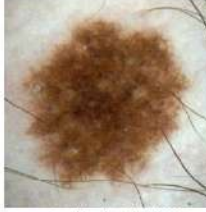

cosine dice l1\_JSC\_1692403

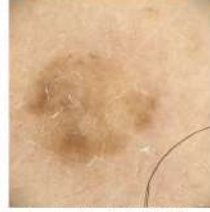

cosine dice l1\_JSC\_8551617

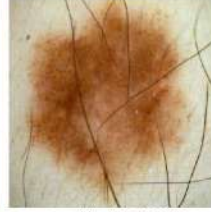

cosine euclidean dice l1\_JSC\_4334767

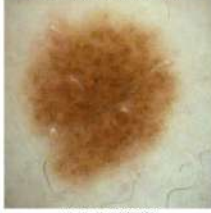

cosine euclidean dice l1\_JSC\_0352620

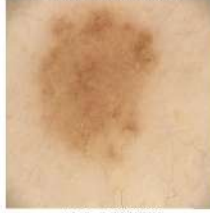

cosine euclidean dice l1\_JSC\_5511088

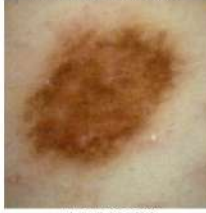

cosine euclidean dice l1\_JSC\_8551617

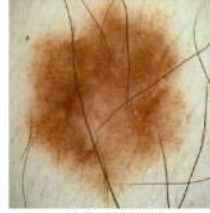

cosine euclidean dice l1\_JSC\_2267335

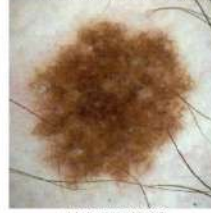

style dice l1\_JSC\_0191776

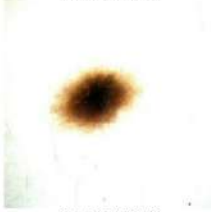

style dice l1\_JSC\_0025636

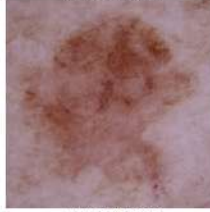

style dice l1\_JSC\_9436034

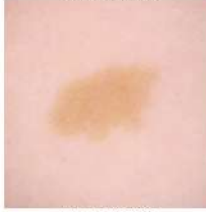

style dice l1\_JSC\_0027411

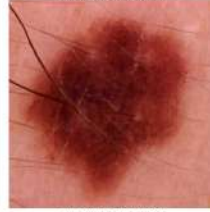

style dice l1\_JSC\_0029597

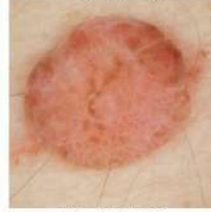

style eucl l1\_JSC\_0352620

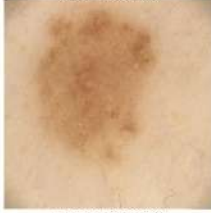

style eucl l1\_JSC\_5969279

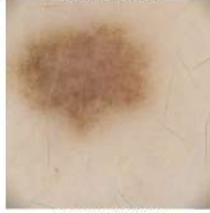

style eucl l1\_JSC\_7590061

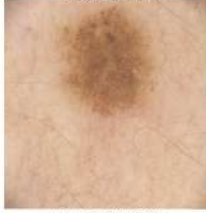

style eucl l1\_JSC\_4771022

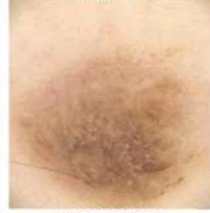

style eucl l1\_JSC\_4111105

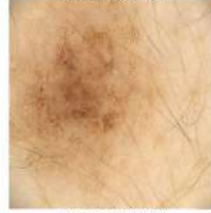

style cosine l1\_JSC\_0352620

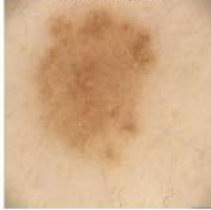

style cosine l1\_JSC\_5969279

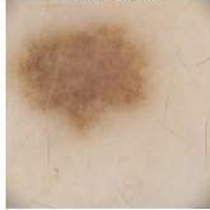

style cosine l1\_JSC\_4771022

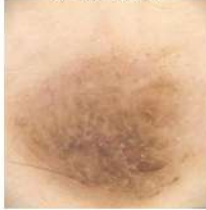

style cosine l1\_JSC\_7590061

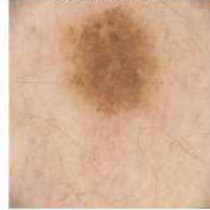

style cosine l1\_JSC\_4354483

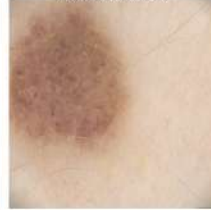



Input image - ISIC\_0168125

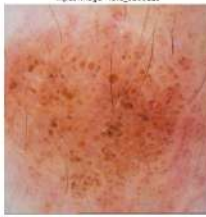

only euclidean\_ISIC\_1274220

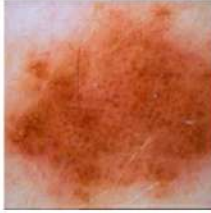

only euclidean\_ISIC\_0362853

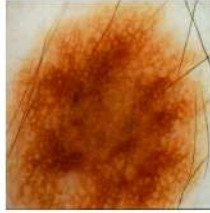

only euclidean\_ISIC\_5280331

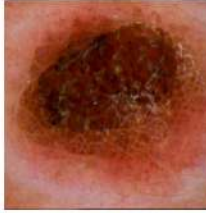

only euclidean\_ISIC\_6074613

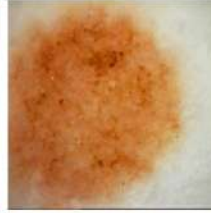

only euclidean\_ISIC\_9417604

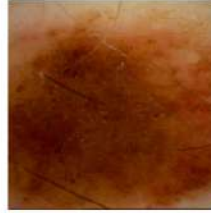

only cosine\_ISIC\_0362853

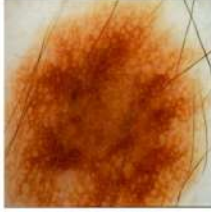

only cosine\_ISIC\_1274220

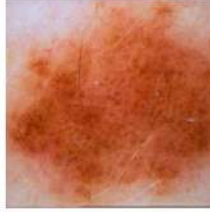

only cosine\_ISIC\_6074613

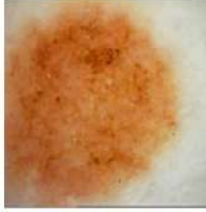

only cosine\_ISIC\_5280331

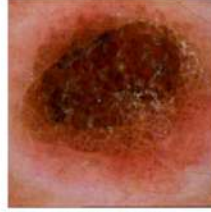

only cosine\_ISIC\_7032299

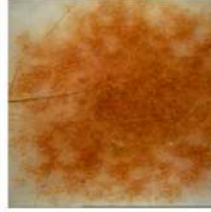

only style loss\_ISIC\_1274220

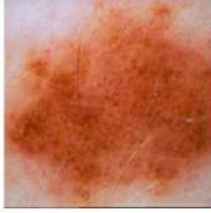

only style loss\_ISIC\_9861747

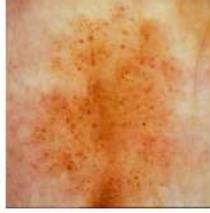

only style loss\_ISIC\_8242507

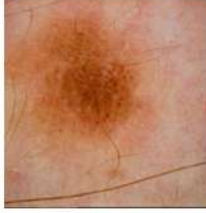

only style loss\_ISIC\_9127064

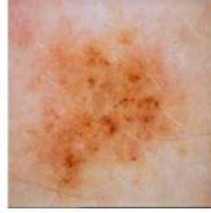

only style loss\_ISIC\_7151808

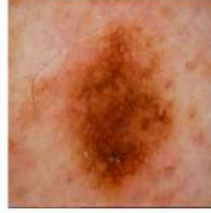

euclidean dice l1\_ISIC\_4905526

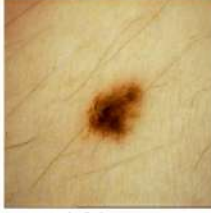

euclidean dice l1\_ISIC\_0342608

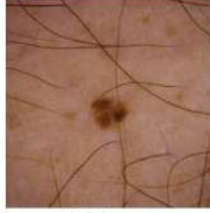

euclidean dice l1\_ISIC\_6352858

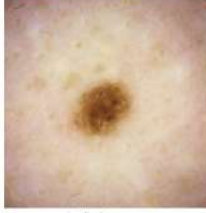

euclidean dice l1\_ISIC\_3382817

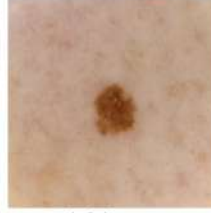

euclidean dice l1\_ISIC\_7810462

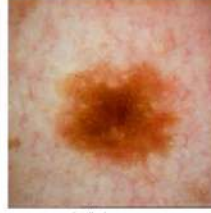

cosine dice l1\_ISIC\_0342608

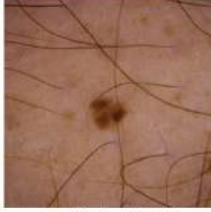

cosine dice l1\_ISIC\_4083460

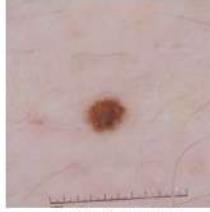

cosine dice l1\_ISIC\_5617771

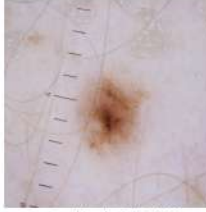

cosine dice l1\_ISIC\_4905526

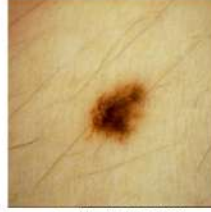

cosine dice l1\_ISIC\_4956965

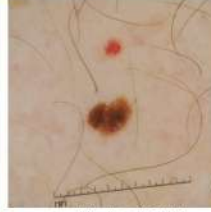

cosine euclidean dice l1\_ISIC\_4905526

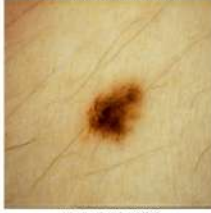

cosine euclidean dice l1\_ISIC\_6352858

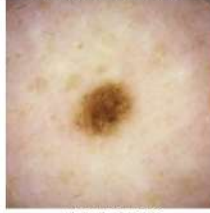

cosine euclidean dice l1\_ISIC\_3382817

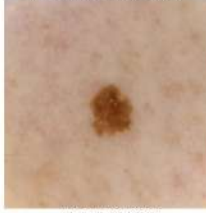

cosine euclidean dice l1\_ISIC\_0342608

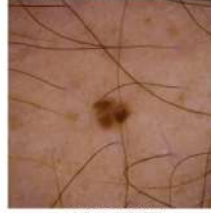

cosine euclidean dice l1\_ISIC\_7810462

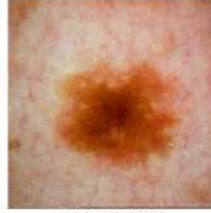

style dice l1\_ISIC\_4956965

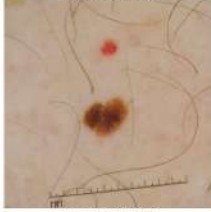

style dice l1\_ISIC\_0342608

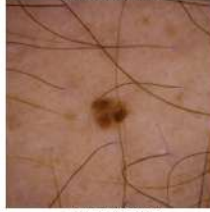

style dice l1\_ISIC\_4083460

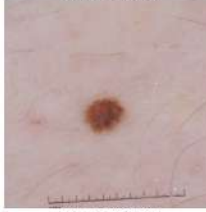

style dice l1\_ISIC\_5617771

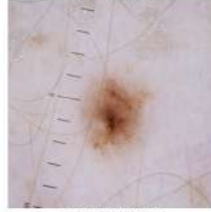

style dice l1\_ISIC\_1665254

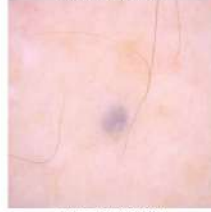

style eucl l1\_ISIC\_1274220

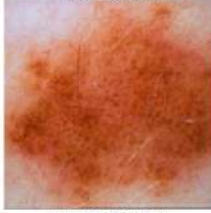

style eucl l1\_ISIC\_5280331

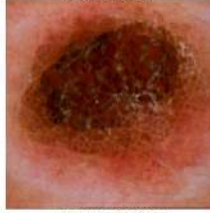

style eucl l1\_ISIC\_0362853

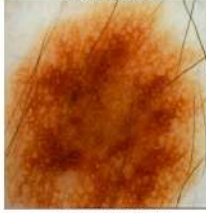

style eucl l1\_ISIC\_6074613

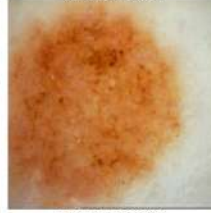

style eucl l1\_ISIC\_9417604

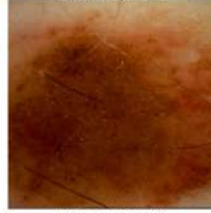

style cosine l1\_ISIC\_1274220

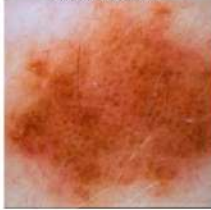

style cosine l1\_ISIC\_5280331

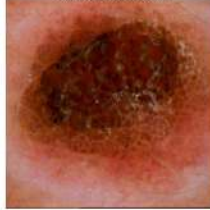

style cosine l1\_ISIC\_0362853

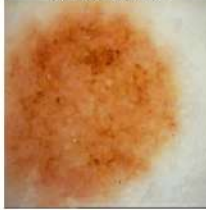

style cosine l1\_ISIC\_6074613

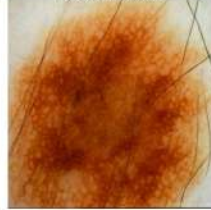

style cosine l1\_ISIC\_7032299

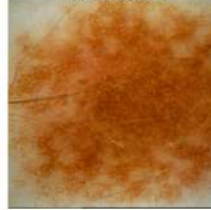

Input image - ISIC\_0171865

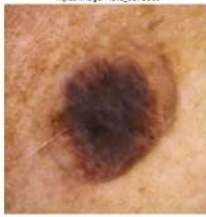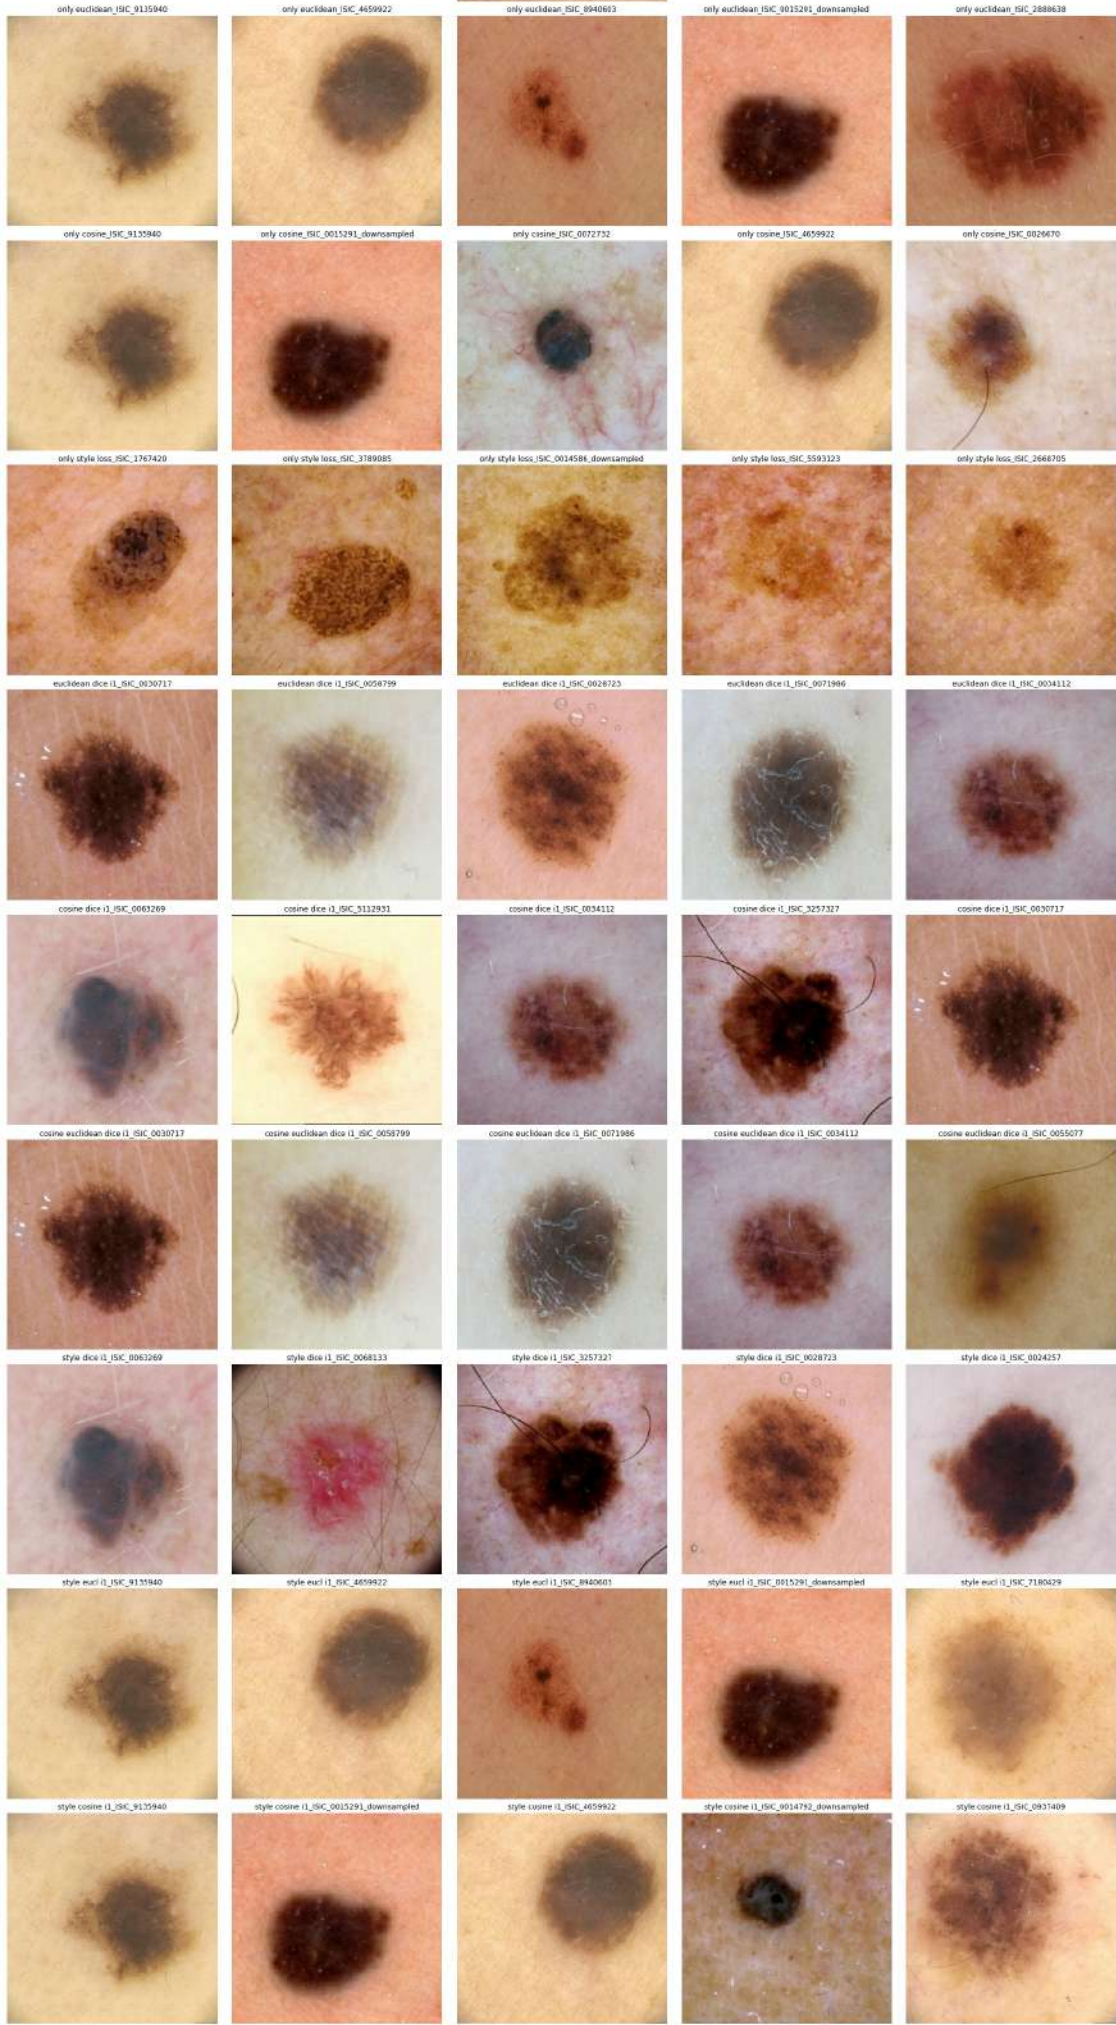

input image - ISIC\_0376152

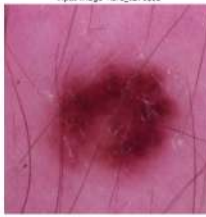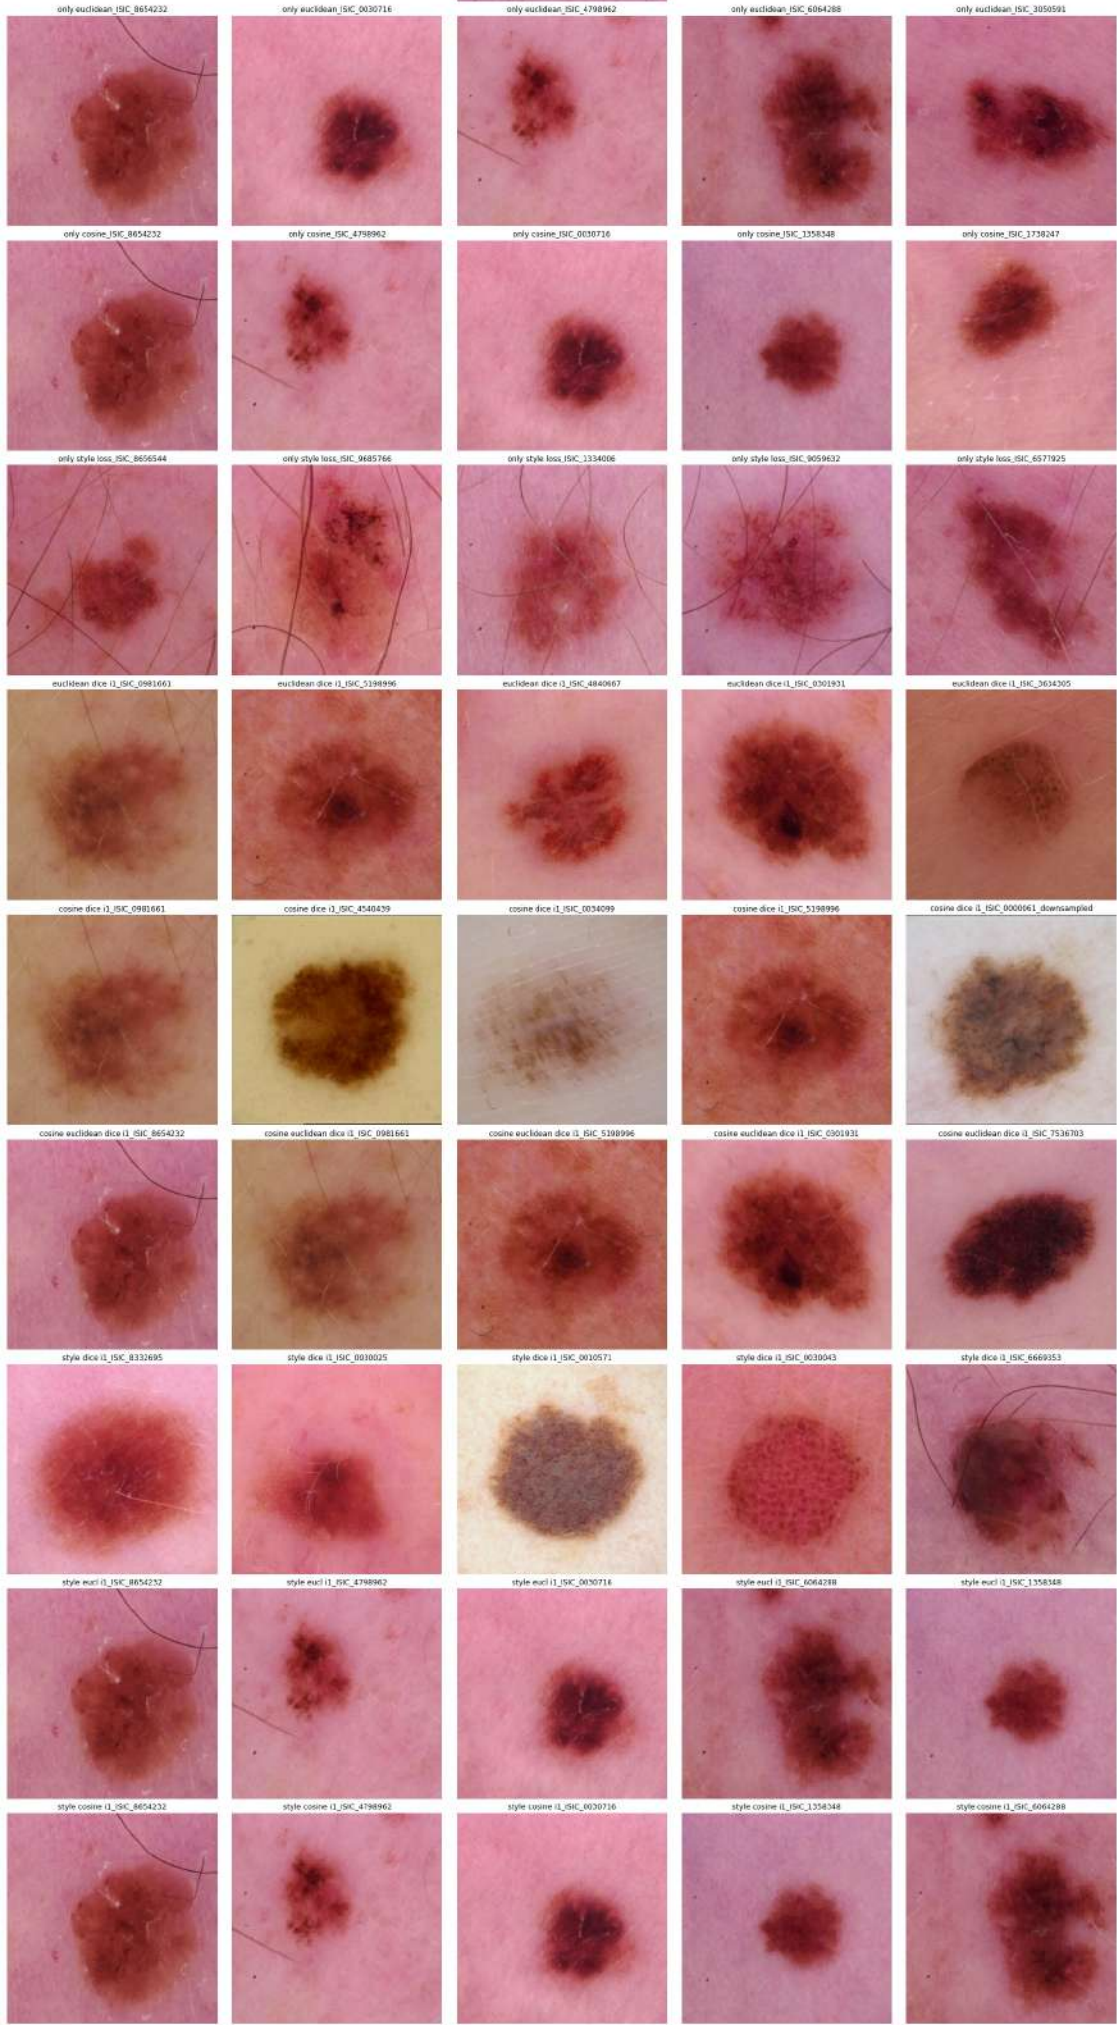

input image - ISIC\_0383449

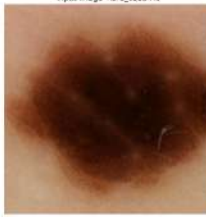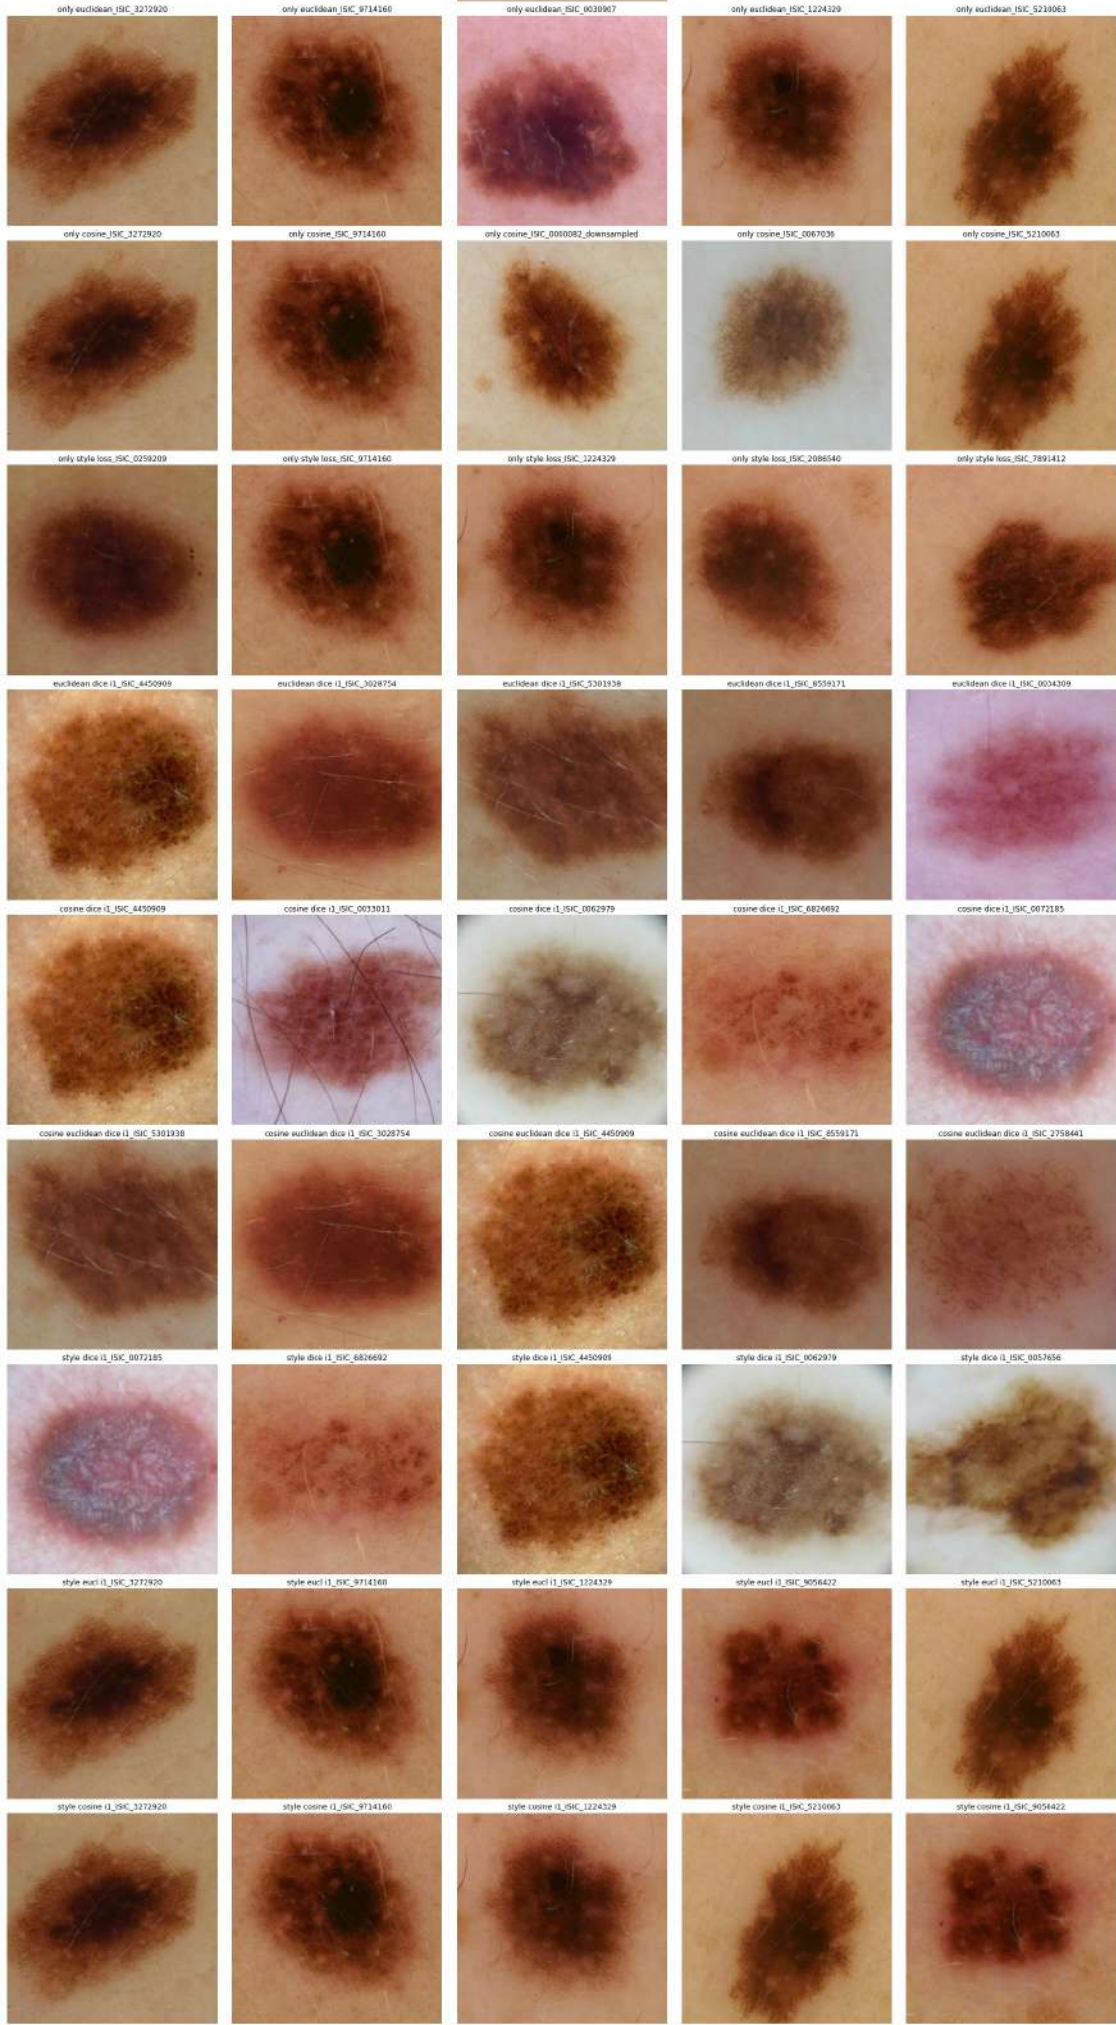

Input image - ISIC\_0183771

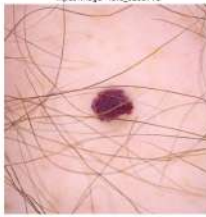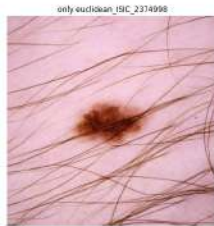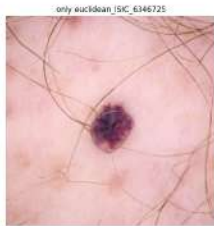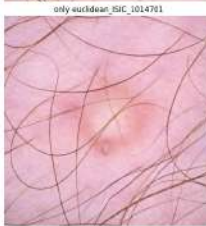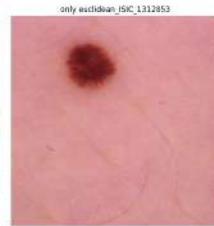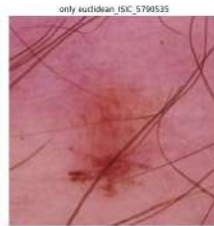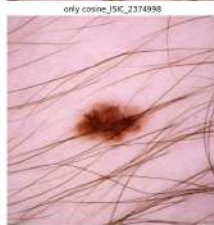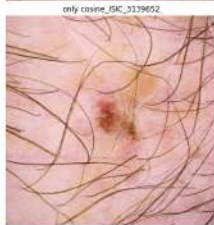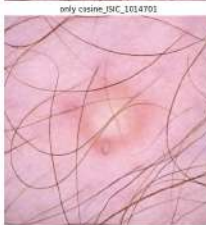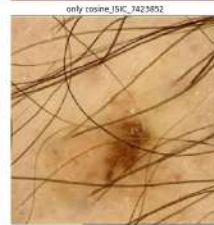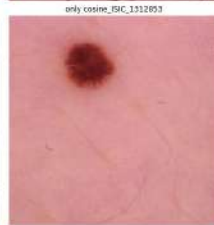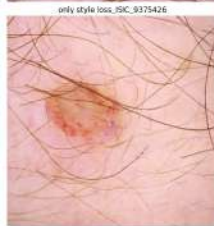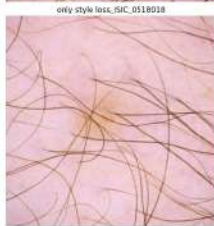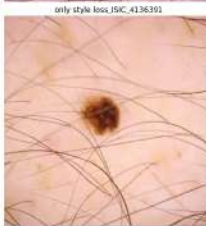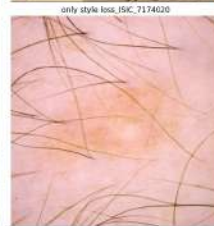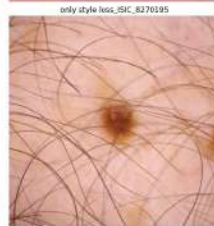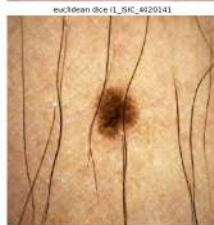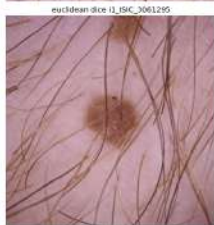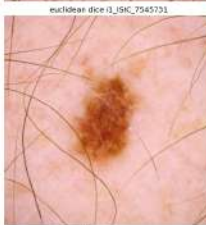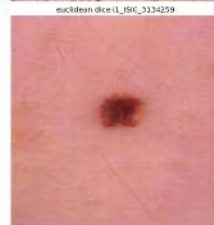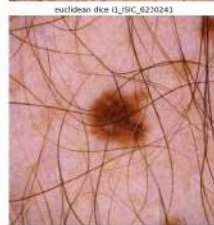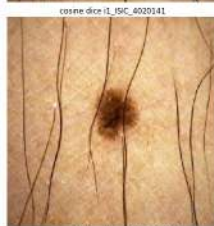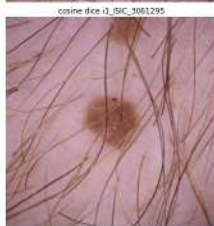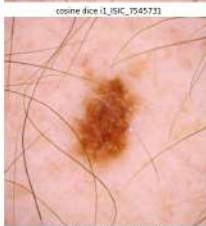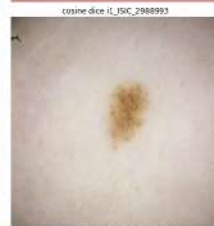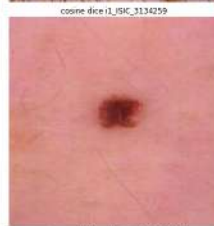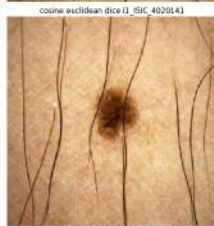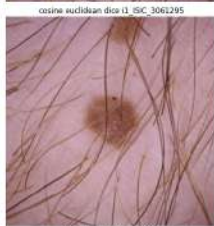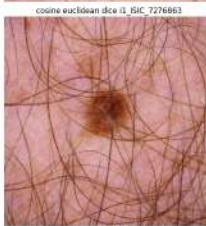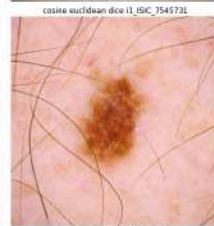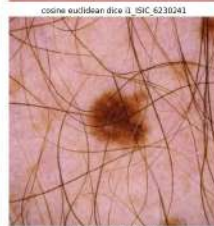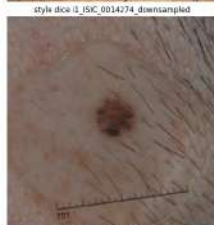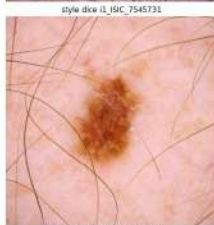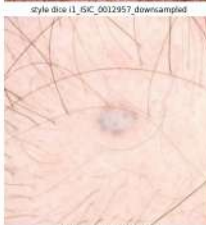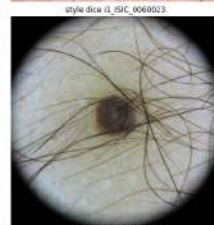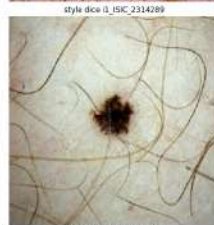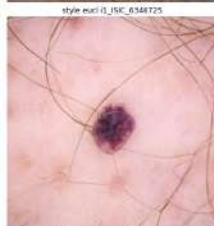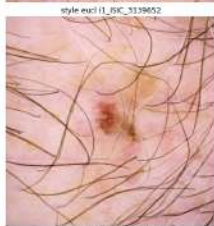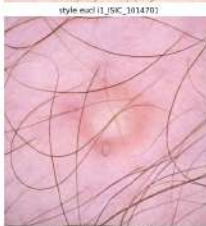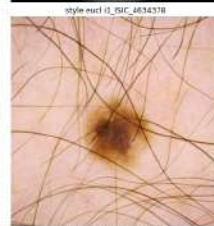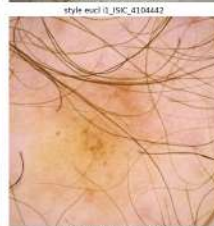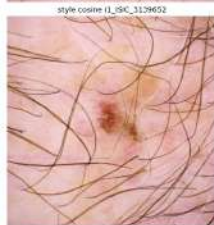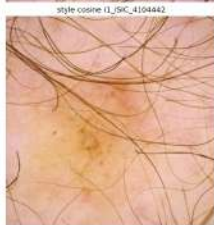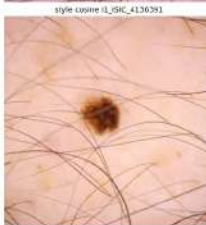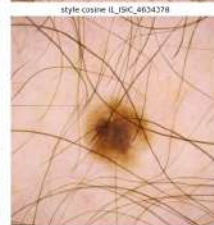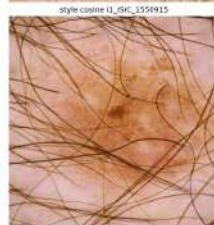

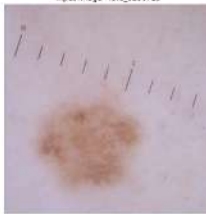

only euclidean\_ISIC\_8119203

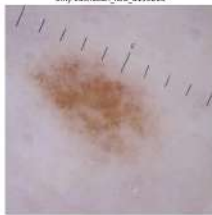

only euclidean\_ISIC\_3322378

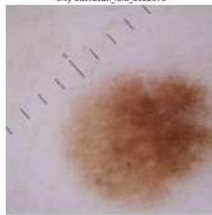

only euclidean\_ISIC\_8474432

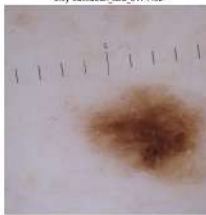

only euclidean\_ISIC\_9806131

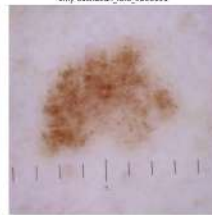

only euclidean\_ISIC\_6636720

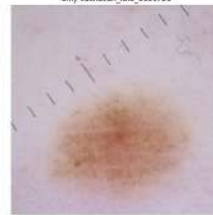

only cosine\_ISIC\_8119203

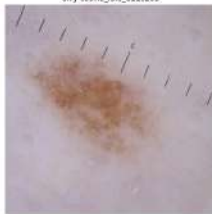

only cosine\_ISIC\_3322378

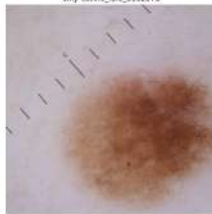

only cosine\_ISIC\_9806131

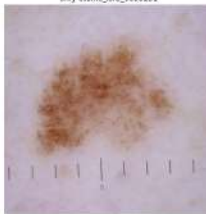

only cosine\_ISIC\_5687776

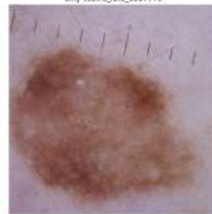

only cosine\_ISIC\_8474432

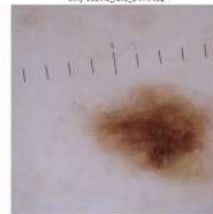

only style loss\_ISIC\_8119203

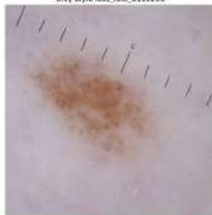

only style loss\_ISIC\_1603834

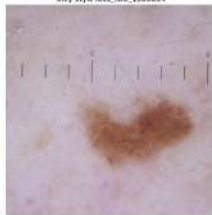

only style loss\_ISIC\_3503498

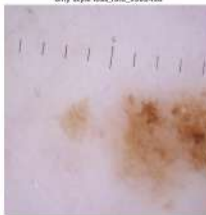

only style loss\_ISIC\_3066195

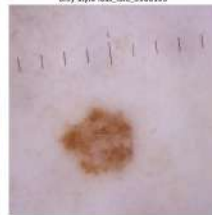

only style loss\_ISIC\_4971739

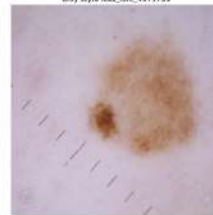

euclidean dice l1\_ISIC\_0000478

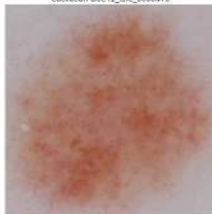

euclidean dice l1\_ISIC\_0031528

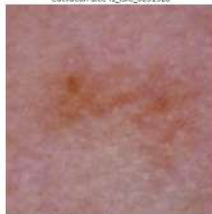

euclidean dice l1\_ISIC\_0027178

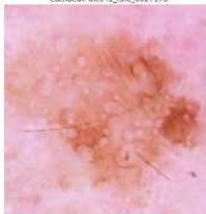

euclidean dice l1\_ISIC\_0057040

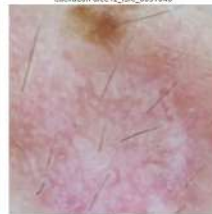

euclidean dice l1\_ISIC\_0026614

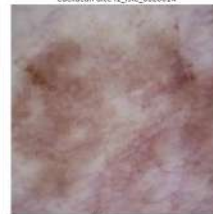

cosine dice l1\_ISIC\_0026614

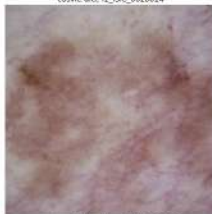

cosine dice l1\_ISIC\_0034142

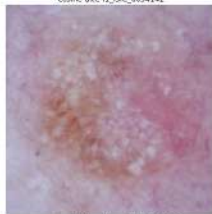

cosine dice l1\_ISIC\_0071005

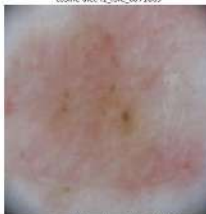

cosine dice l1\_ISIC\_0063948

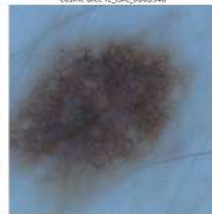

cosine dice l1\_ISIC\_0031528

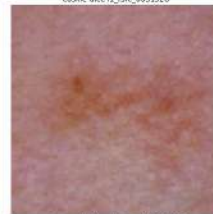

cosine euclidean dice l1\_ISIC\_0000478

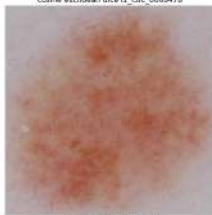

cosine euclidean dice l1\_ISIC\_0031528

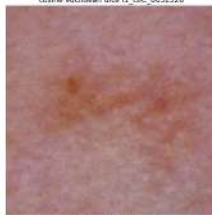

cosine euclidean dice l1\_ISIC\_0027178

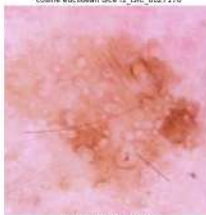

cosine euclidean dice l1\_ISIC\_0057040

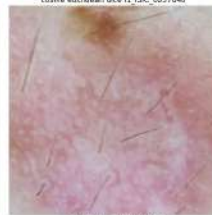

cosine euclidean dice l1\_ISIC\_0028755

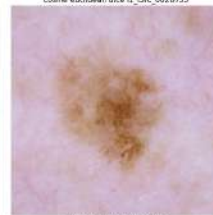

style dice l1\_ISIC\_0053511

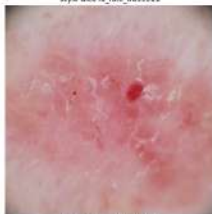

style dice l1\_ISIC\_0071147

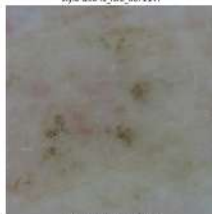

style dice l1\_ISIC\_0026614

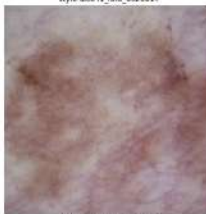

style dice l1\_ISIC\_0065584

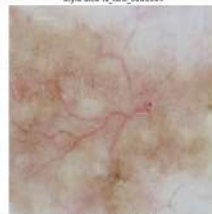

style dice l1\_ISIC\_0071005

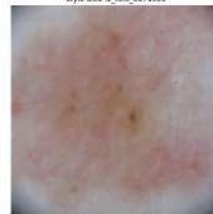

style euc1 l1\_ISIC\_8119203

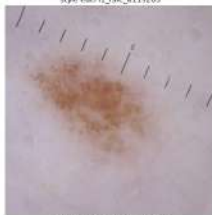

style euc1 l1\_ISIC\_3322378

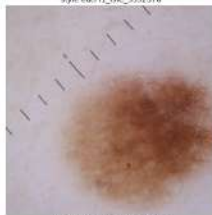

style euc1 l1\_ISIC\_9806131

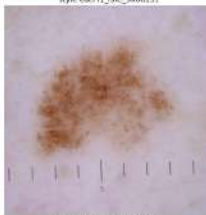

style euc1 l1\_ISIC\_8474432

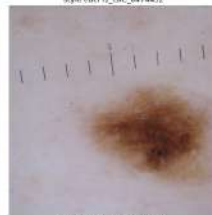

style euc1 l1\_ISIC\_6636720

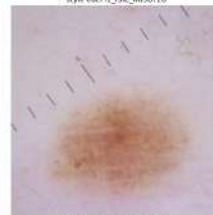

style cosine l1\_ISIC\_8119203

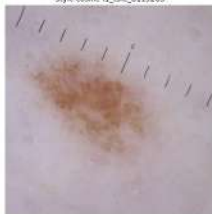

style cosine l1\_ISIC\_3322378

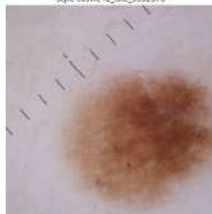

style cosine l1\_ISIC\_9806131

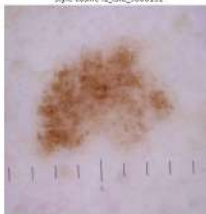

style cosine l1\_ISIC\_8474432

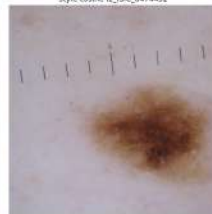

style cosine l1\_ISIC\_6636720

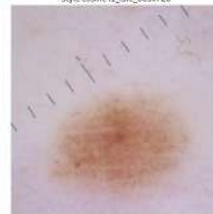

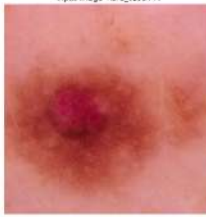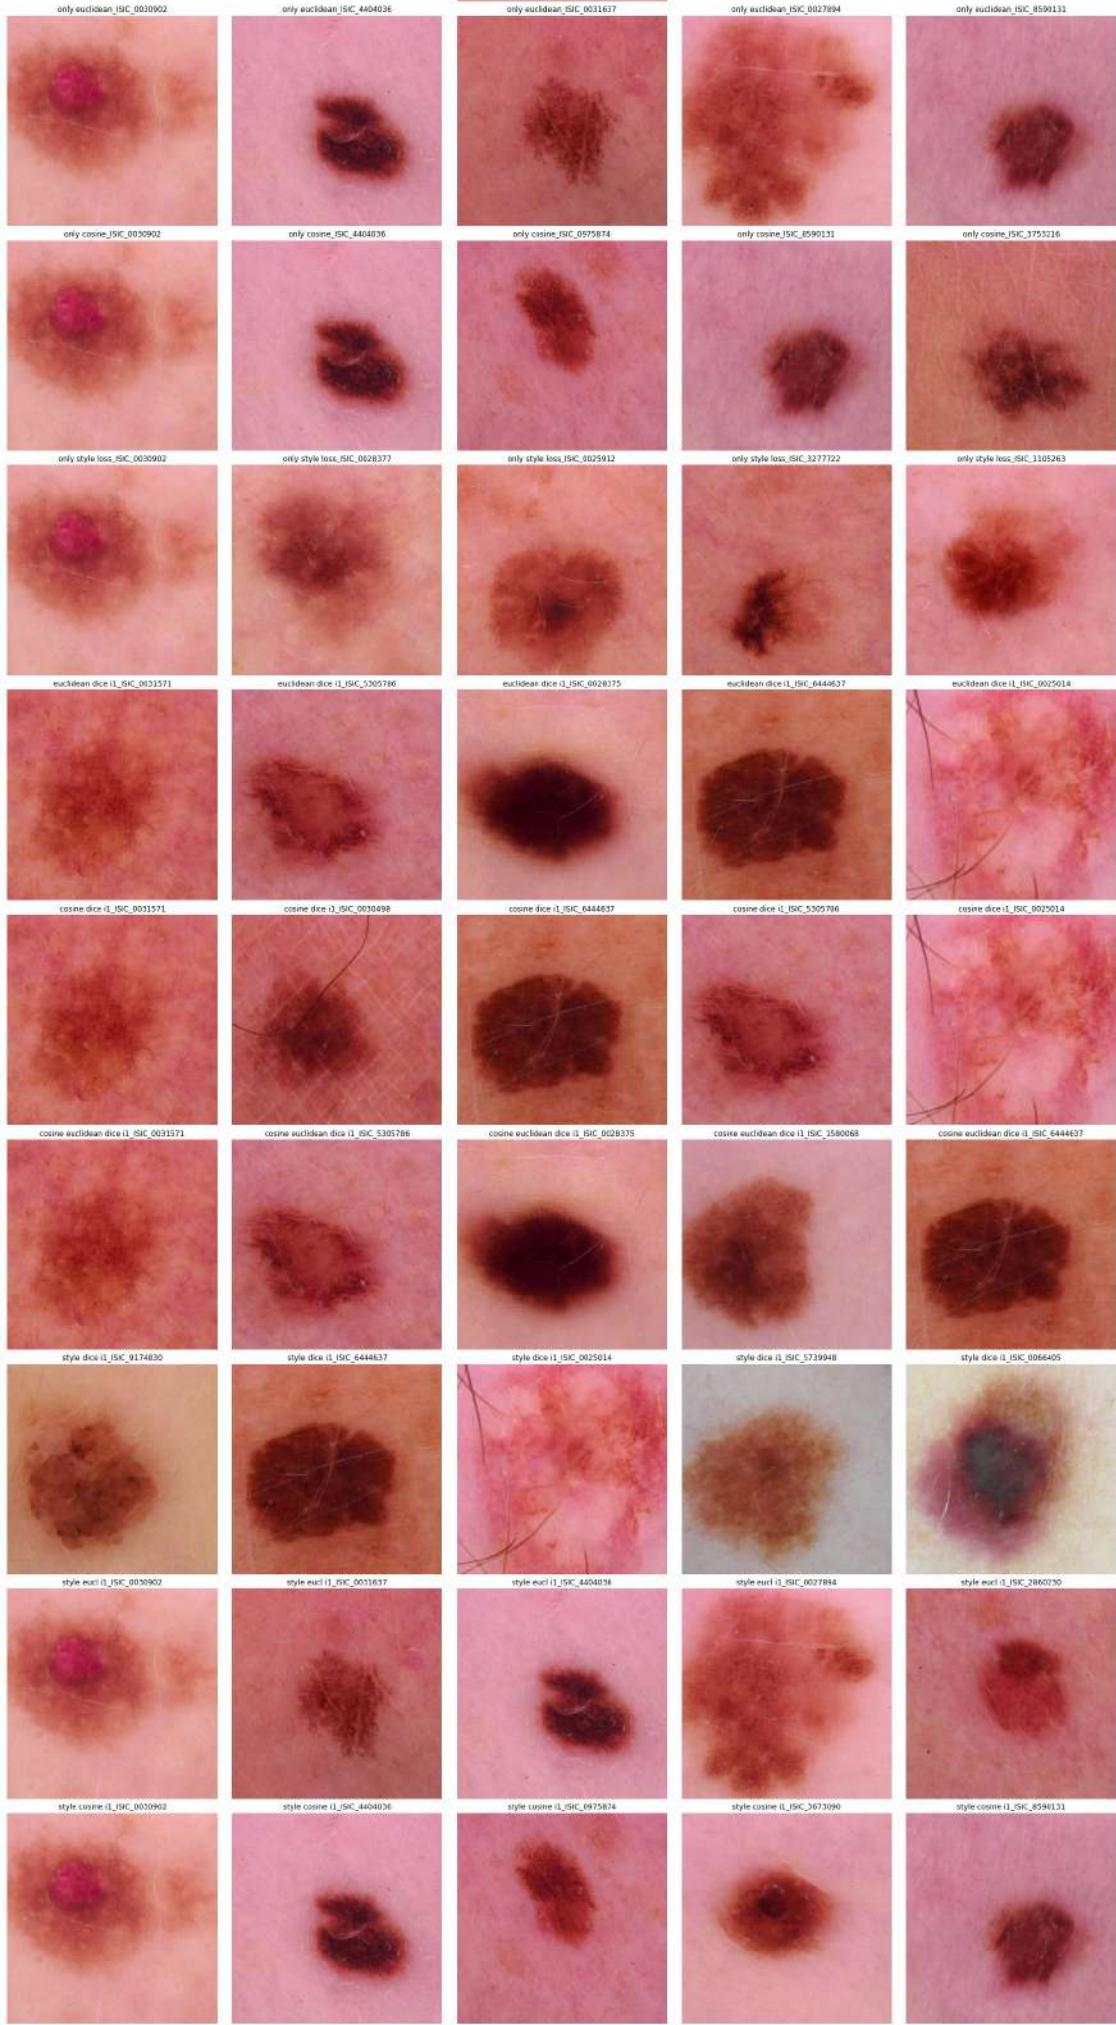

Input image - ISIC\_0196807

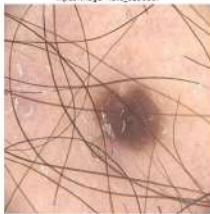

only euclidean\_ISIC\_4431911

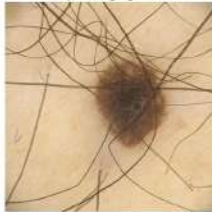

only euclidean\_ISIC\_2105735

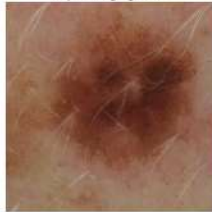

only euclidean\_ISIC\_7858885

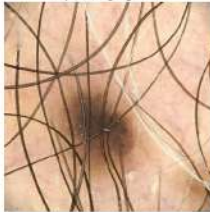

only euclidean\_ISIC\_8655808

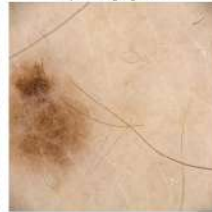

only euclidean\_ISIC\_0012549\_downsampled

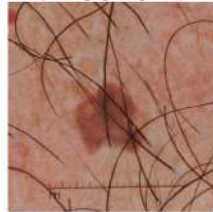

only cosine\_ISIC\_4431911

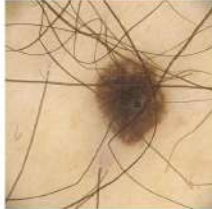

only cosine\_ISIC\_0000380\_downsampled

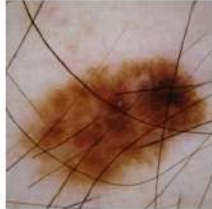

only cosine\_ISIC\_0053931

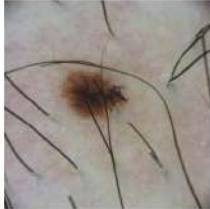

only cosine\_ISIC\_0012548\_downsampled

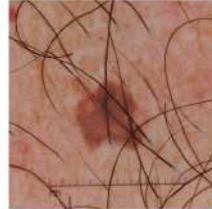

only cosine\_ISIC\_2105735

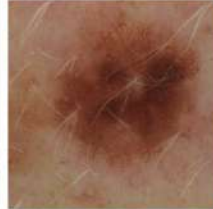

only style loss\_ISIC\_4564430

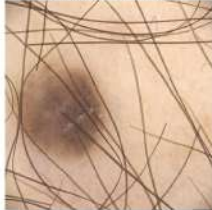

only style loss\_ISIC\_0284441

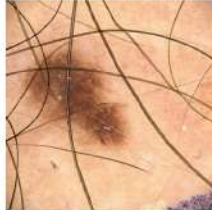

only style loss\_ISIC\_0948167

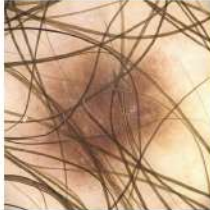

only style loss\_ISIC\_1497685

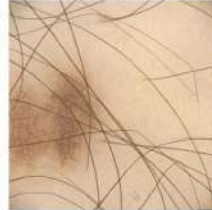

only style loss\_ISIC\_5311159

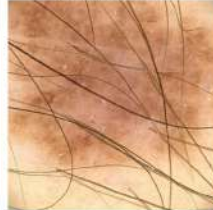

euclidean dice l1\_ISIC\_0033982

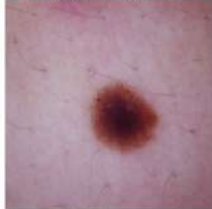

euclidean dice l1\_ISIC\_2914669

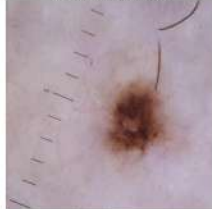

euclidean dice l1\_ISIC\_3372750

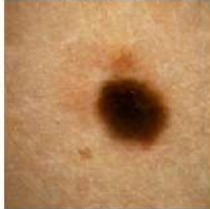

euclidean dice l1\_ISIC\_6609484

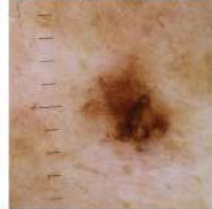

euclidean dice l1\_ISIC\_0030061

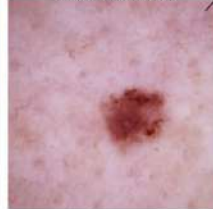

cosine dice l1\_ISIC\_3372750

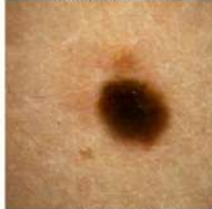

cosine dice l1\_ISIC\_0030061

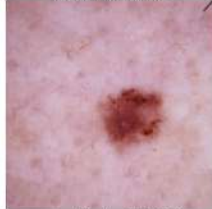

cosine dice l1\_ISIC\_0033982

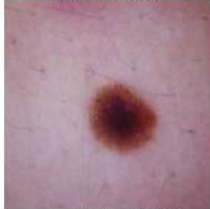

cosine dice l1\_ISIC\_2914669

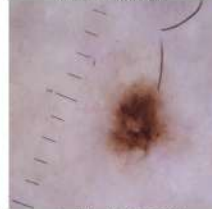

cosine dice l1\_ISIC\_0053551

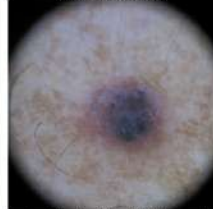

cosine euclidean dice l1\_ISIC\_0033982

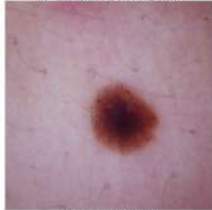

cosine euclidean dice l1\_ISIC\_2914669

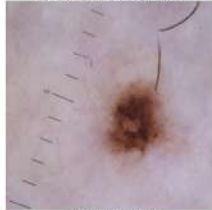

cosine euclidean dice l1\_ISIC\_6609484

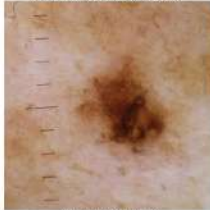

cosine euclidean dice l1\_ISIC\_3372750

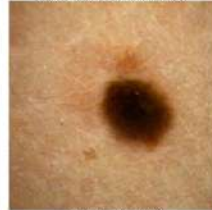

cosine euclidean dice l1\_ISIC\_0013678\_downsampled

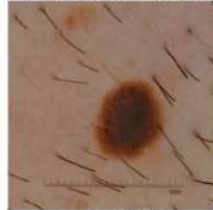

style dice l1\_ISIC\_3495113

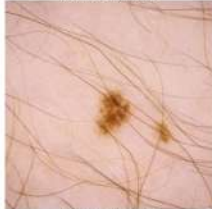

style dice l1\_ISIC\_6394612

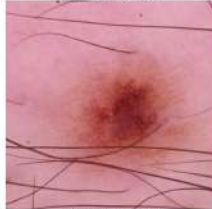

style dice l1\_ISIC\_4308121

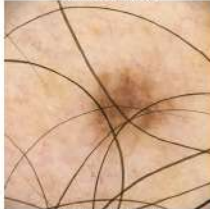

style dice l1\_ISIC\_3372750

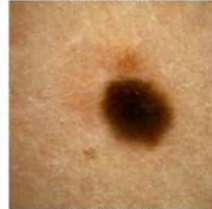

style dice l1\_ISIC\_4390998

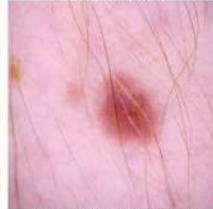

style eucl l1\_ISIC\_4431911

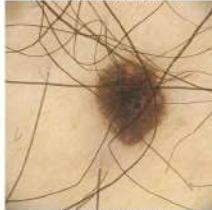

style eucl l1\_ISIC\_2671409

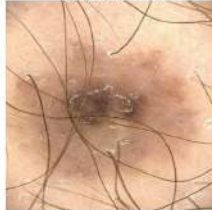

style eucl l1\_ISIC\_7858881

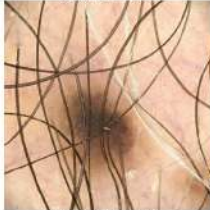

style eucl l1\_ISIC\_2587981

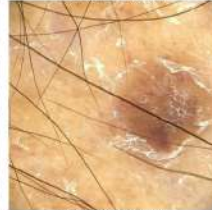

style eucl l1\_ISIC\_0012549\_downsampled

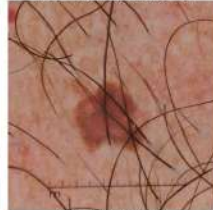

style cosine l1\_ISIC\_2671409

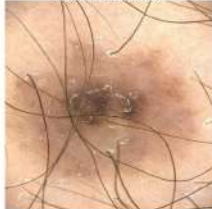

style cosine l1\_ISIC\_2387801

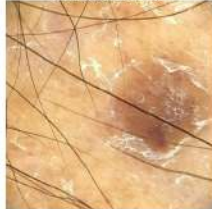

style cosine l1\_ISIC\_4431911

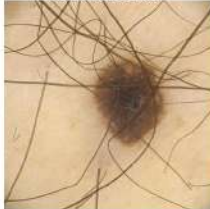

style cosine l1\_ISIC\_7858885

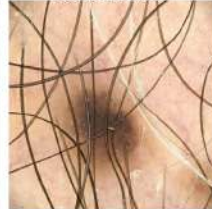

style cosine l1\_ISIC\_5311159

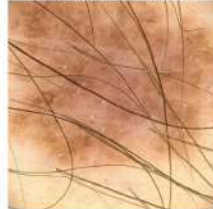

input image - ISIC\_0207137

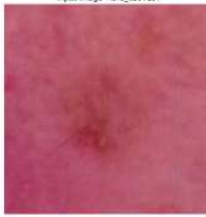

only euclidean\_ISIC\_9950853

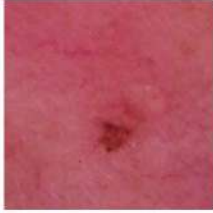

only euclidean\_ISIC\_9456752

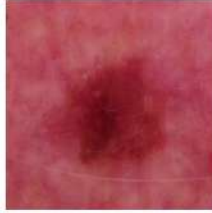

only euclidean\_ISIC\_9031637

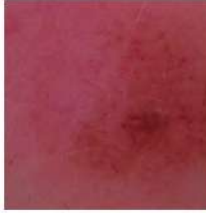

only euclidean\_ISIC\_0189333

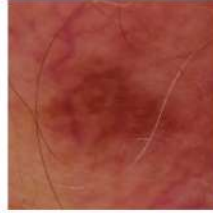

only euclidean\_ISIC\_7582818

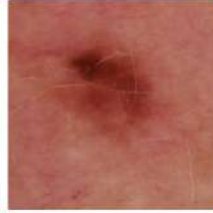

only cosine\_ISIC\_9950853

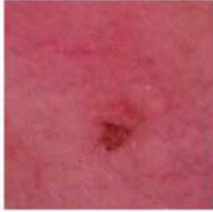

only cosine\_ISIC\_3671274

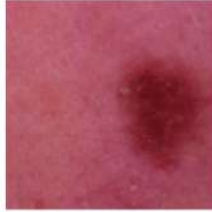

only cosine\_ISIC\_7582818

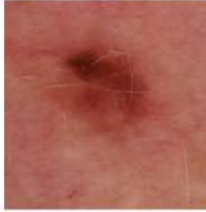

only cosine\_ISIC\_9456752

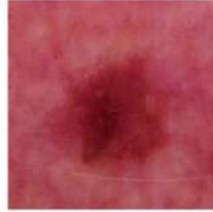

only cosine\_ISIC\_9031637

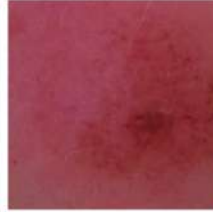

only style loss\_ISIC\_9456752

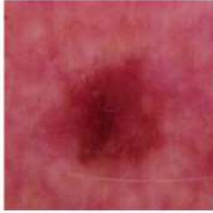

only style loss\_ISIC\_8904639

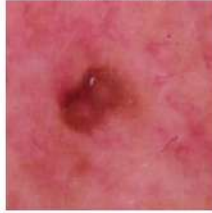

only style loss\_ISIC\_3405391

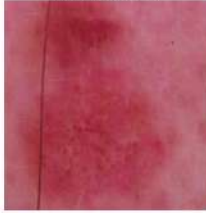

only style loss\_ISIC\_6333067

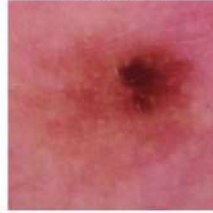

only style loss\_ISIC\_3671274

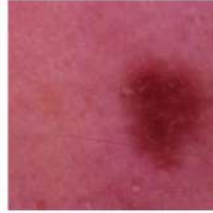

euclidean dice l1\_ISIC\_0027880

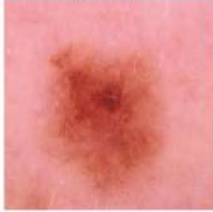

euclidean dice l1\_ISIC\_3490323

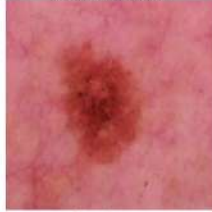

euclidean dice l1\_ISIC\_0780942

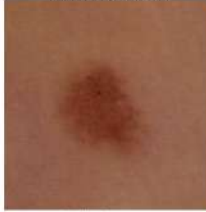

euclidean dice l1\_ISIC\_6342224

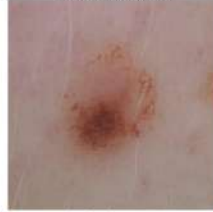

euclidean dice l1\_ISIC\_4223575

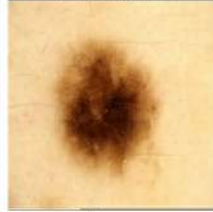

cosine dice l1\_ISIC\_0790942

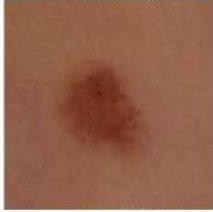

cosine dice l1\_ISIC\_0028205

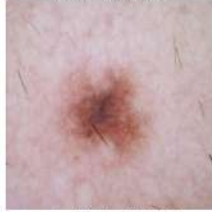

cosine dice l1\_ISIC\_6342224

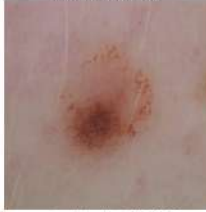

cosine dice l1\_ISIC\_4223575

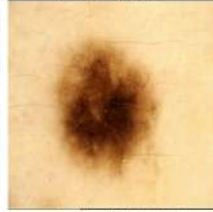

cosine dice l1\_ISIC\_4018473

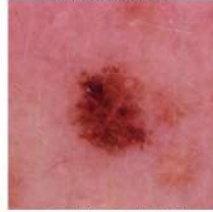

cosine euclidean dice l1\_ISIC\_3490323

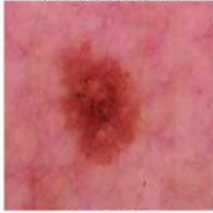

cosine euclidean dice l1\_ISIC\_0027880

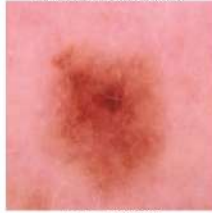

cosine euclidean dice l1\_ISIC\_1988777

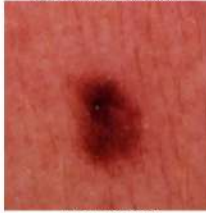

cosine euclidean dice l1\_ISIC\_3588706

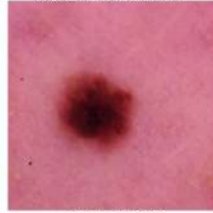

cosine euclidean dice l1\_ISIC\_4223575

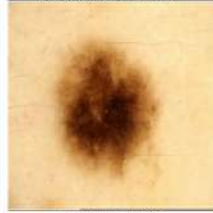

style dice l1\_ISIC\_4018473

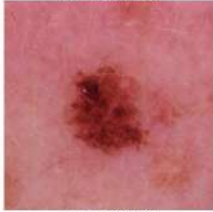

style dice l1\_ISIC\_0780942

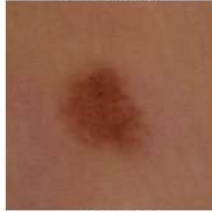

style dice l1\_ISIC\_6352994

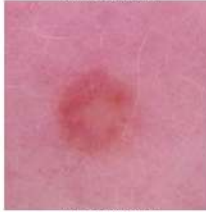

style dice l1\_ISIC\_0026636

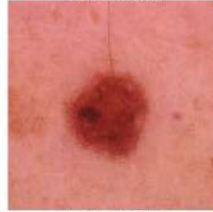

style dice l1\_ISIC\_0028205

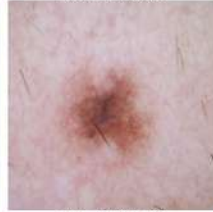

style eucl l1\_ISIC\_9950853

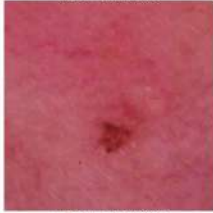

style eucl l1\_ISIC\_9456752

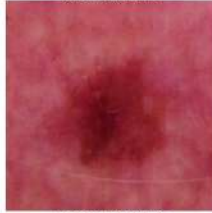

style eucl l1\_ISIC\_9031637

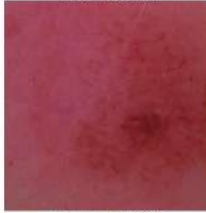

style eucl l1\_ISIC\_3671274

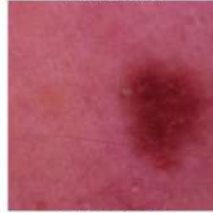

style eucl l1\_ISIC\_5565693

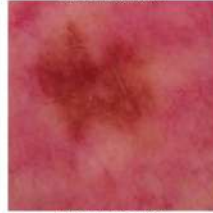

style cosine l1\_ISIC\_9950853

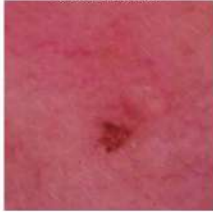

style cosine l1\_ISIC\_3671274

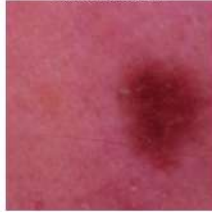

style cosine l1\_ISIC\_9456752

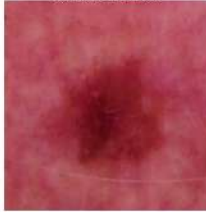

style cosine l1\_ISIC\_9031637

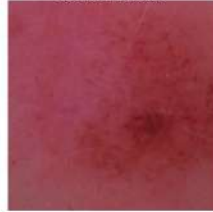

style cosine l1\_ISIC\_7351839

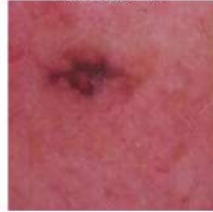

input image - ISIC\_0216447

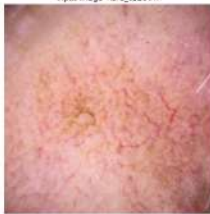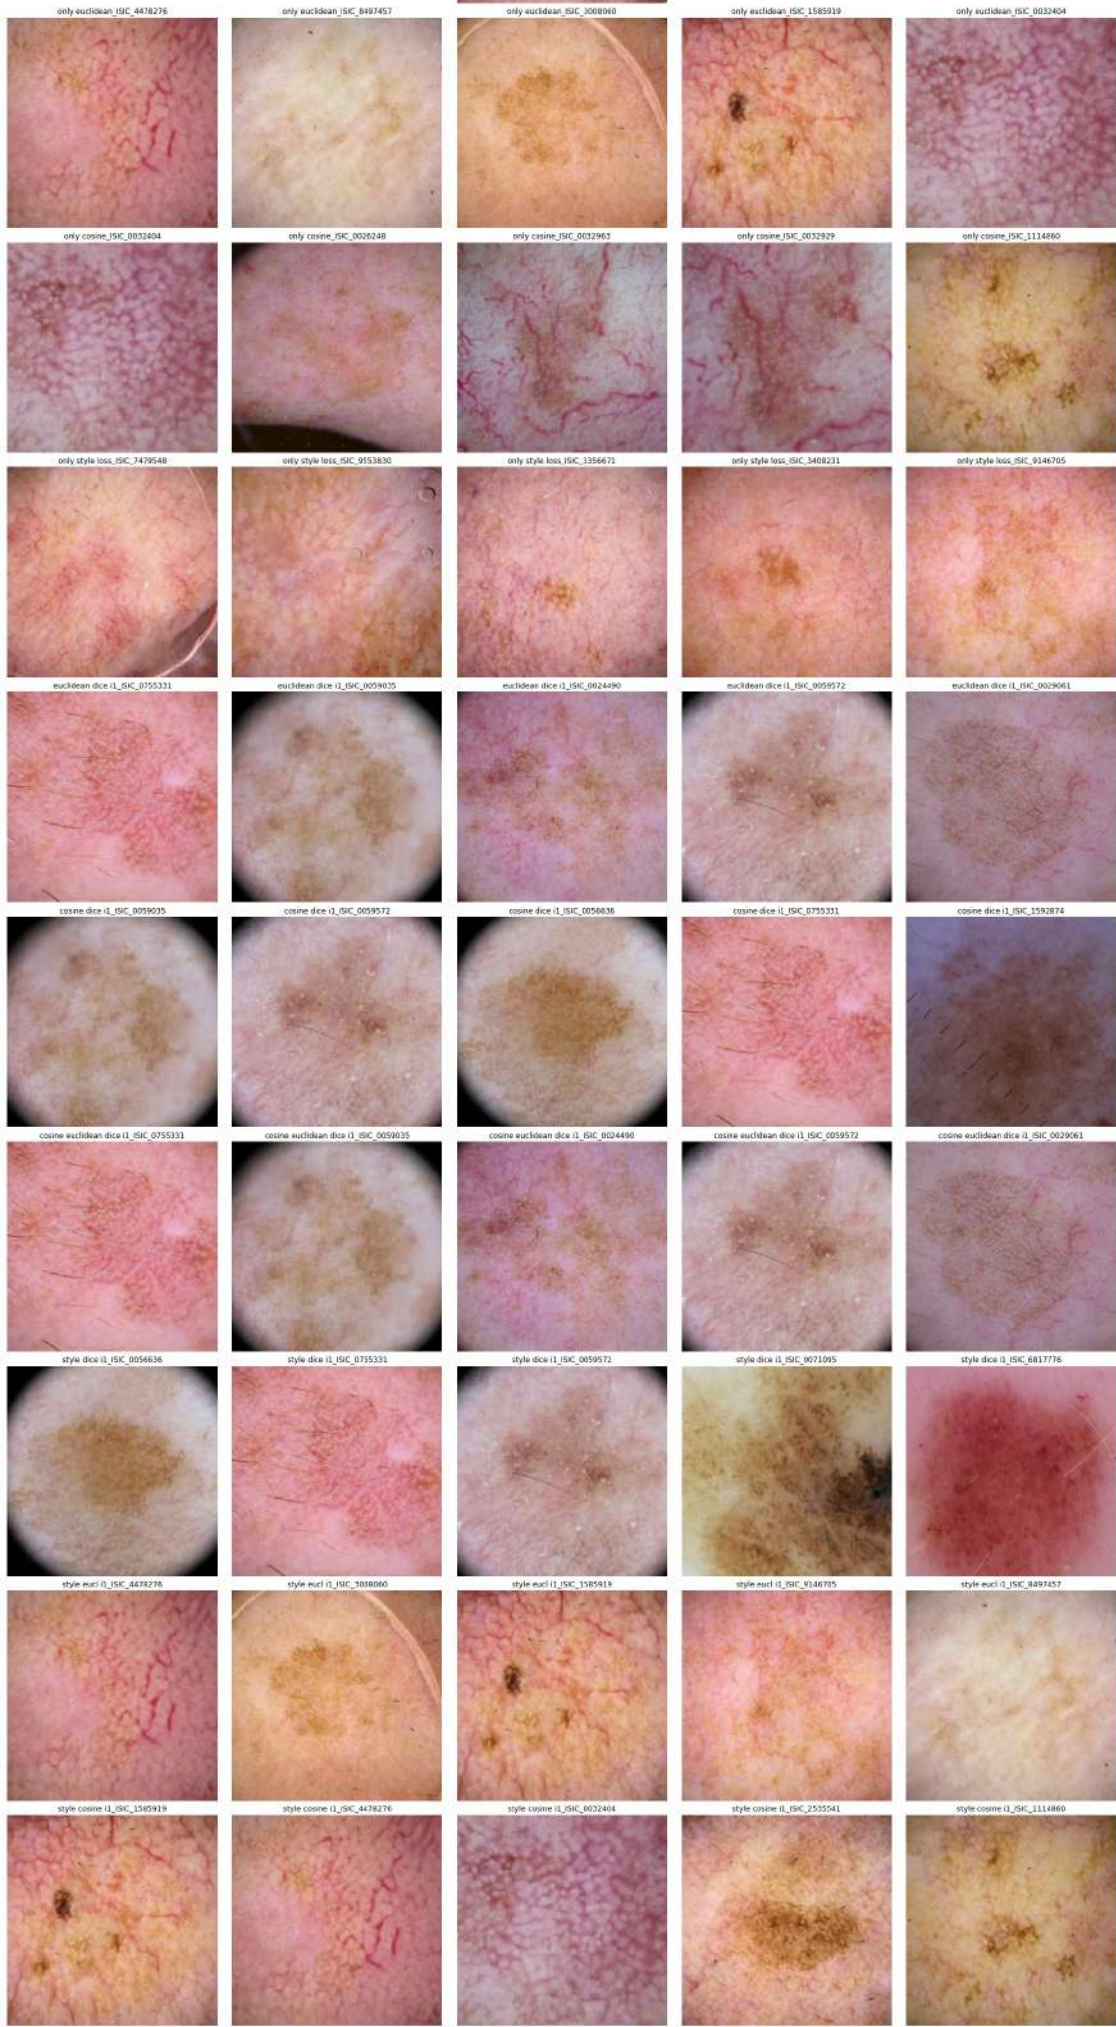



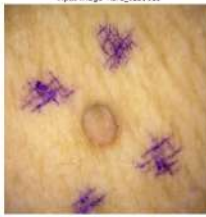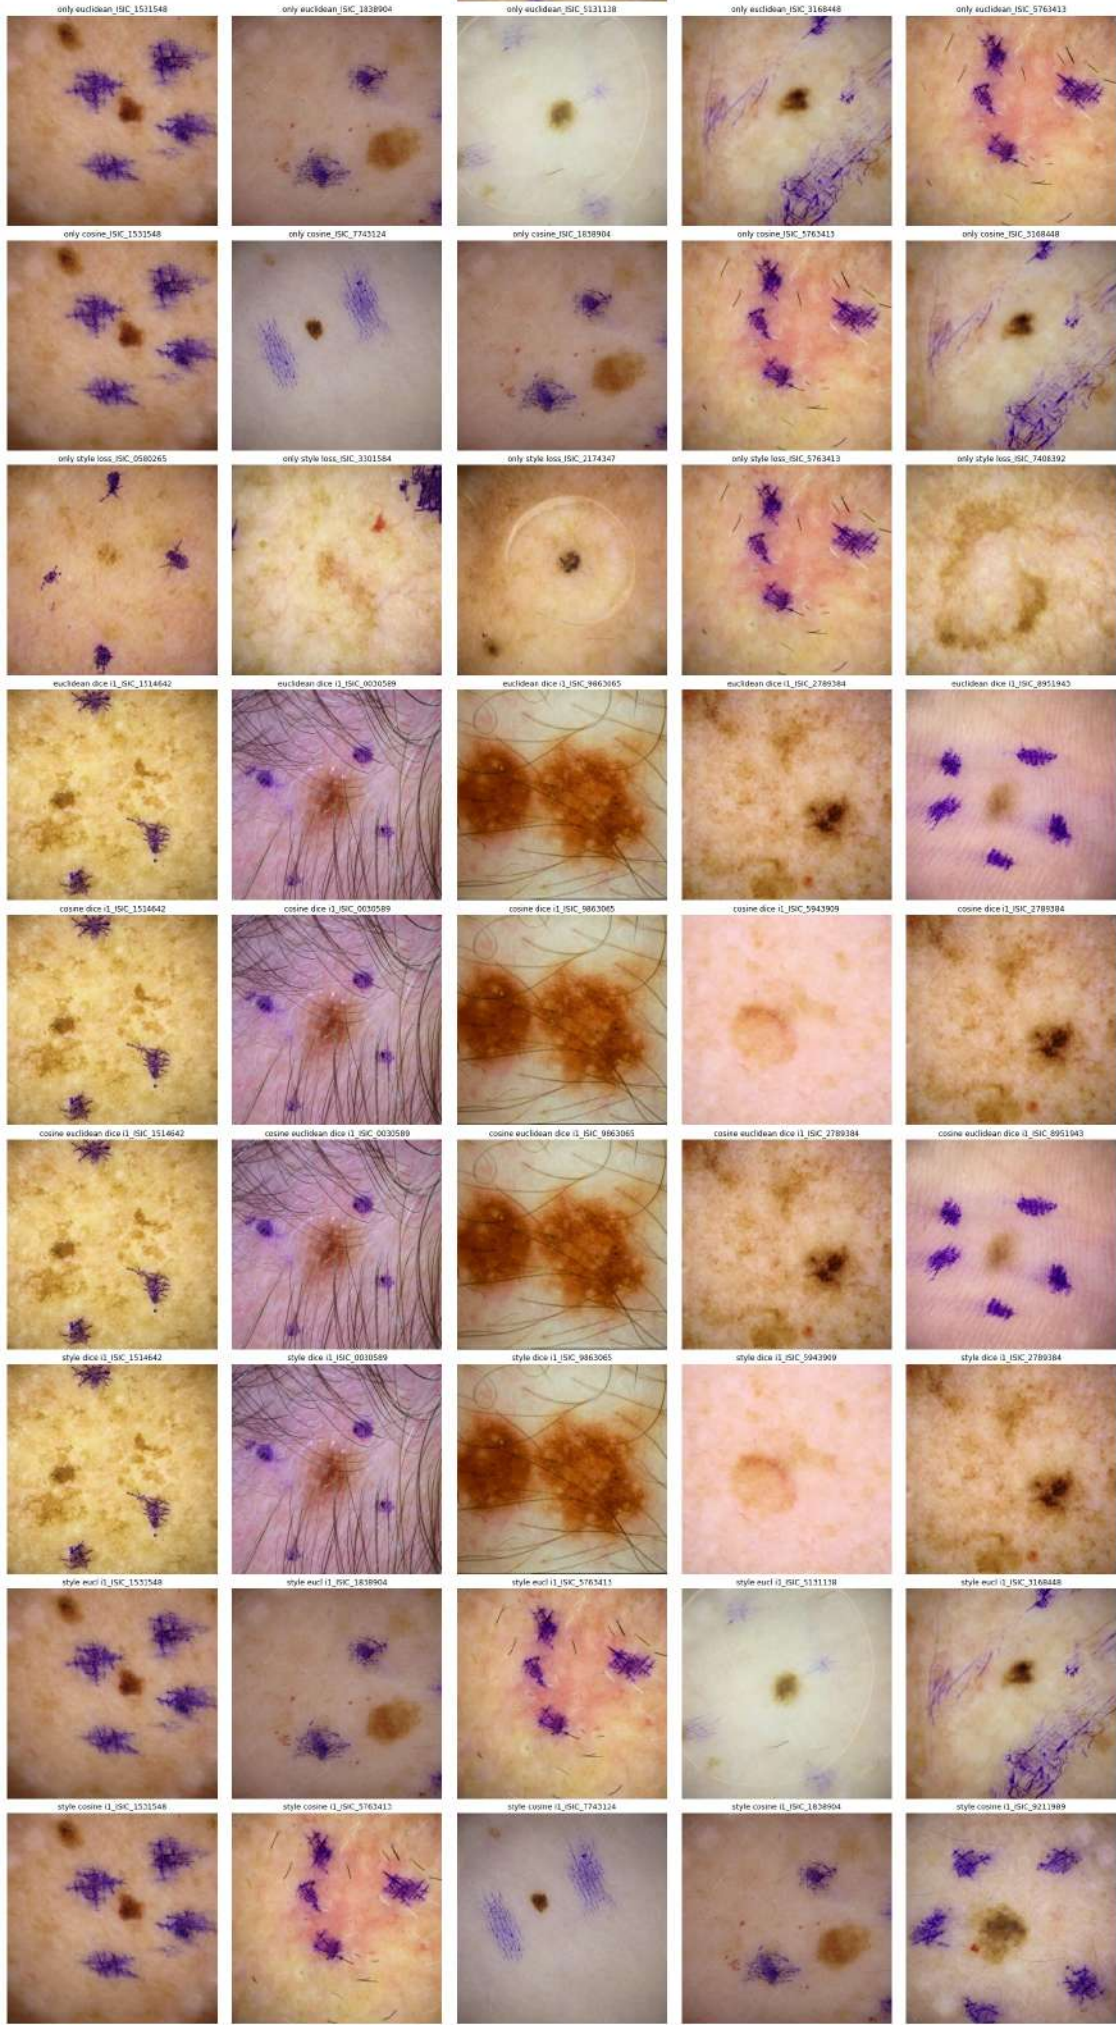

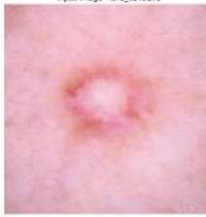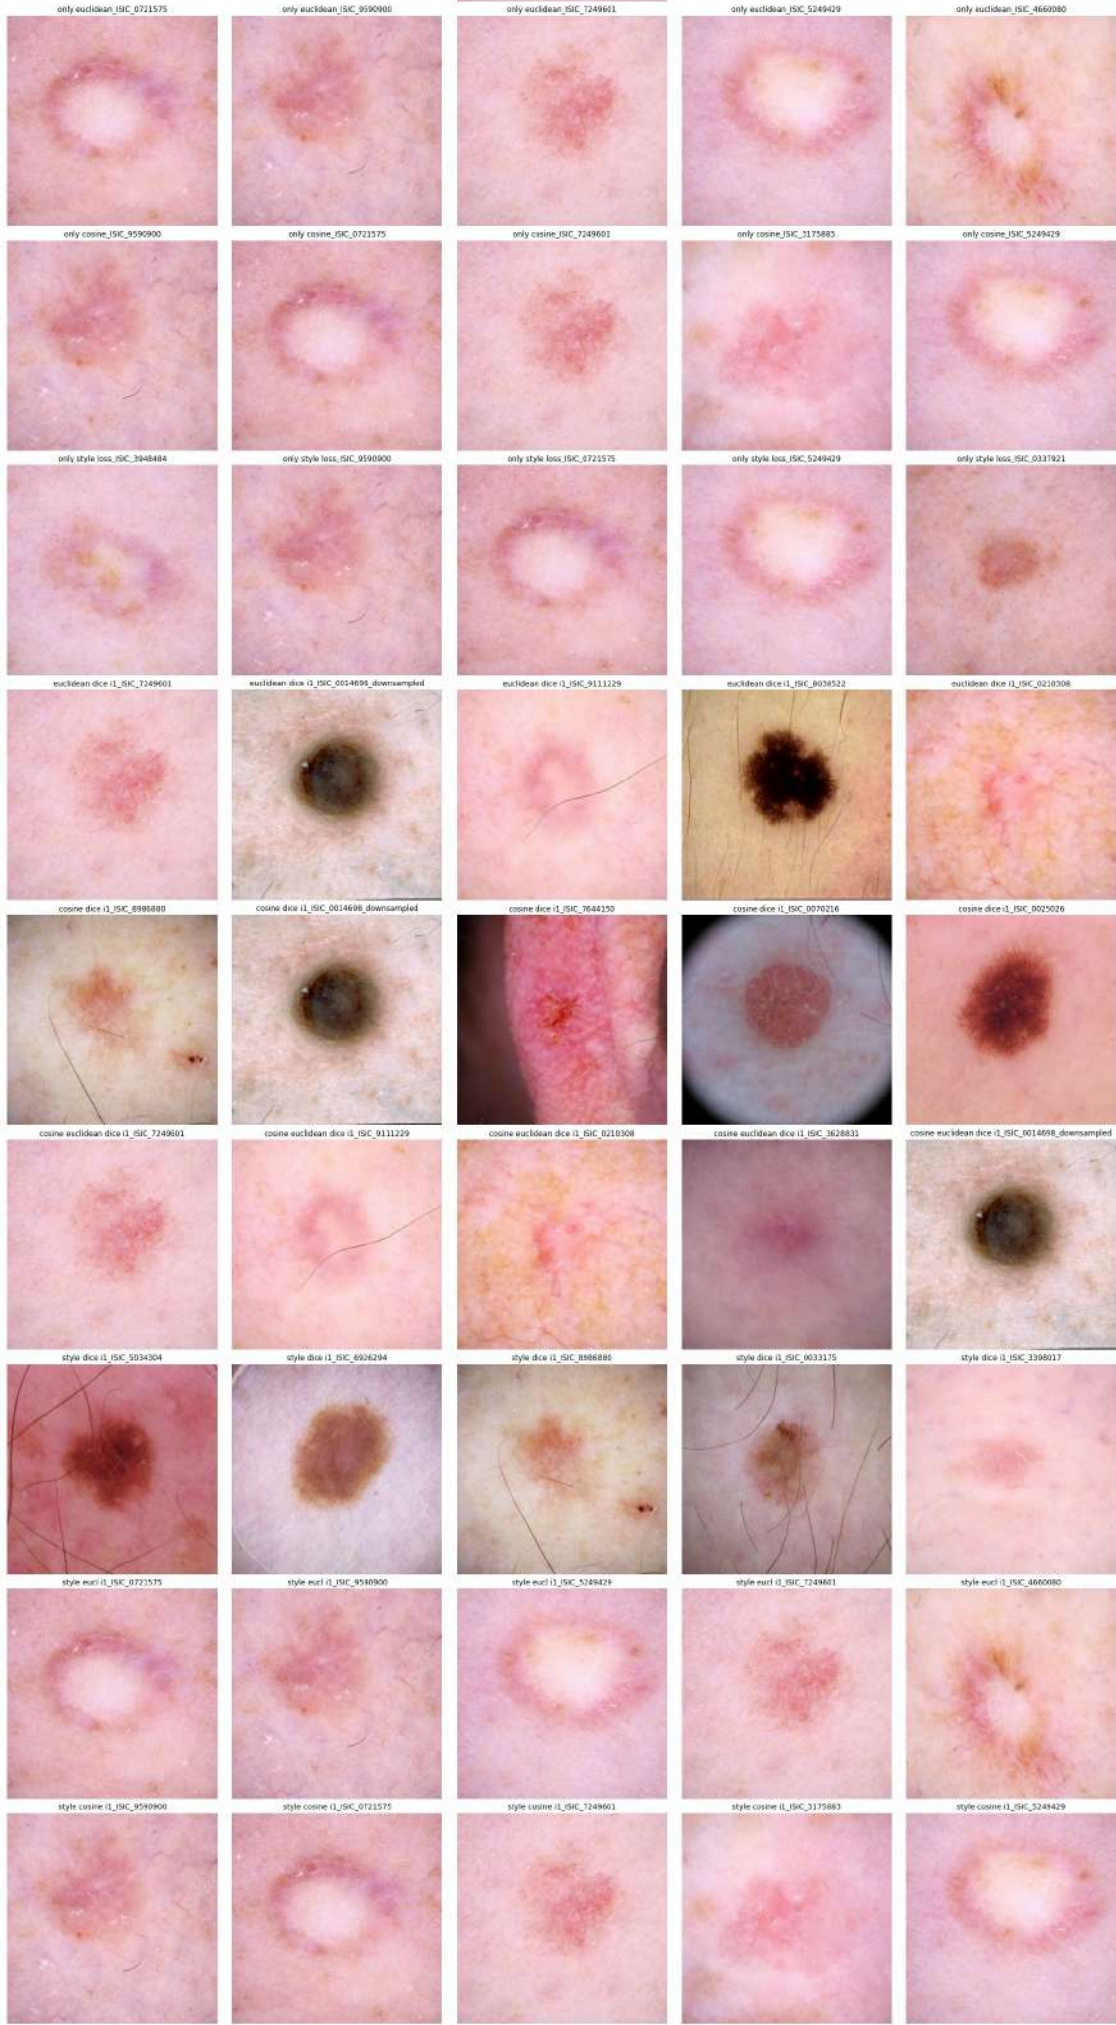

Input image - ISIC\_0267082

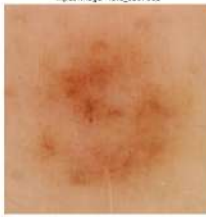

only euclidean\_ISIC\_3625918

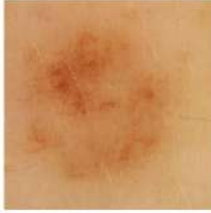

only euclidean\_ISIC\_4871936

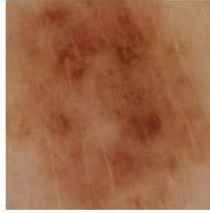

only euclidean\_ISIC\_3833467

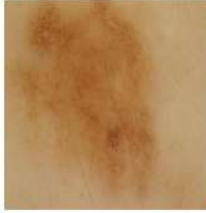

only euclidean\_ISIC\_4583712

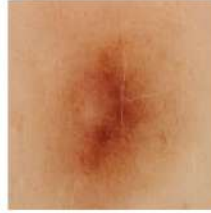

only euclidean\_ISIC\_3071338

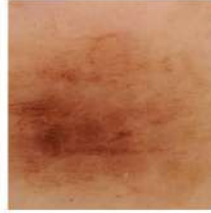

only cosine\_ISIC\_3625918

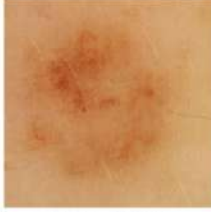

only cosine\_ISIC\_4871936

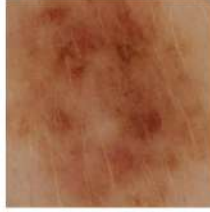

only cosine\_ISIC\_3833467

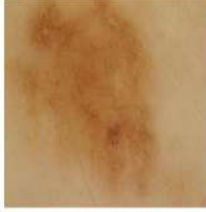

only cosine\_ISIC\_5926079

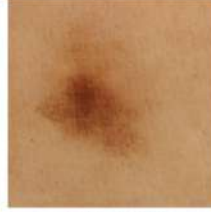

only cosine\_ISIC\_4073425

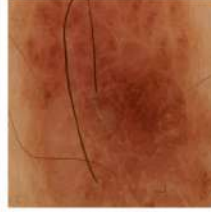

only style loss\_ISIC\_3625918

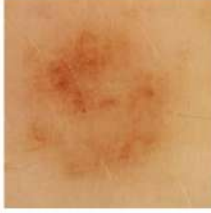

only style loss\_ISIC\_3448546

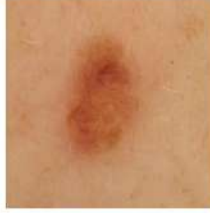

only style loss\_ISIC\_3175837

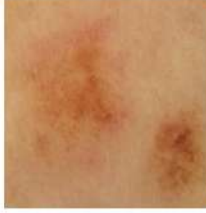

only style loss\_ISIC\_8519402

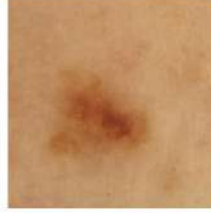

only style loss\_ISIC\_3729749

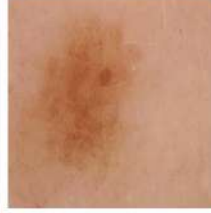

euclidean dice l1\_ISIC\_3817681

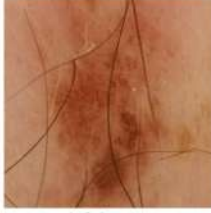

euclidean dice l2\_ISIC\_9025314

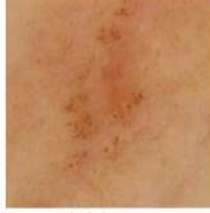

euclidean dice l1\_ISIC\_3200264

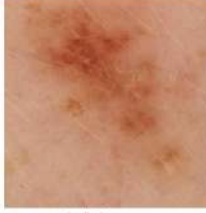

euclidean dice l1\_ISIC\_9884397

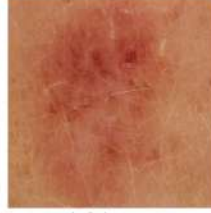

euclidean dice l1\_ISIC\_4924690

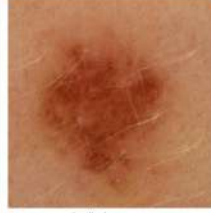

cosine dice l1\_ISIC\_4924690

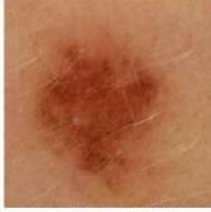

cosine dice l2\_ISIC\_9025314

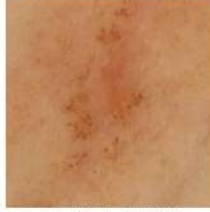

cosine dice l1\_ISIC\_4377099

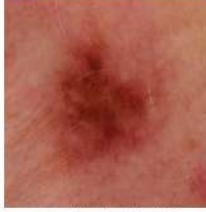

cosine dice l1\_ISIC\_3817681

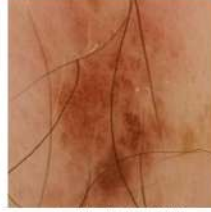

cosine dice l1\_ISIC\_1825481

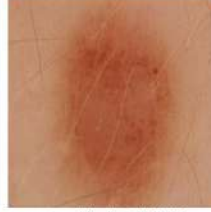

cosine euclidean dice l1\_ISIC\_3817681

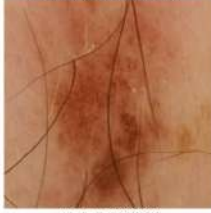

cosine euclidean dice l1\_ISIC\_9025314

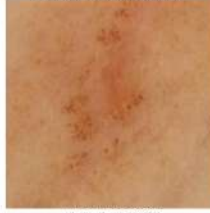

cosine euclidean dice l1\_ISIC\_3200264

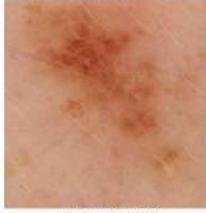

cosine euclidean dice l1\_ISIC\_9884397

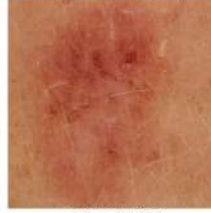

cosine euclidean dice l1\_ISIC\_5089085

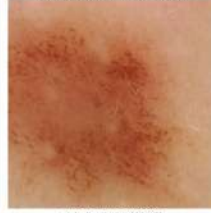

style dice l1\_ISIC\_0031746

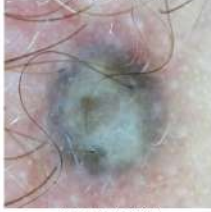

style dice l1\_ISIC\_2386961

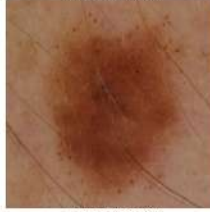

style dice l1\_ISIC\_4924690

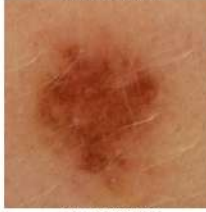

style dice l1\_ISIC\_9465385

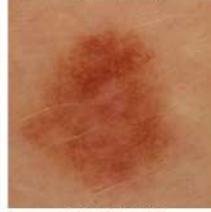

style dice l1\_ISIC\_0069071

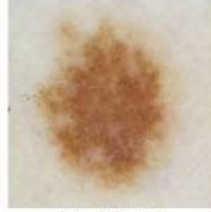

style eucl l1\_ISIC\_3625918

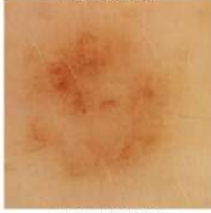

style eucl l1\_ISIC\_4871936

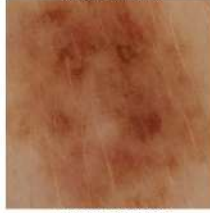

style eucl l1\_ISIC\_4583712

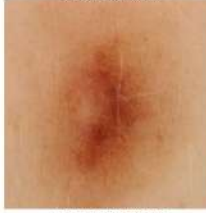

style eucl l1\_ISIC\_3833467

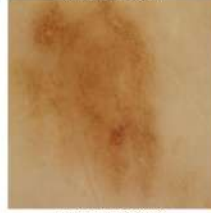

style eucl l1\_ISIC\_1705871

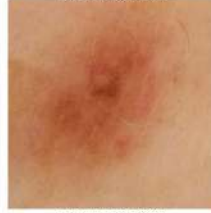

style cosine l1\_ISIC\_3625918

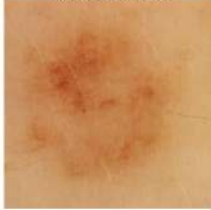

style cosine l1\_ISIC\_4871936

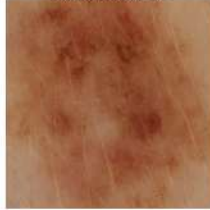

style cosine l1\_ISIC\_3833467

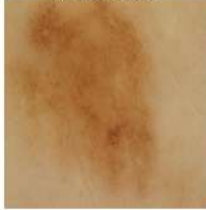

style cosine l1\_ISIC\_5926079

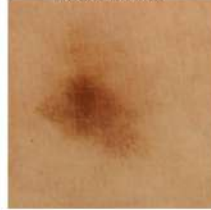

style cosine l1\_ISIC\_3463425

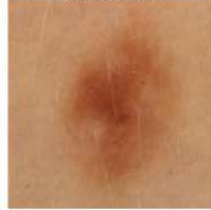



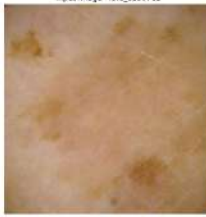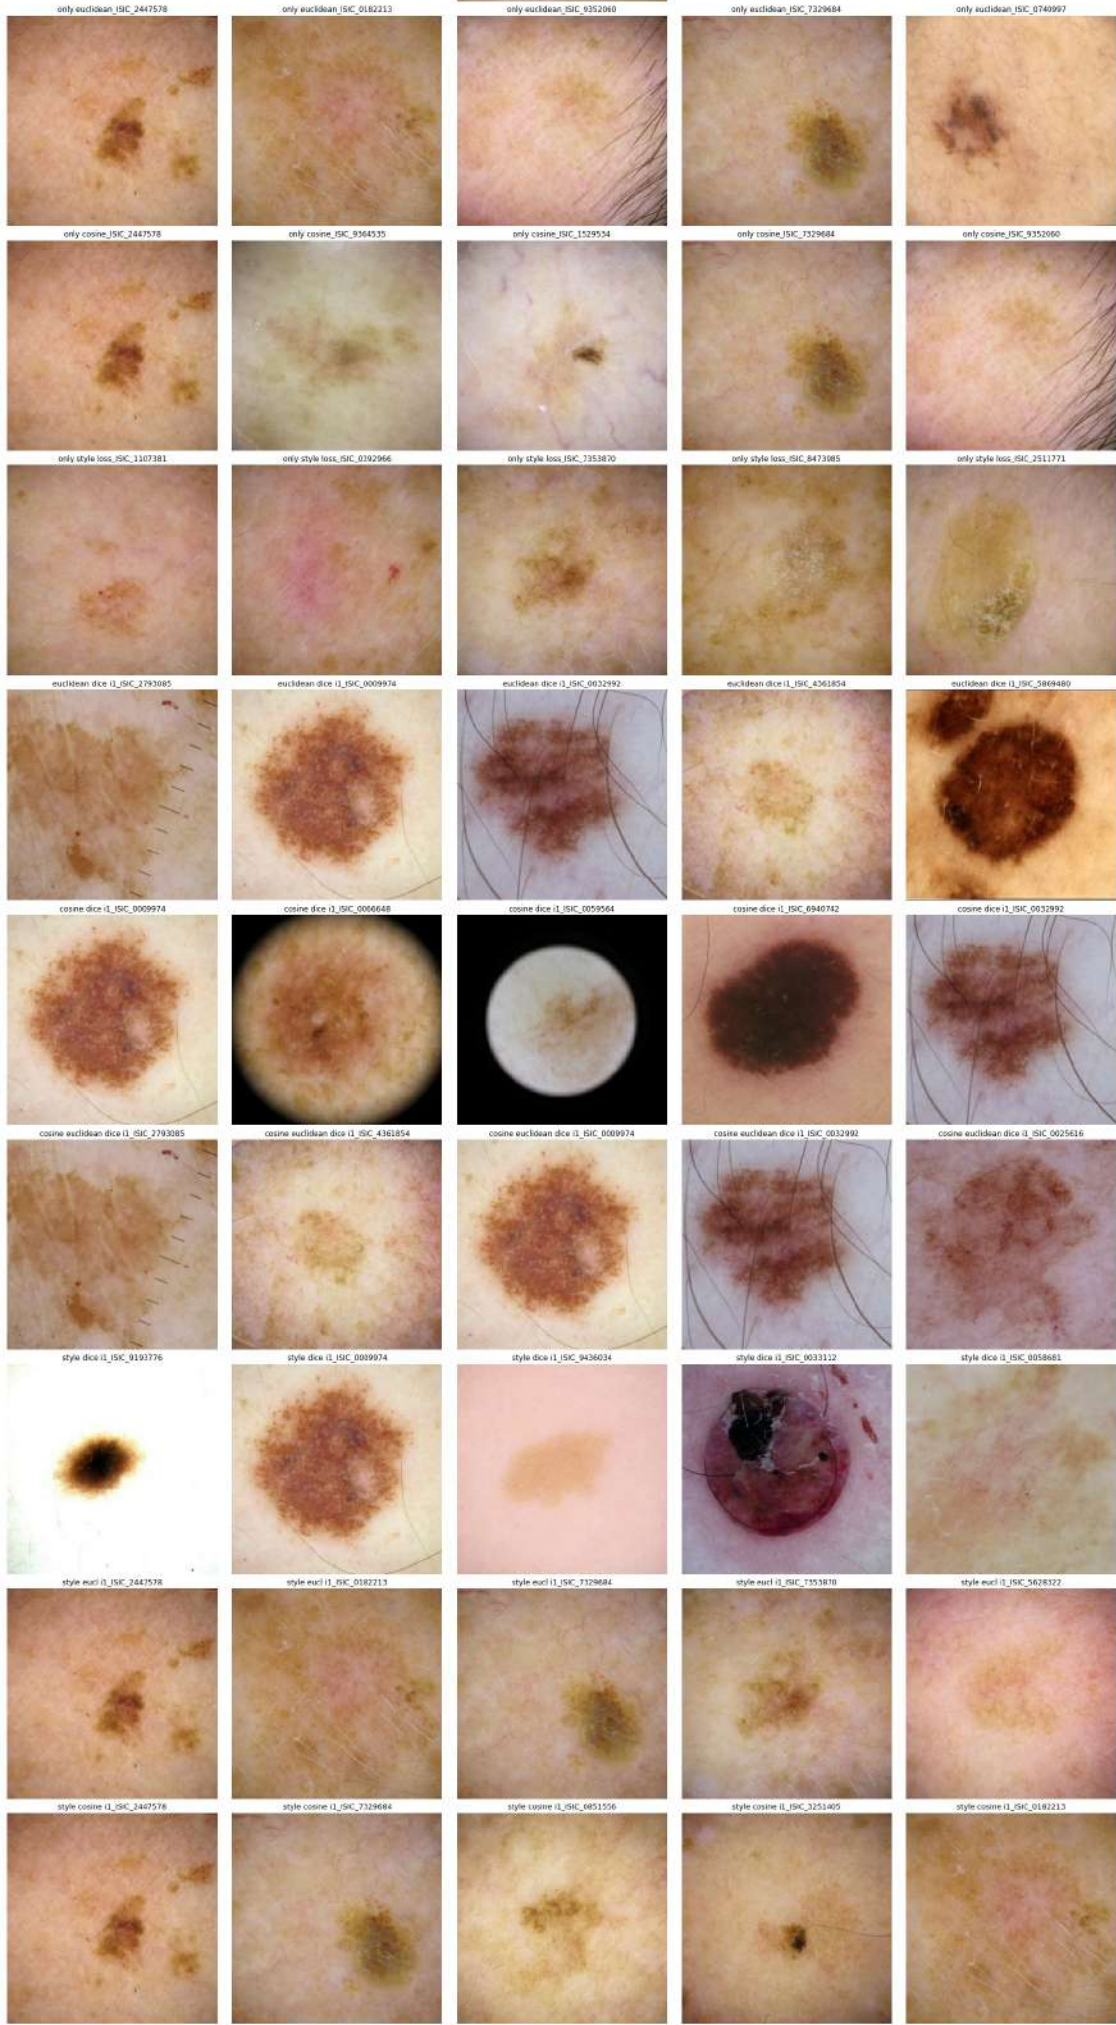

Input image - ISIC\_0299870

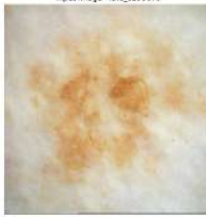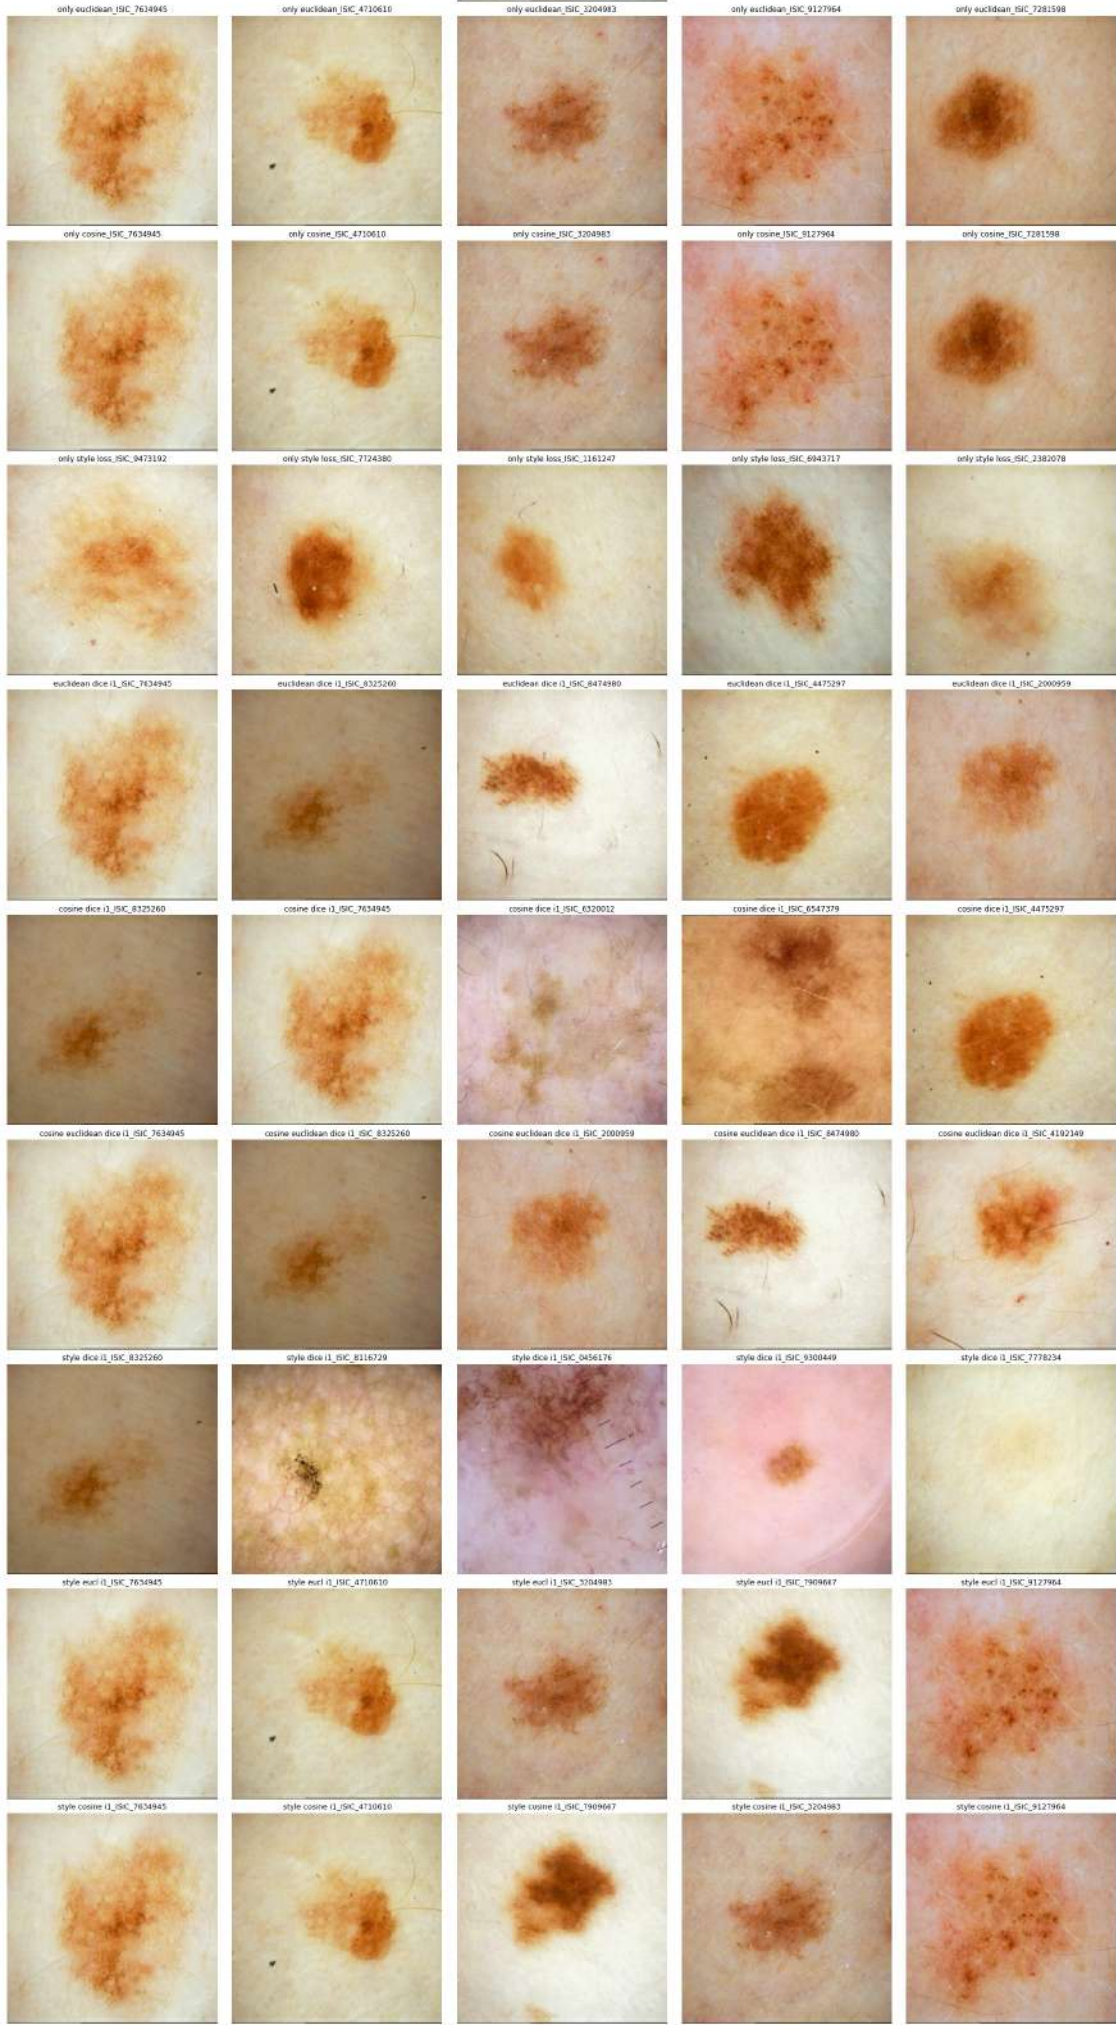

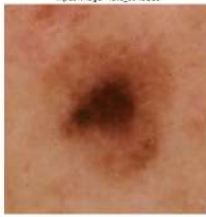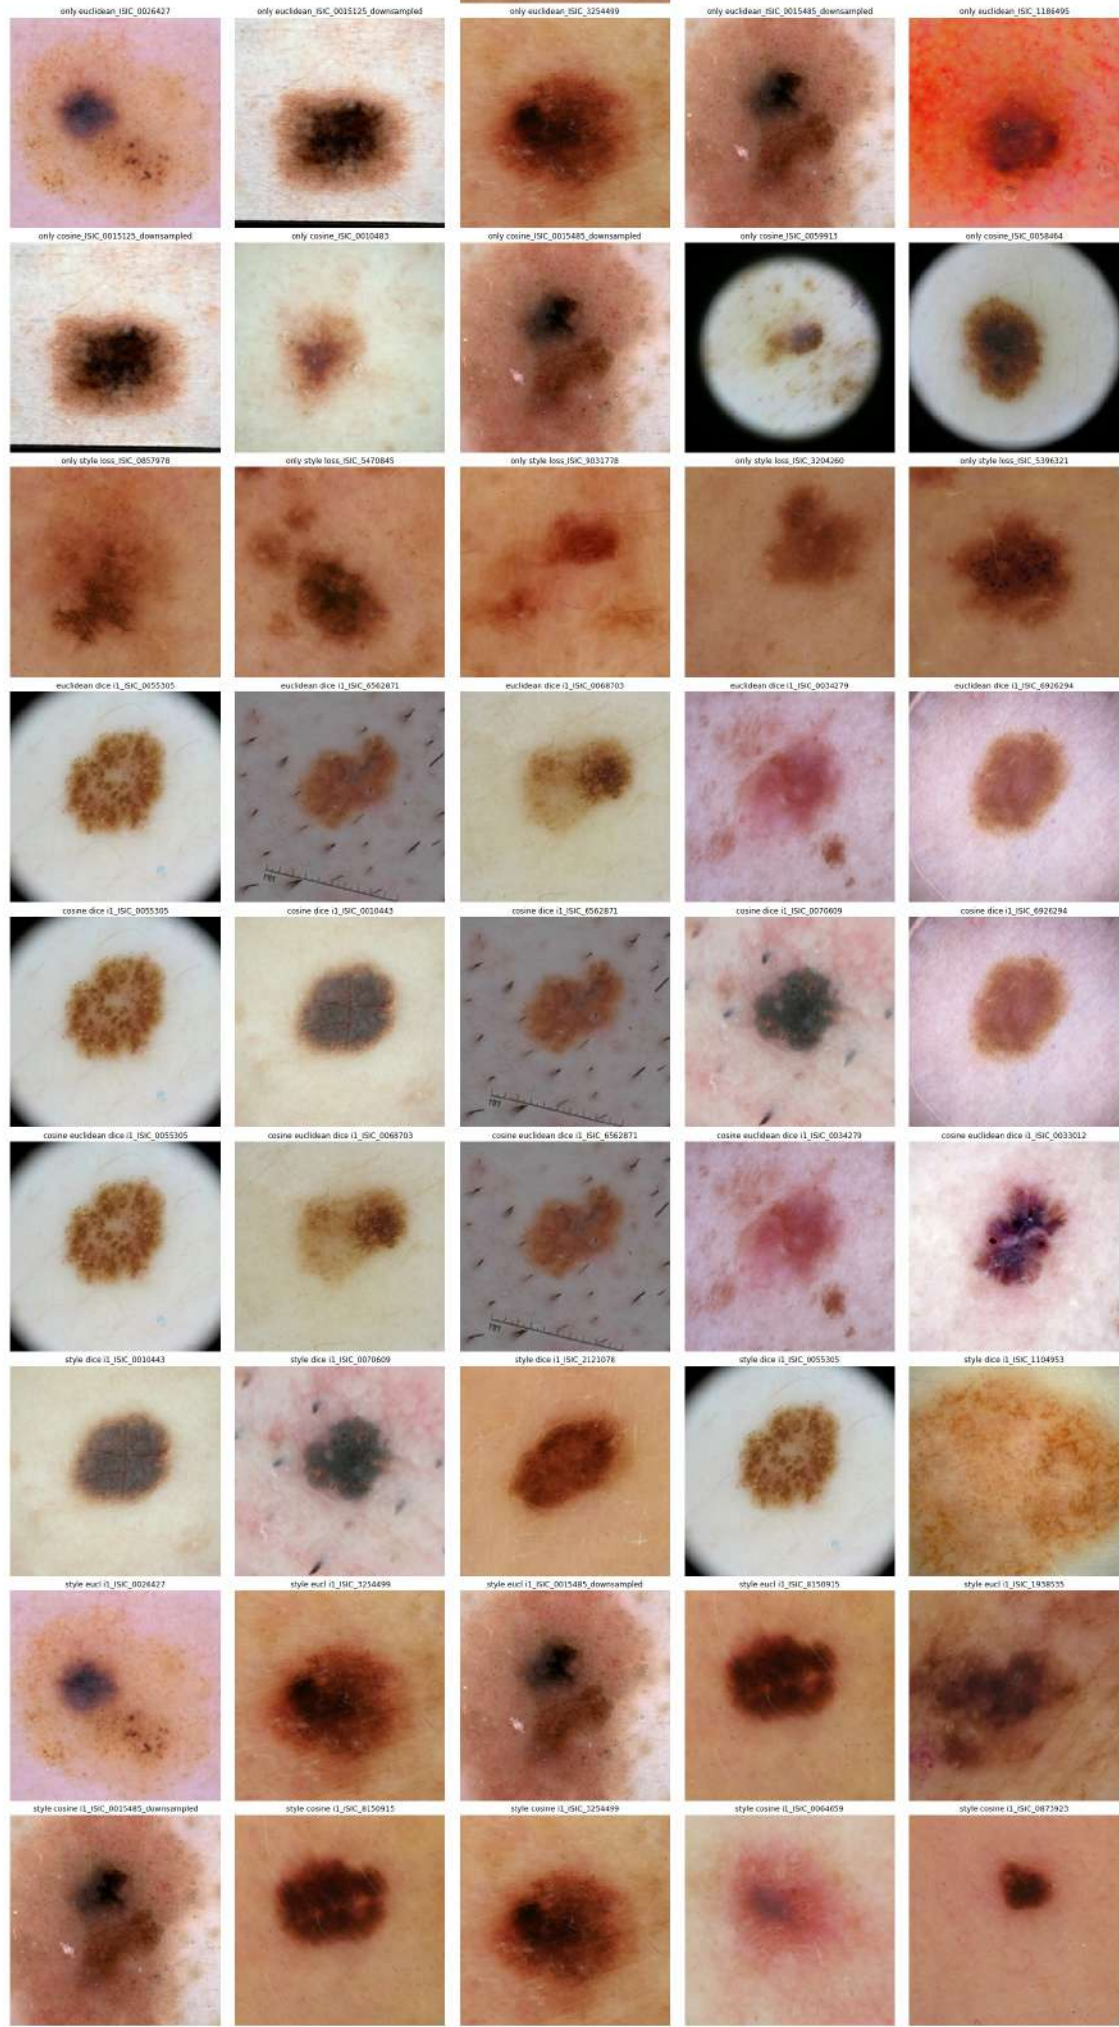

Input image - ISIC\_0368092

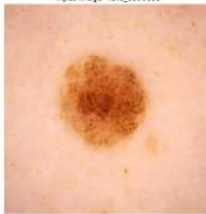

only euclidean\_ISIC\_9918584

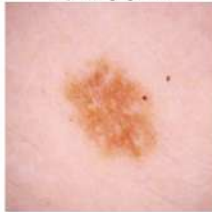

only euclidean\_ISIC\_2957069

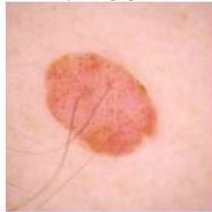

only euclidean\_ISIC\_6628721

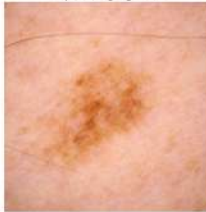

only euclidean\_ISIC\_1753360

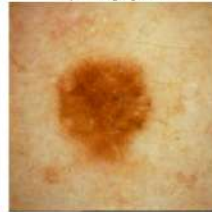

only euclidean\_ISIC\_5065245

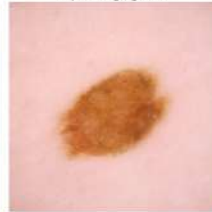

only cosine\_ISIC\_9918584

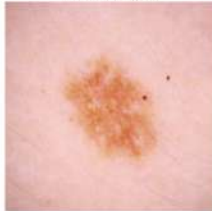

only cosine\_ISIC\_2957069

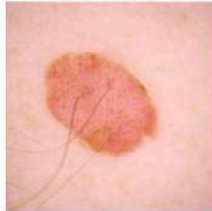

only cosine\_ISIC\_1200819

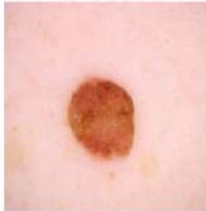

only cosine\_ISIC\_6628721

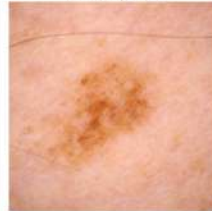

only cosine\_ISIC\_1753360

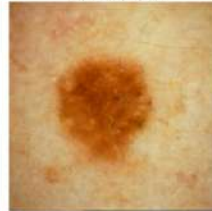

only style loss\_ISIC\_8811316

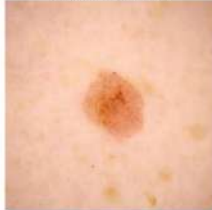

only style loss\_ISIC\_7055743

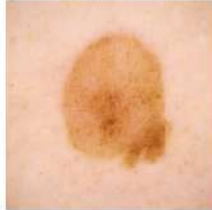

only style loss\_ISIC\_3025923

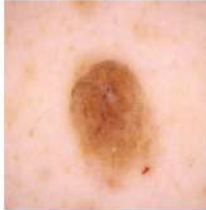

only style loss\_ISIC\_6605684

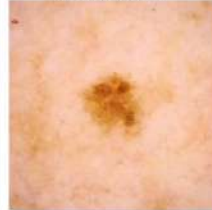

only style loss\_ISIC\_8874925

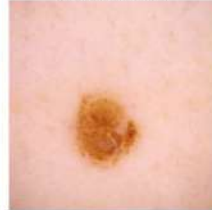

euclidean dice l1\_ISIC\_7327592

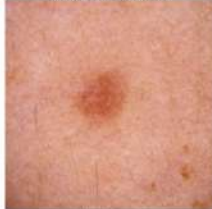

euclidean dice l2\_ISIC\_3592904

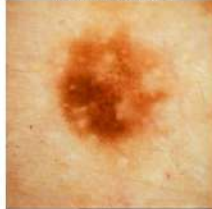

euclidean dice l1\_ISIC\_3157835

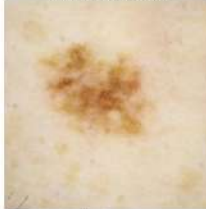

euclidean dice l1\_ISIC\_5055871

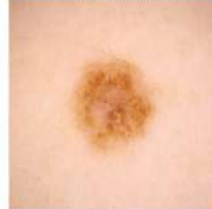

euclidean dice l2\_ISIC\_3567352

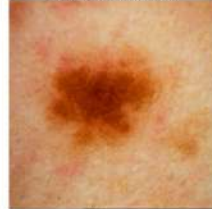

cosine dice l1\_ISIC\_7327592

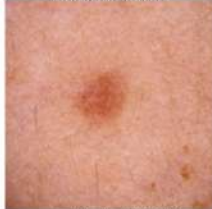

cosine dice l1\_ISIC\_8439036

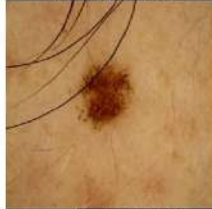

cosine dice l1\_ISIC\_3157835

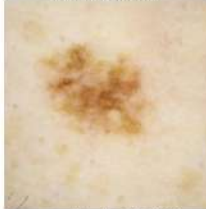

cosine dice l2\_ISIC\_5153725

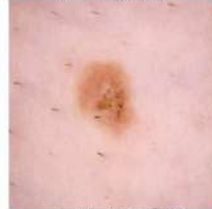

cosine dice l1\_ISIC\_0981883

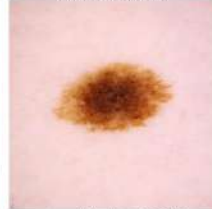

cosine euclidean dice l1\_ISIC\_7327592

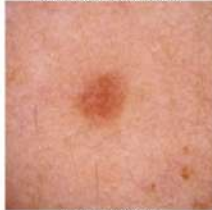

cosine euclidean dice l1\_ISIC\_5055871

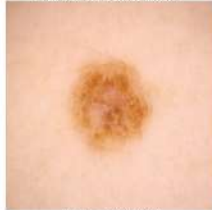

cosine euclidean dice l2\_ISIC\_3592904

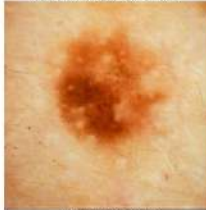

cosine euclidean dice l1\_ISIC\_3157835

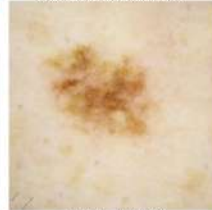

cosine euclidean dice l2\_ISIC\_3567352

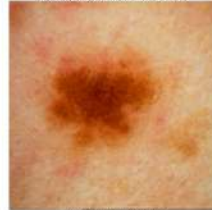

style dice l1\_ISIC\_0028026

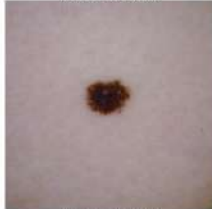

style dice l1\_ISIC\_0011159

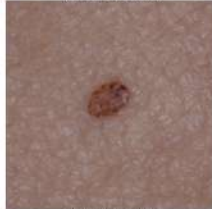

style dice l1\_ISIC\_7327592

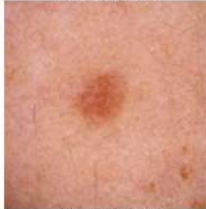

style dice l2\_ISIC\_0027719

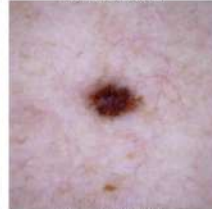

style dice l2\_ISIC\_3491877

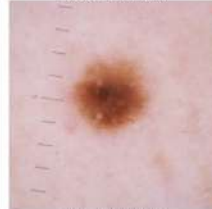

style eucl l1\_ISIC\_9918584

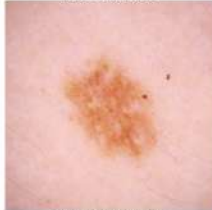

style eucl l1\_ISIC\_2957069

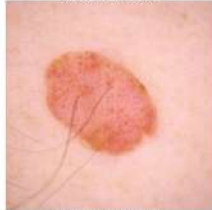

style eucl l1\_ISIC\_6628721

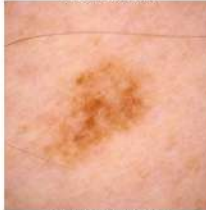

style eucl l2\_ISIC\_1753360

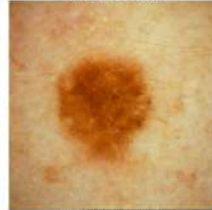

style eucl l2\_ISIC\_5065245

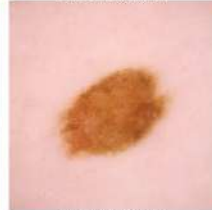

style cosine l1\_ISIC\_9918584

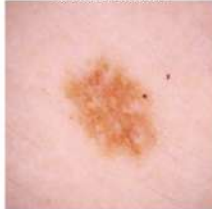

style cosine l1\_ISIC\_2957069

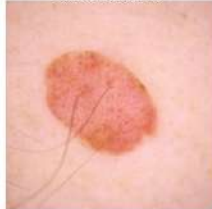

style cosine l1\_ISIC\_1200819

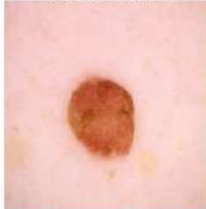

style cosine l2\_ISIC\_7210119

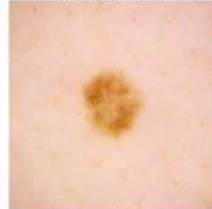

style cosine l2\_ISIC\_3481834

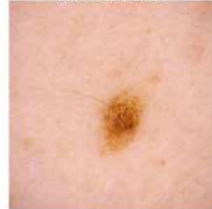

Input image - ISIC\_0371907

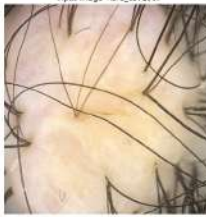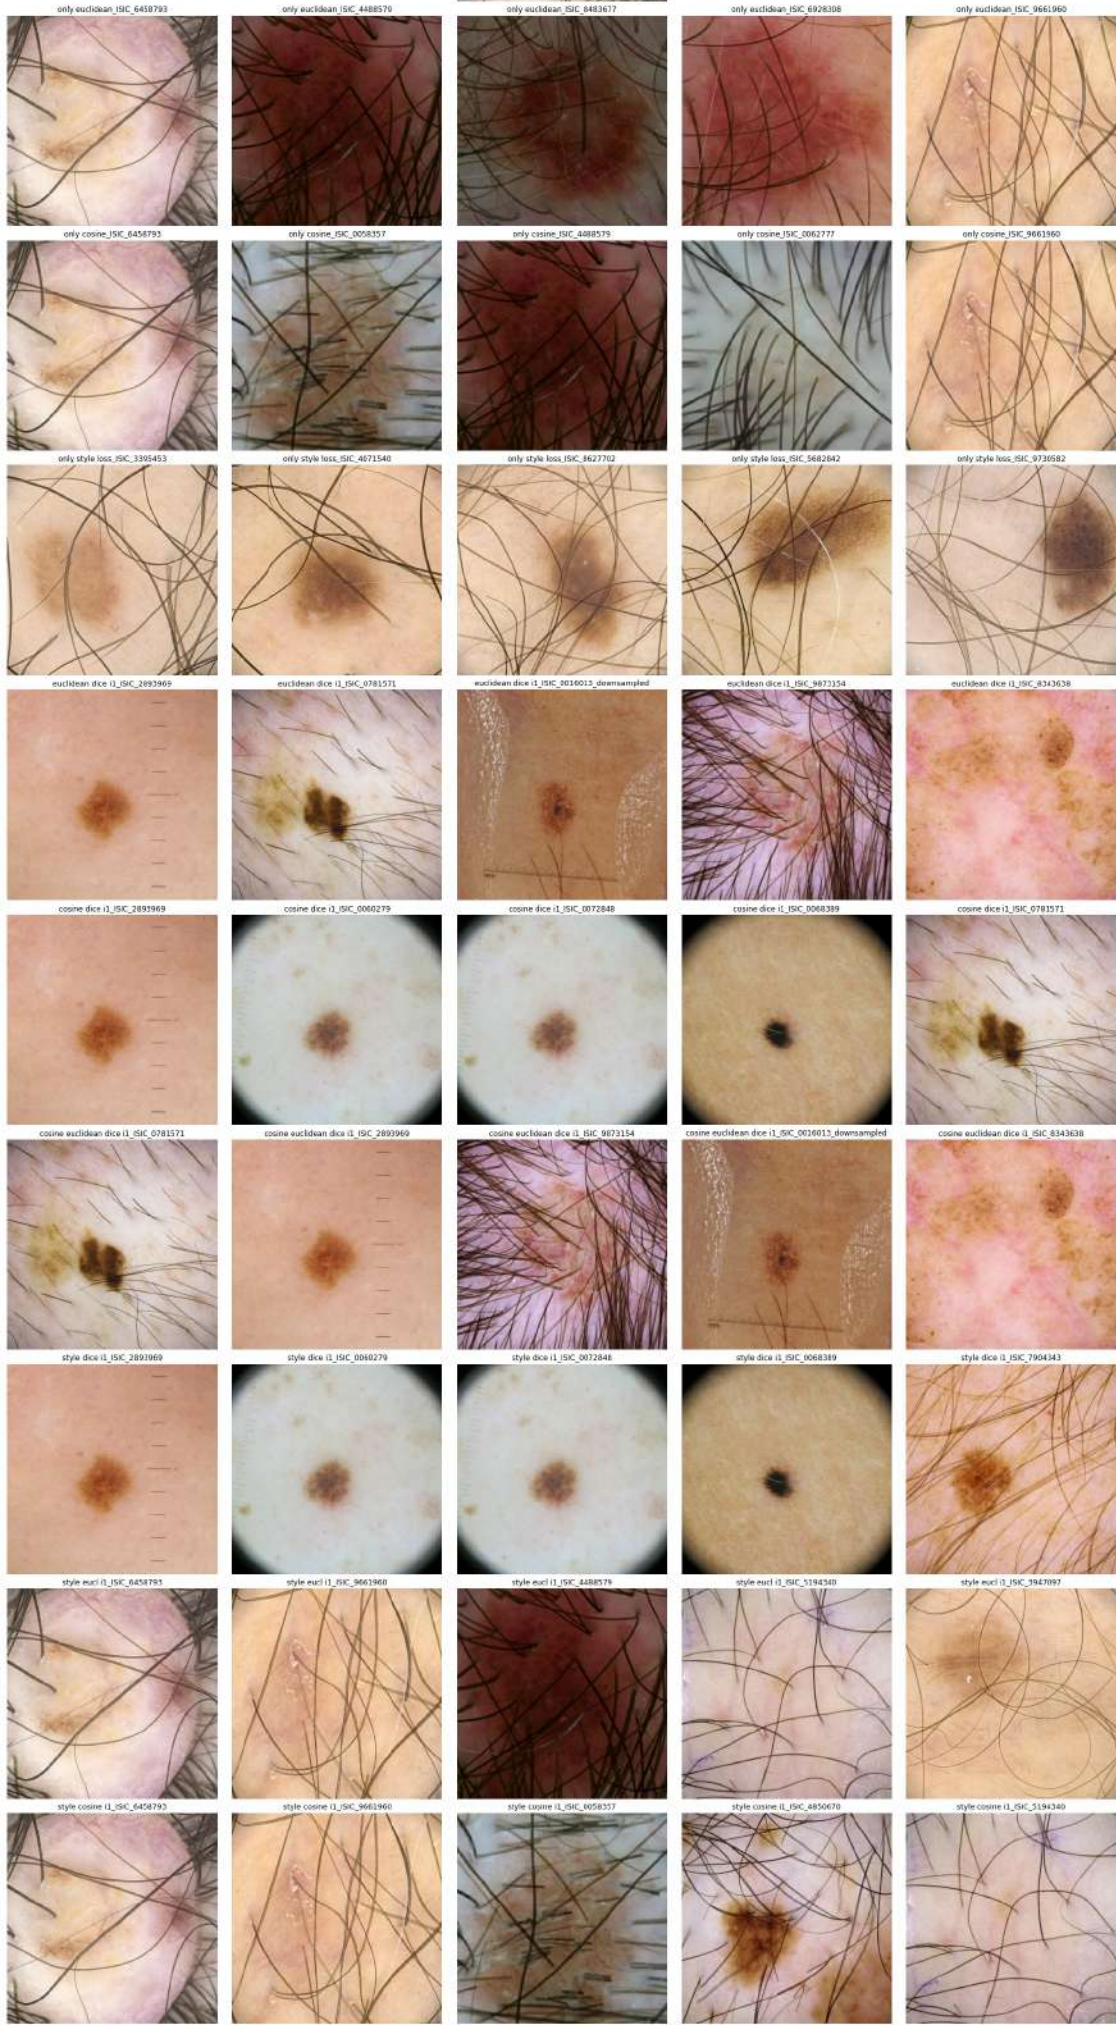

Input Image - ISIC\_0591046

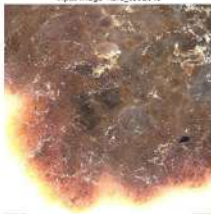

only euclidean\_ISIC\_8814160

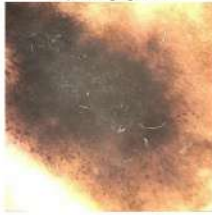

only euclidean\_ISIC\_0671197

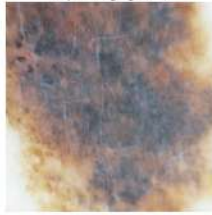

only euclidean\_ISIC\_5541445

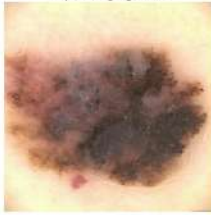

only euclidean\_ISIC\_2568903

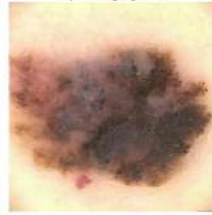

only euclidean\_ISIC\_2218693

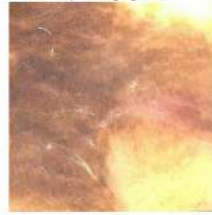

only cosine\_ISIC\_8814160

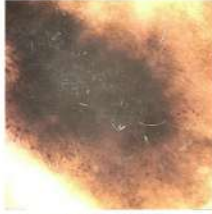

only cosine\_ISIC\_0056044

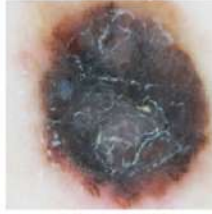

only cosine\_ISIC\_2568903

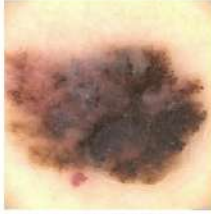

only cosine\_ISIC\_5541445

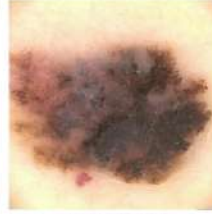

only cosine\_ISIC\_0062239

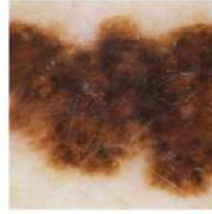

only style loss\_ISIC\_7208452

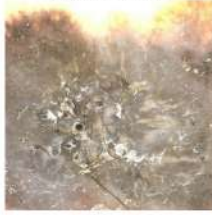

only style loss\_ISIC\_2887299

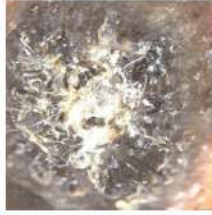

only style loss\_ISIC\_4519116

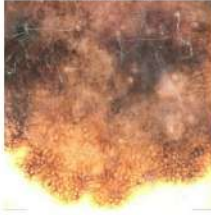

only style loss\_ISIC\_4219443

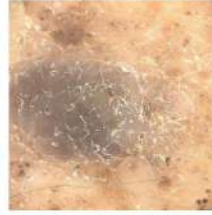

only style loss\_ISIC\_5688896

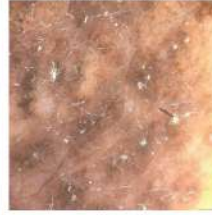

euclidean dice l1\_ISIC\_0610723

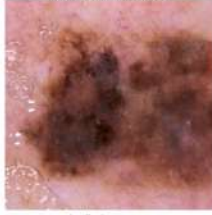

euclidean dice l2\_ISIC\_6426806

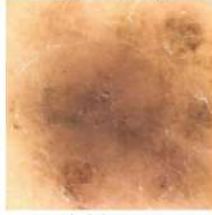

euclidean dice l1\_ISIC\_0032873

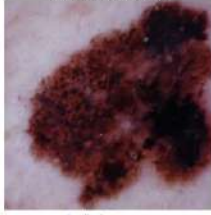

euclidean dice l1\_ISIC\_0569831

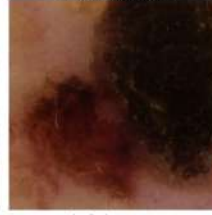

euclidean dice l1\_ISIC\_0010036

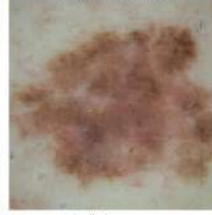

cosine dice l1\_ISIC\_0068310

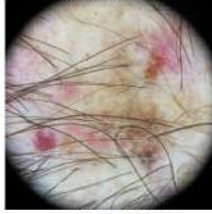

cosine dice l2\_ISIC\_0032873

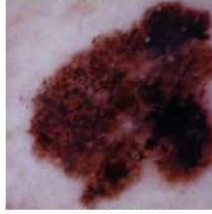

cosine dice l1\_ISIC\_0011495

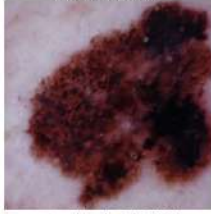

cosine dice l1\_ISIC\_0010723

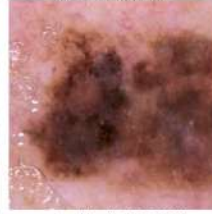

cosine dice l1\_ISIC\_0056937

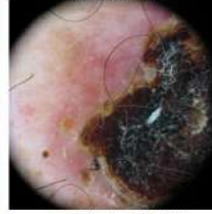

cosine euclidean dice l1\_ISIC\_6426806

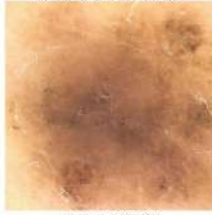

cosine euclidean dice l1\_ISIC\_7886355

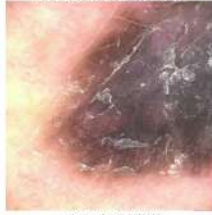

cosine euclidean dice l2\_ISIC\_0010723

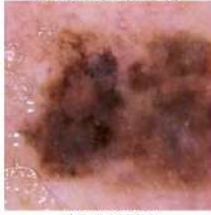

cosine euclidean dice l1\_ISIC\_0066500

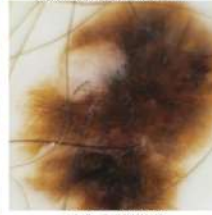

cosine euclidean dice l1\_ISIC\_0010036

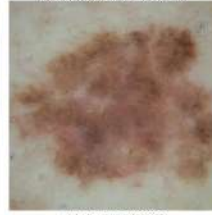

style dice l1\_ISIC\_9191776

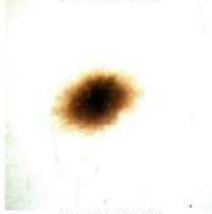

style dice l1\_ISIC\_0068310

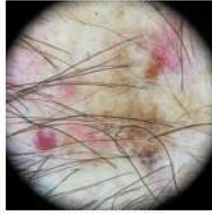

style dice l1\_ISIC\_0030652

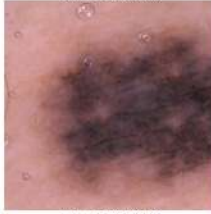

style dice l1\_ISIC\_0011495

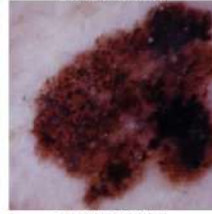

style dice l1\_ISIC\_0032873

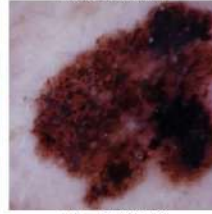

style eucl l1\_ISIC\_8814160

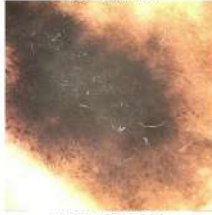

style eucl l1\_ISIC\_2568903

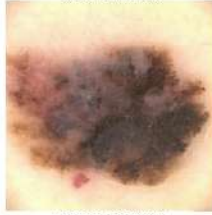

style eucl l1\_ISIC\_5541445

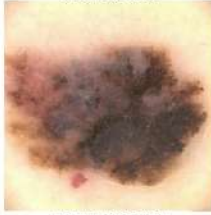

style eucl l1\_ISIC\_2218693

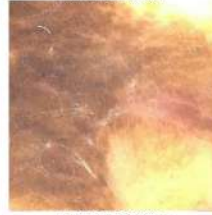

style eucl l1\_ISIC\_2887299

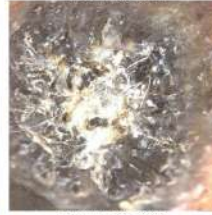

style cosine l1\_ISIC\_8814160

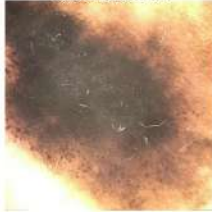

style cosine l1\_ISIC\_7208452

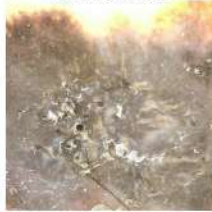

style cosine l1\_ISIC\_2887299

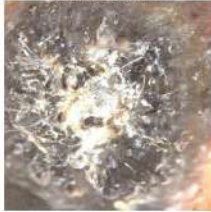

style cosine l1\_ISIC\_5688896

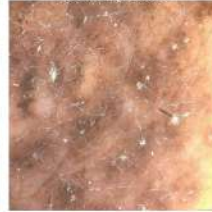

style cosine l1\_ISIC\_7886355

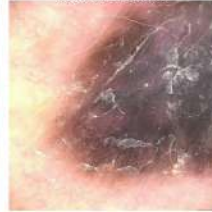

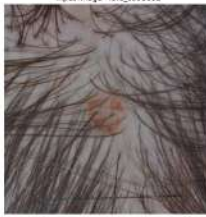

only euclidean\_ISIC\_5873539

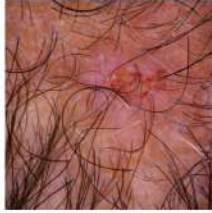

only euclidean\_ISIC\_9488995

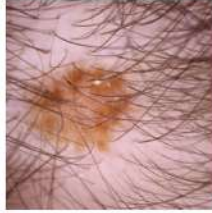

only euclidean\_ISIC\_4677073

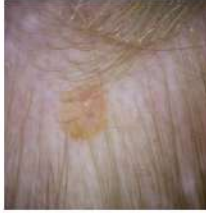

only euclidean\_ISIC\_6432615

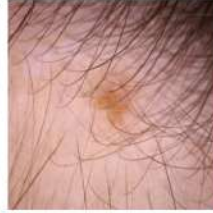

only euclidean\_ISIC\_7782029

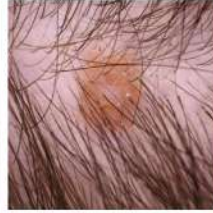

only cosine\_ISIC\_9488995

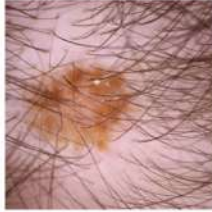

only cosine\_ISIC\_6432615

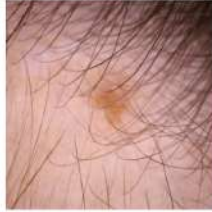

only cosine\_ISIC\_5873539

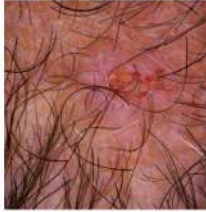

only cosine\_ISIC\_4677073

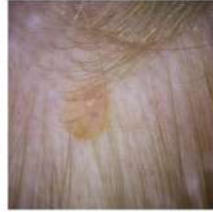

only cosine\_ISIC\_7059744

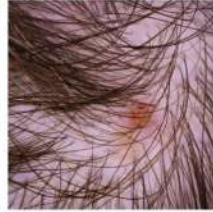

only style loss\_ISIC\_0011167\_downsampled

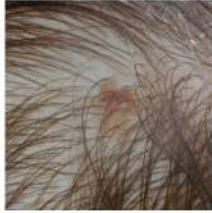

only style loss\_ISIC\_0012149\_downsampled

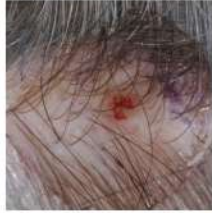

only style loss\_ISIC\_3541028

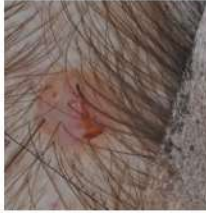

only style loss\_ISIC\_6694200

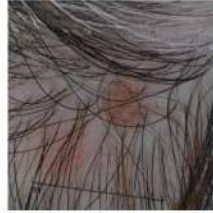

only style loss\_ISIC\_0071570

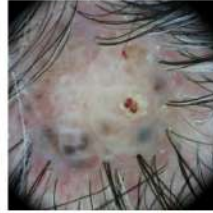

euclidean dice l1\_ISIC\_1187477

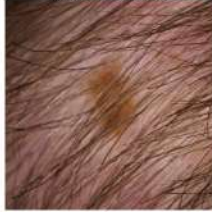

euclidean dice l2\_ISIC\_9023820

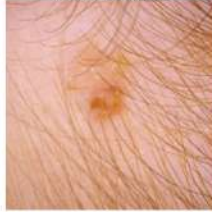

euclidean dice l1\_ISIC\_0877919

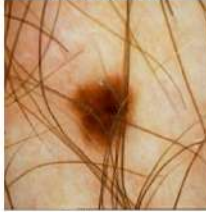

euclidean dice l1\_ISIC\_0007157\_downsampled

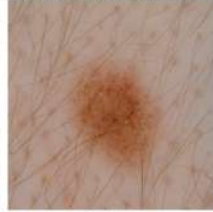

euclidean dice l1\_ISIC\_5476770

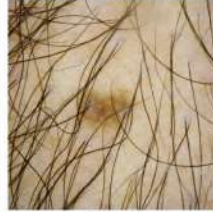

cosine dice l1\_ISIC\_4640621

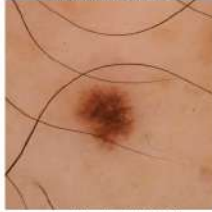

cosine dice l2\_ISIC\_7590008

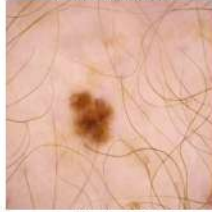

cosine dice l1\_ISIC\_9530032

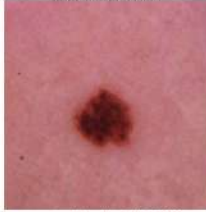

cosine dice l1\_ISIC\_0877919

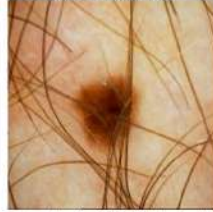

cosine dice l1\_ISIC\_1187477

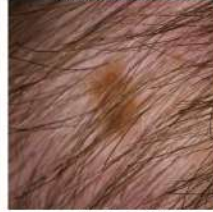

cosine euclidean dice l1\_ISIC\_1187477

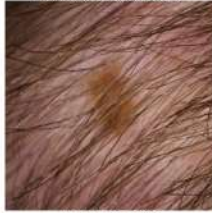

cosine euclidean dice l1\_ISIC\_9023820

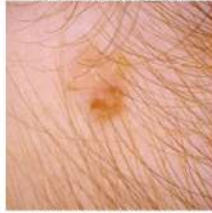

cosine euclidean dice l1\_ISIC\_0877919

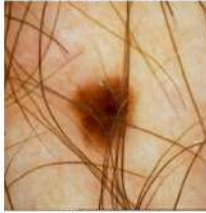

cosine euclidean dice l1\_ISIC\_0007157\_downsampled

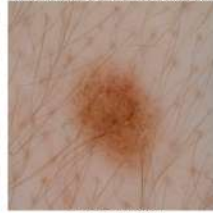

cosine euclidean dice l1\_ISIC\_5476770

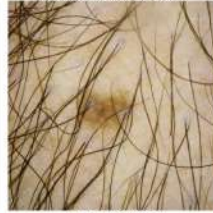

style dice l1\_ISIC\_4640621

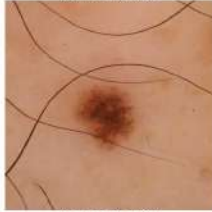

style dice l1\_ISIC\_0013222\_downsampled

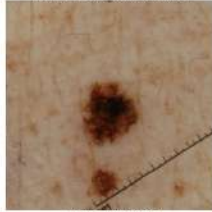

style dice l1\_ISIC\_7590008

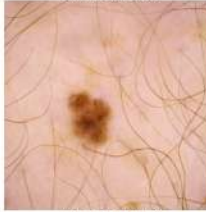

style dice l1\_ISIC\_0597581

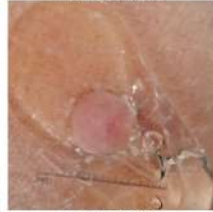

style dice l1\_ISIC\_0053749

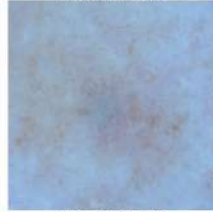

style euc l1\_ISIC\_4677073

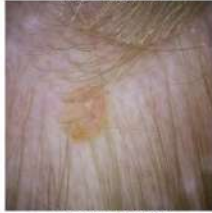

style euc l1\_ISIC\_9488995

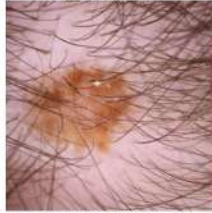

style euc l1\_ISIC\_5873539

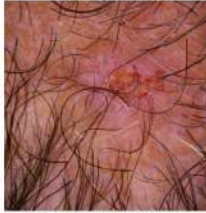

style euc l1\_ISIC\_6432615

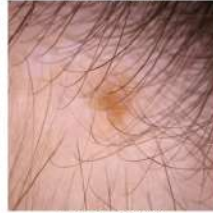

style euc l1\_ISIC\_0552421

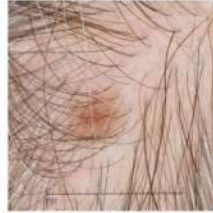

style cosine l1\_ISIC\_9488995

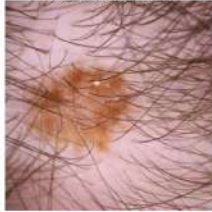

style cosine l1\_ISIC\_0012167\_downsampled

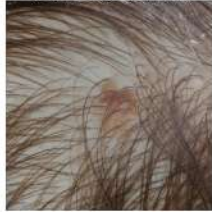

style cosine l1\_ISIC\_4677073

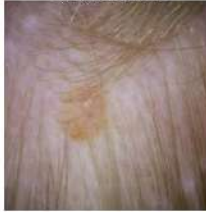

style cosine l1\_ISIC\_6694200

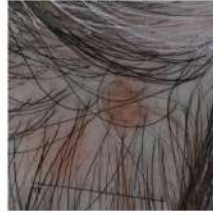

style cosine l1\_ISIC\_6432615

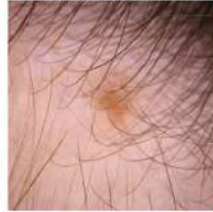

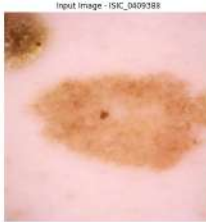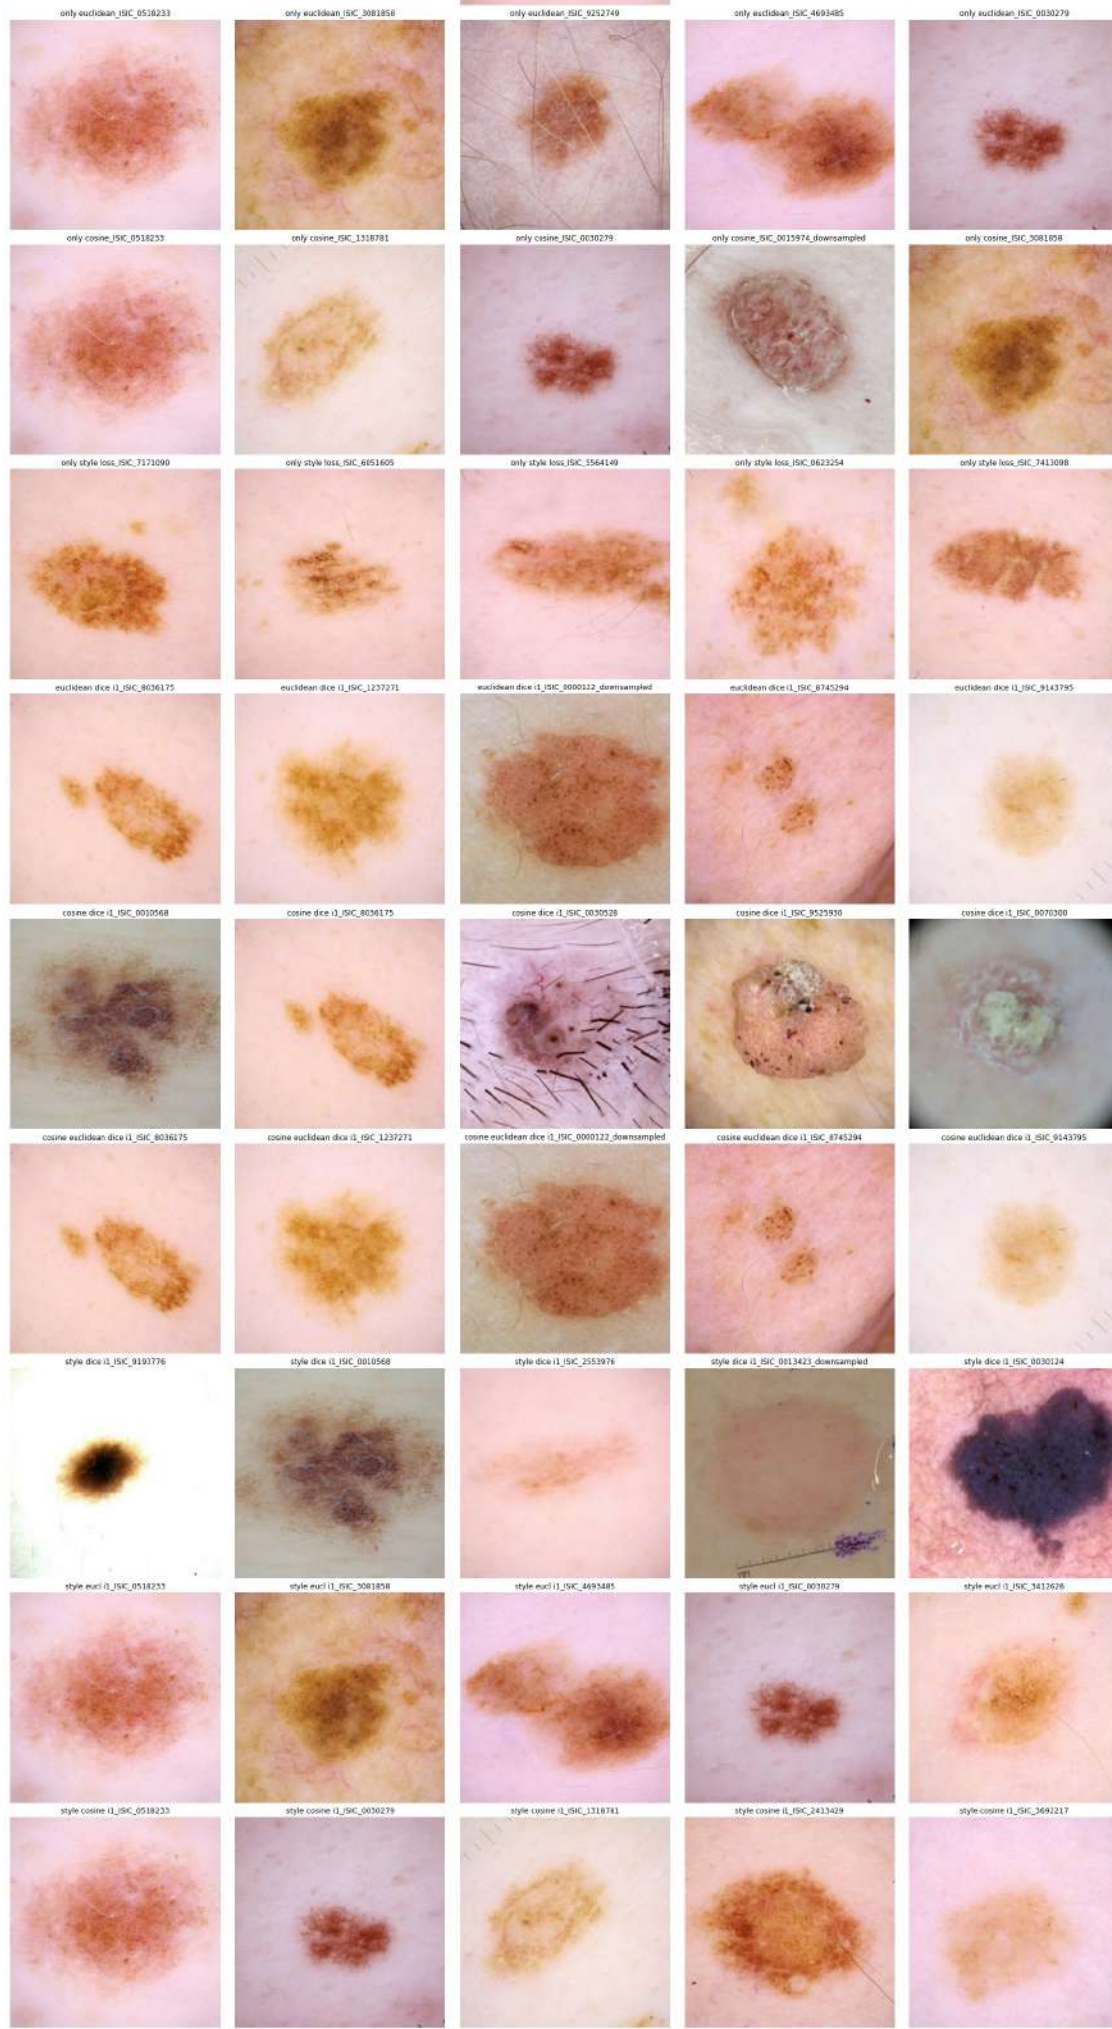

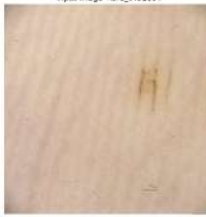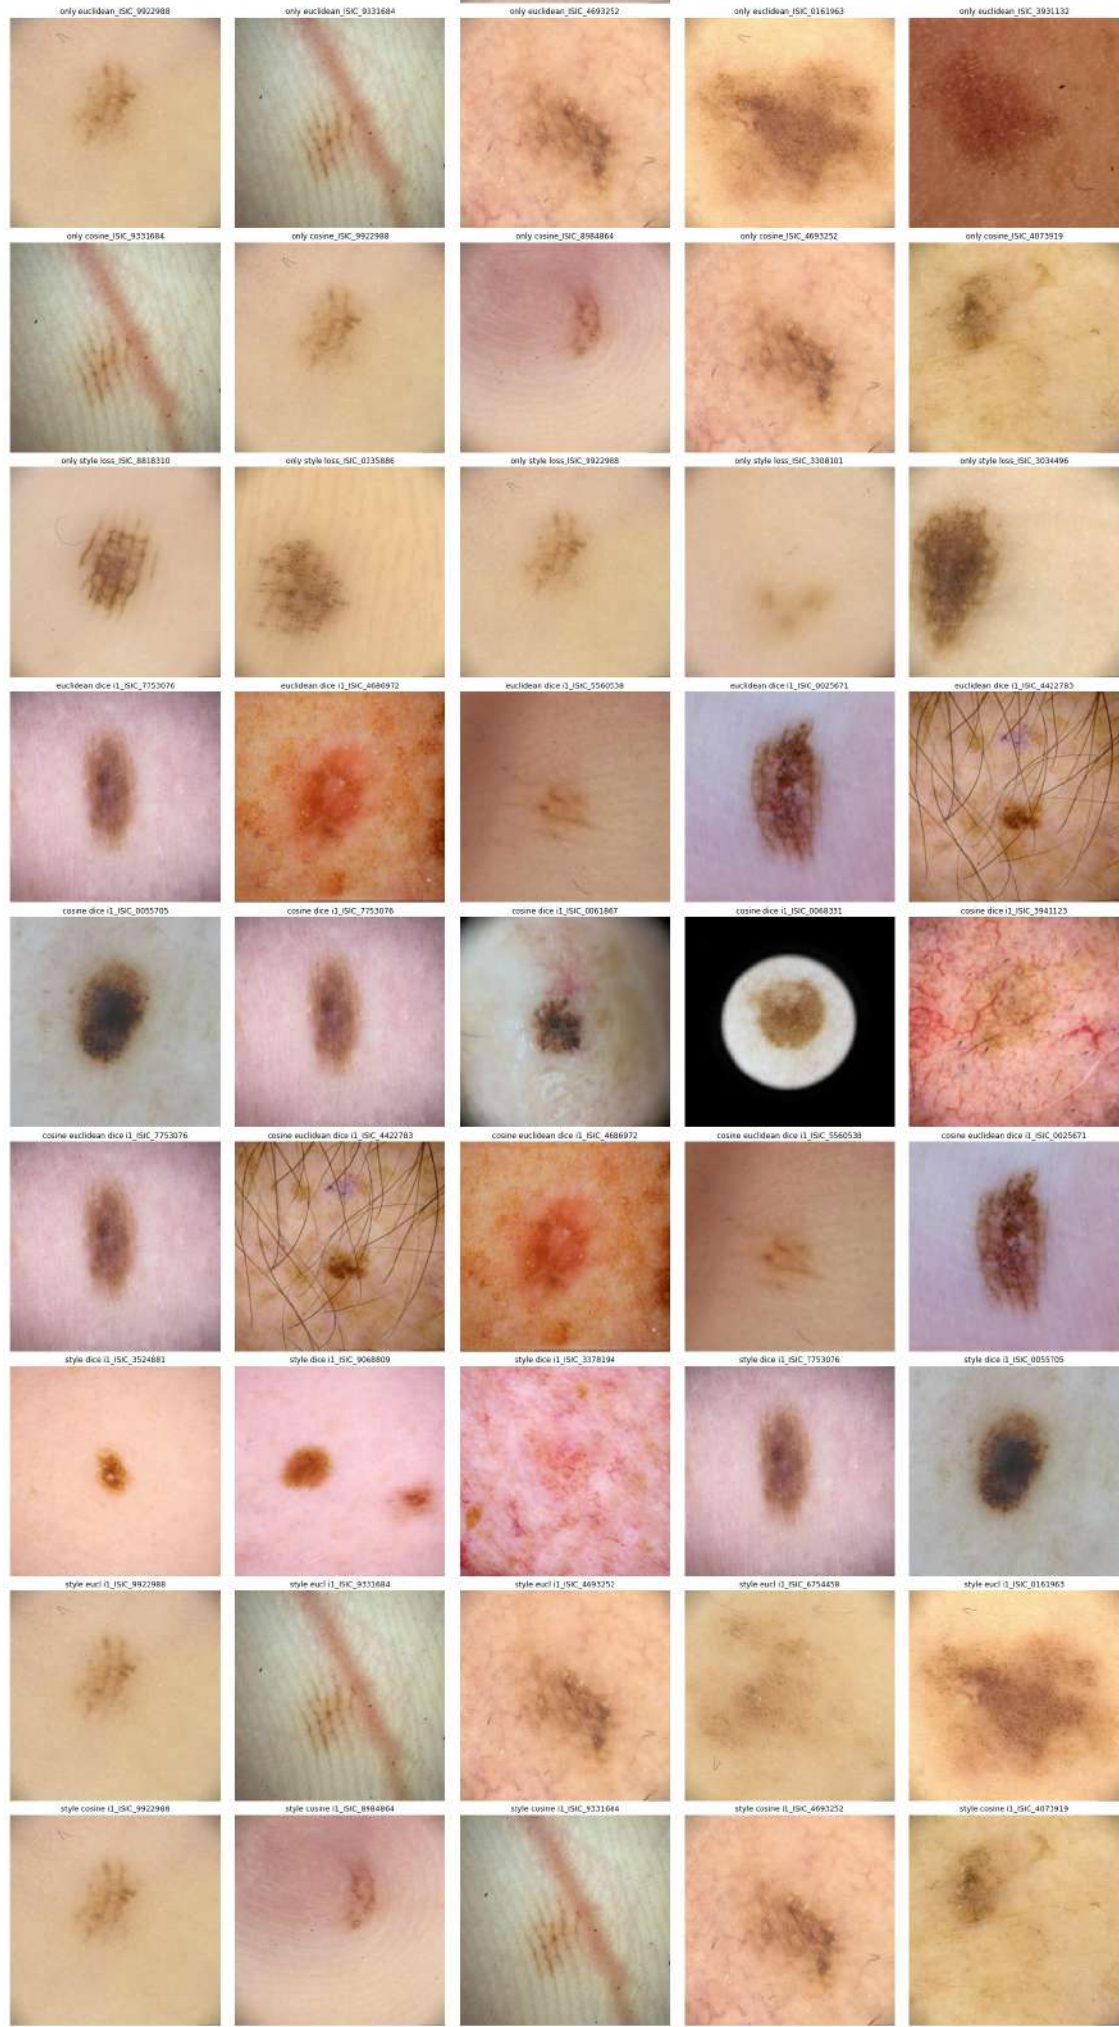

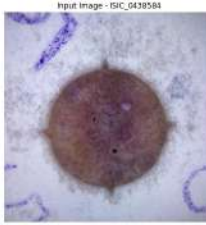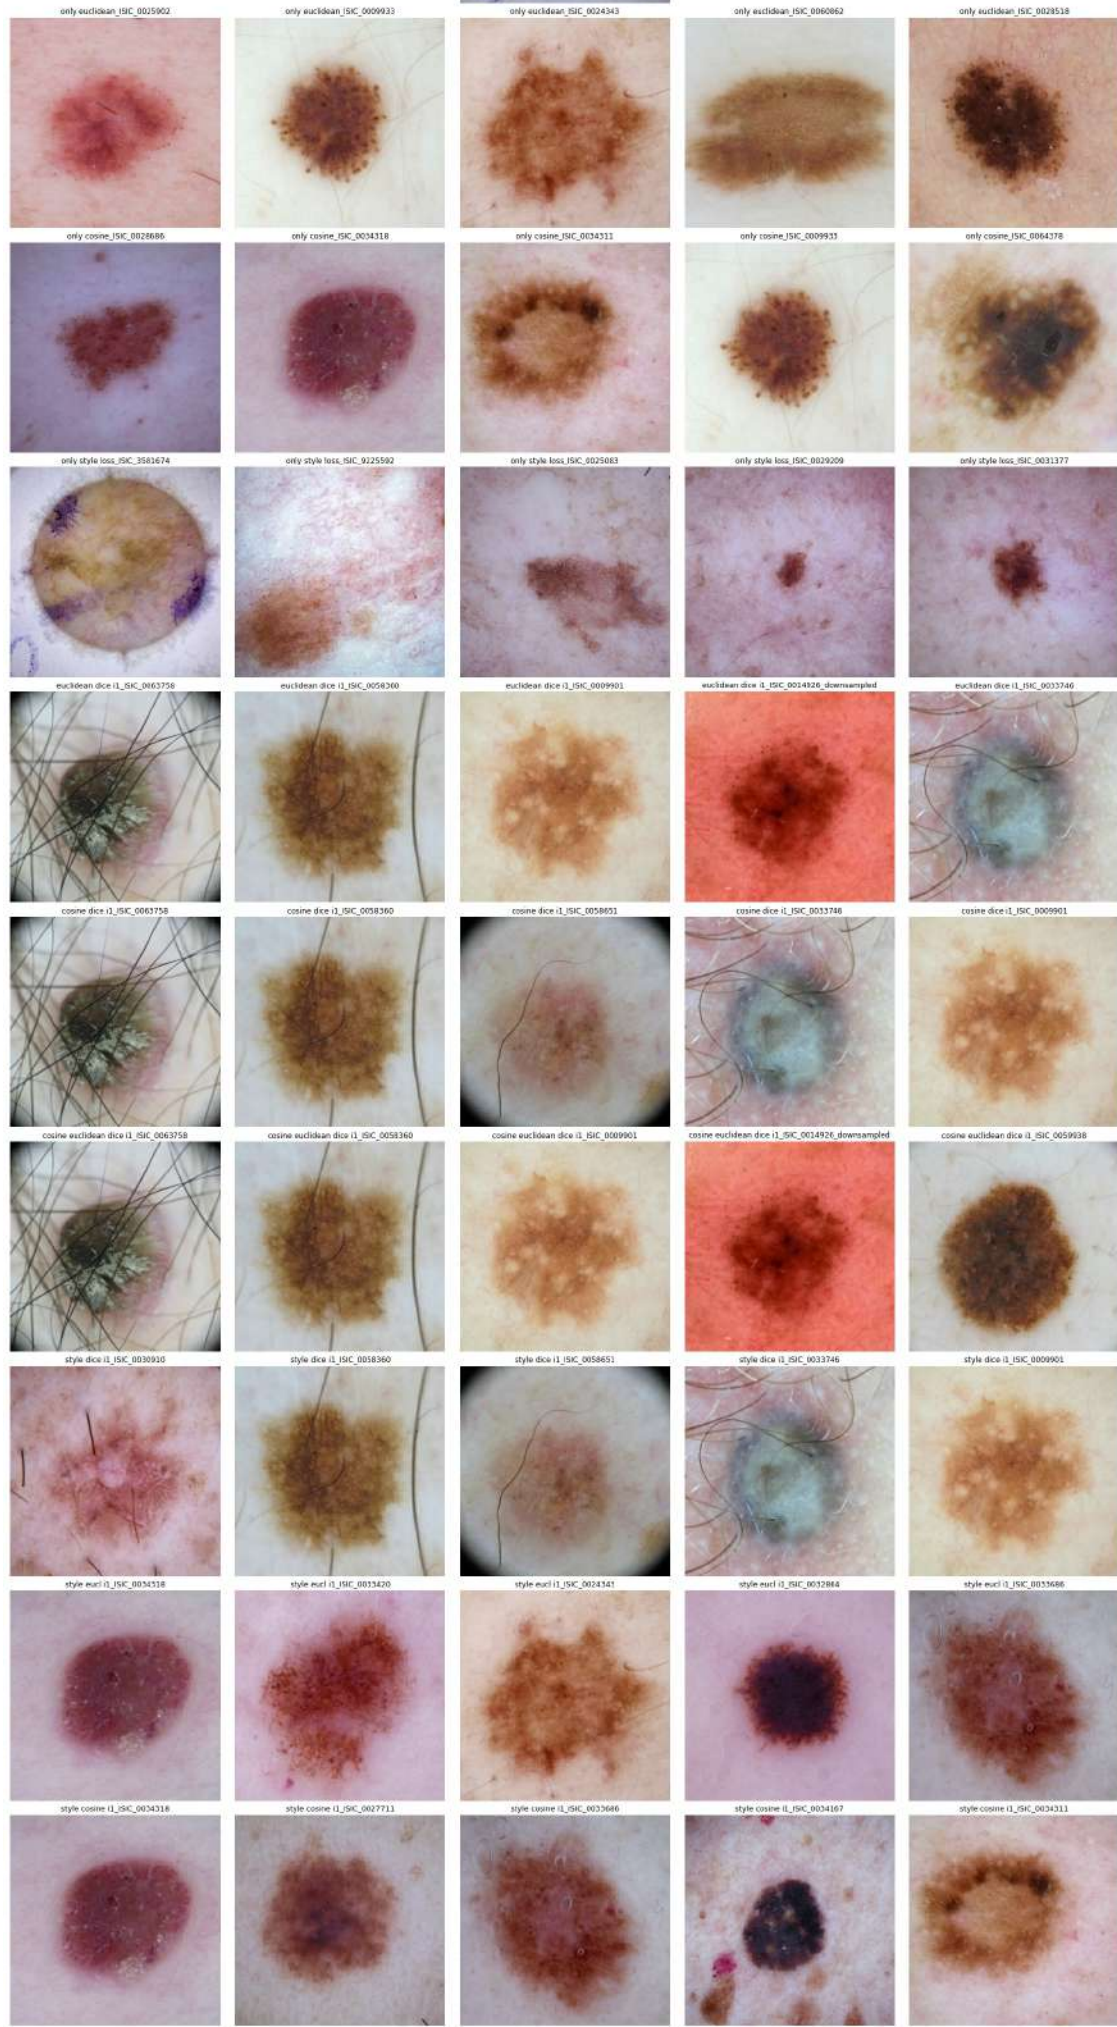



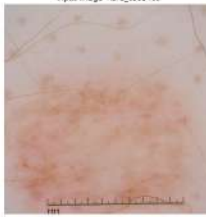

only euclidean\_ISIC\_7973564

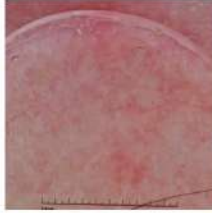

only euclidean\_ISIC\_2302286

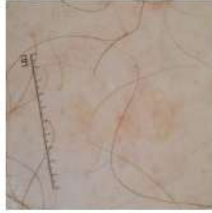

only euclidean\_ISIC\_1024617

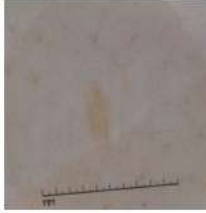

only euclidean\_ISIC\_9014045\_downsampled

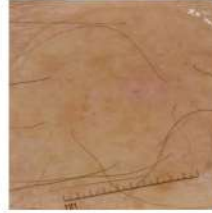

only euclidean\_ISIC\_3696570

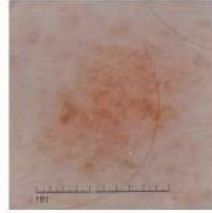

only cosine\_ISIC\_7973564

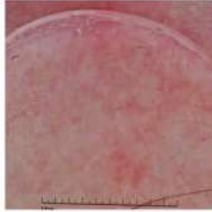

only cosine\_ISIC\_3696570

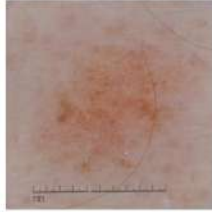

only cosine\_ISIC\_2302286

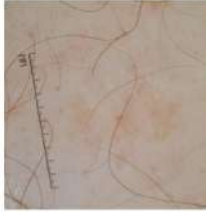

only cosine\_ISIC\_1817524

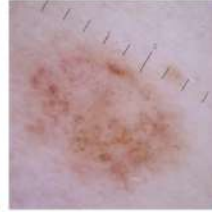

only cosine\_ISIC\_7681336

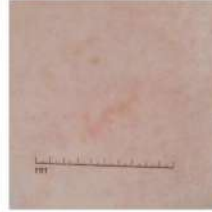

only style loss\_ISIC\_2310322

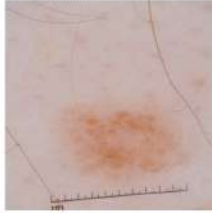

only style loss\_ISIC\_4134016

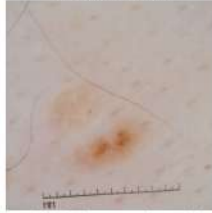

only style loss\_ISIC\_5962462

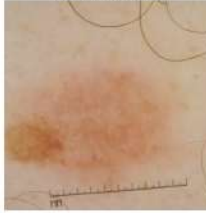

only style loss\_ISIC\_9012358\_downsampled

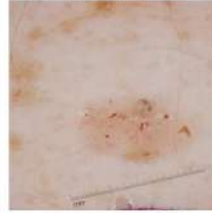

only style loss\_ISIC\_4441776

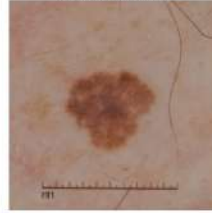

euclidean dice l1\_ISIC\_0029217

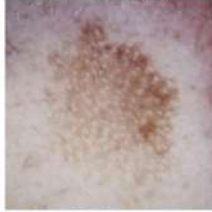

euclidean dice l1\_ISIC\_000473\_downsampled

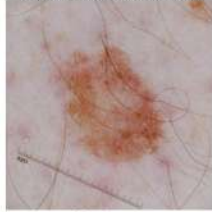

euclidean dice l1\_ISIC\_0071979

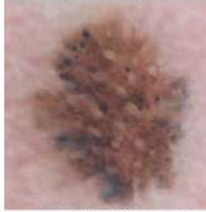

euclidean dice l1\_ISIC\_0061175

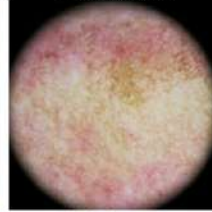

euclidean dice l1\_ISIC\_0593756

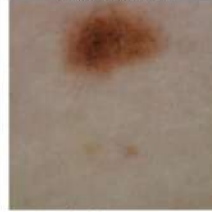

cosine dice l1\_ISIC\_0029217

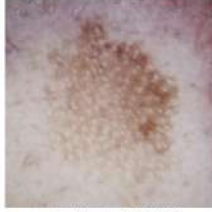

cosine dice l1\_ISIC\_0071979

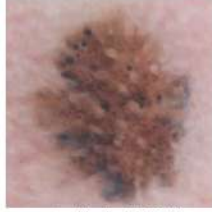

cosine dice l1\_ISIC\_000473\_downsampled

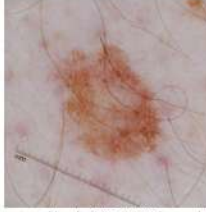

cosine dice l1\_ISIC\_0593756

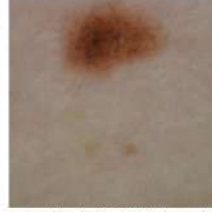

cosine dice l1\_ISIC\_0053753

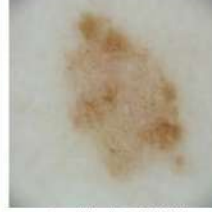

cosine euclidean dice l1\_ISIC\_0029217

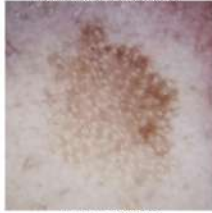

cosine euclidean dice l1\_ISIC\_0061175

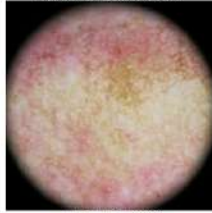

cosine euclidean dice l1\_ISIC\_000473\_downsampled

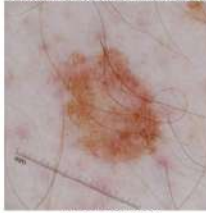

cosine euclidean dice l1\_ISIC\_003765\_downsampled

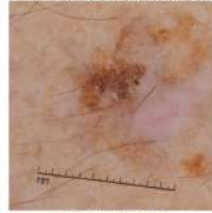

cosine euclidean dice l1\_ISIC\_0071979

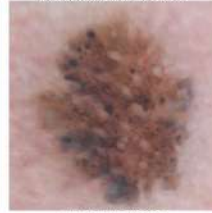

style dice l1\_ISIC\_0096328

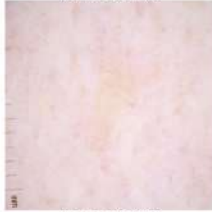

style dice l1\_ISIC\_0071979

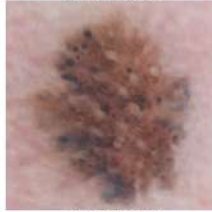

style dice l1\_ISIC\_4198680

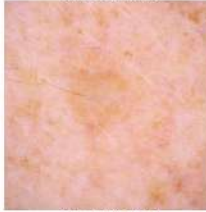

style dice l1\_ISIC\_6060655

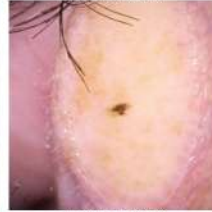

style dice l1\_ISIC\_0593756

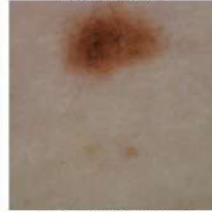

style eucl l1\_ISIC\_2302286

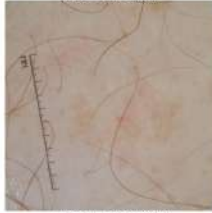

style eucl l1\_ISIC\_3696570

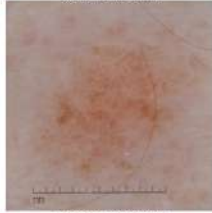

style eucl l1\_ISIC\_7973564

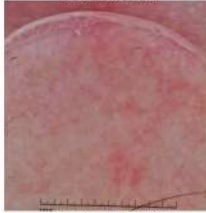

style eucl l1\_ISIC\_1024617

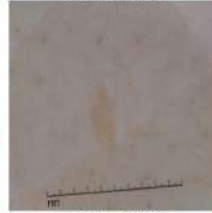

style eucl l1\_ISIC\_9014045\_downsampled

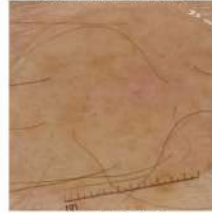

style cosine l1\_ISIC\_3696570

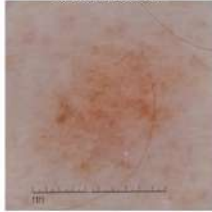

style cosine l1\_ISIC\_7973564

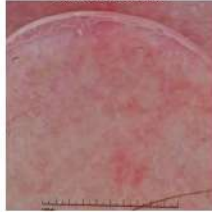

style cosine l1\_ISIC\_2302286

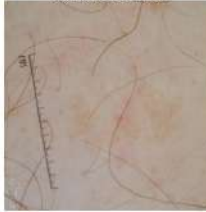

style cosine l1\_ISIC\_5923285

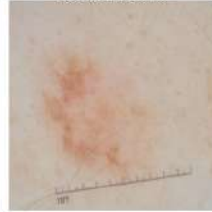

style cosine l1\_ISIC\_7681336

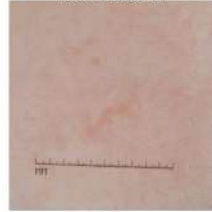

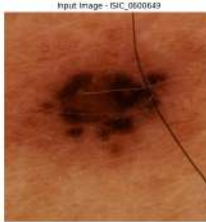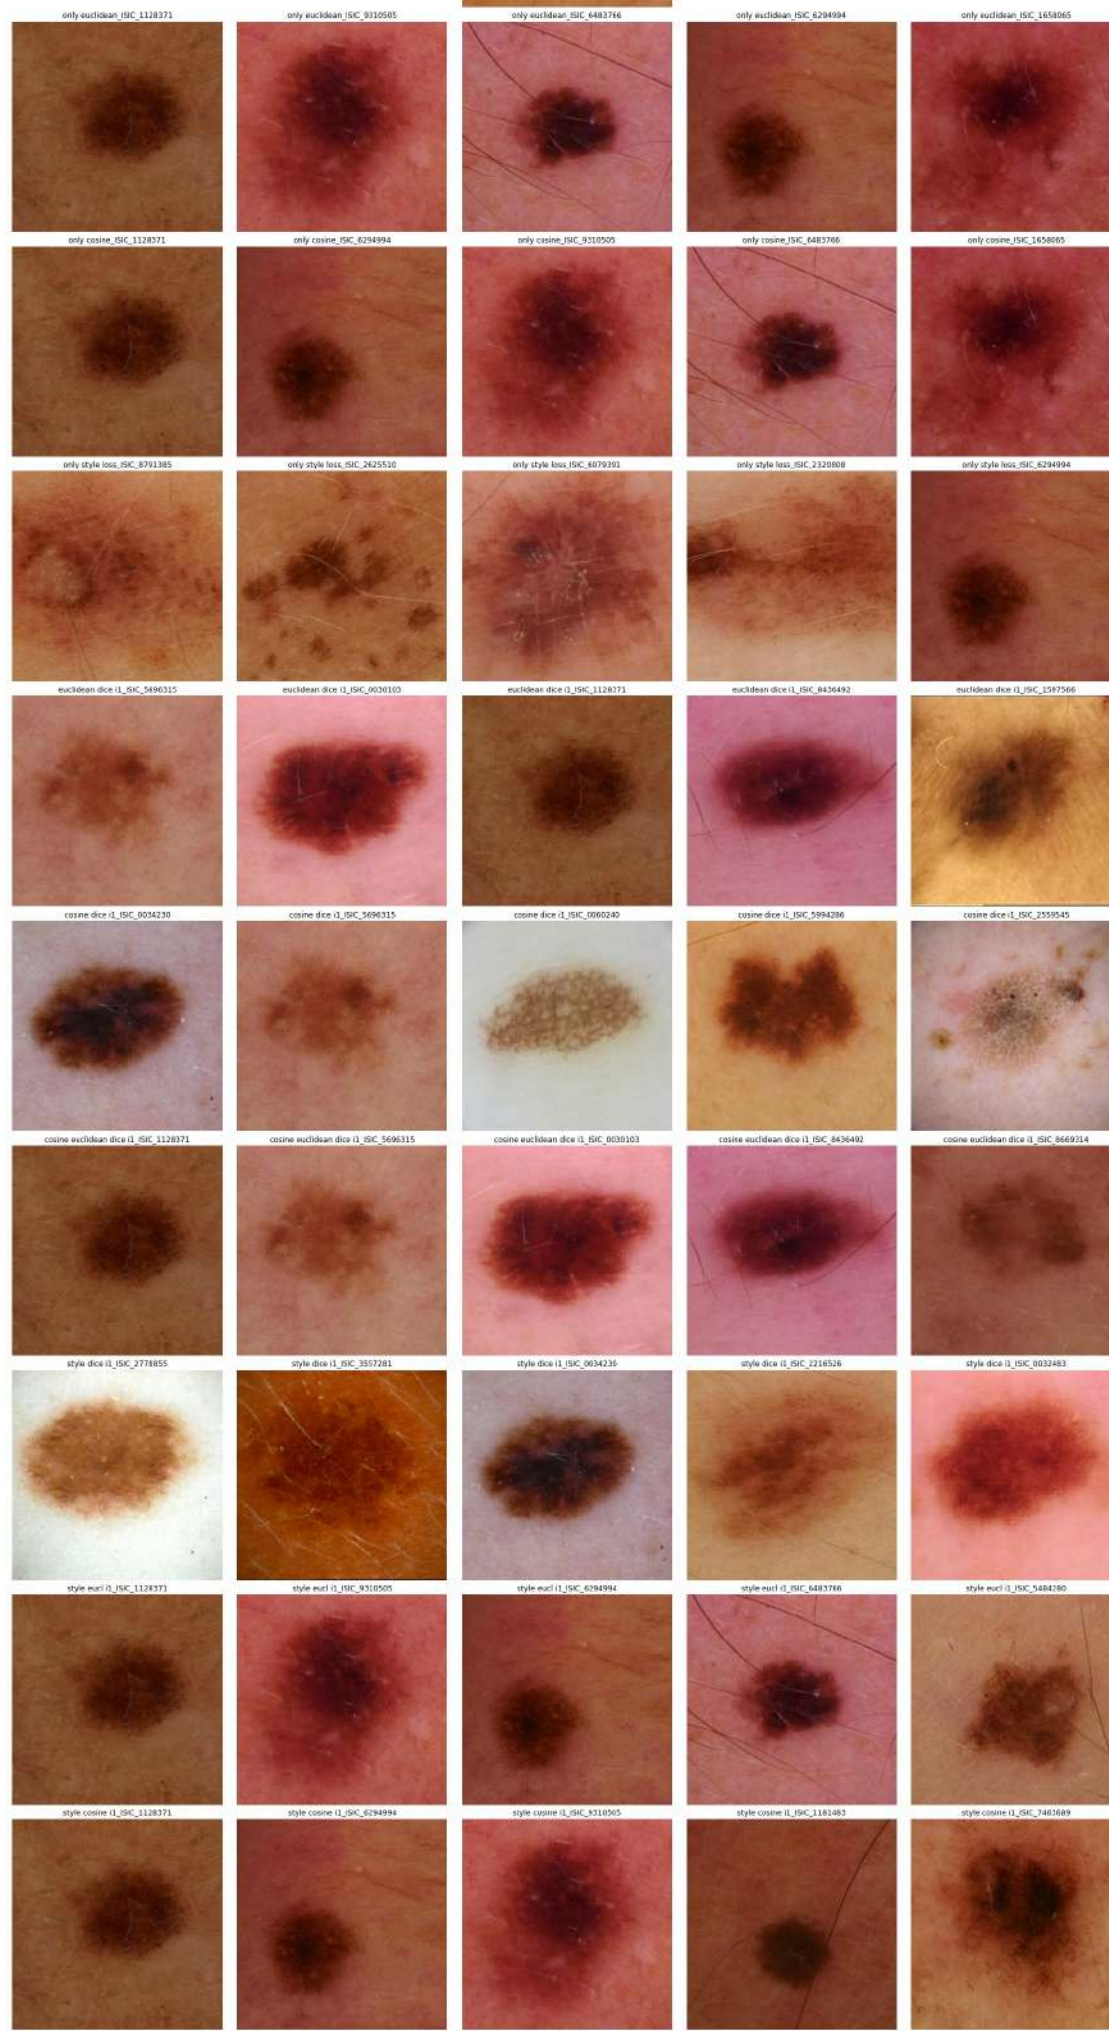

Input image - ISIC\_0034896

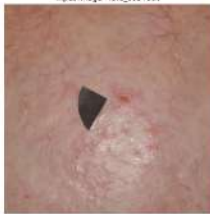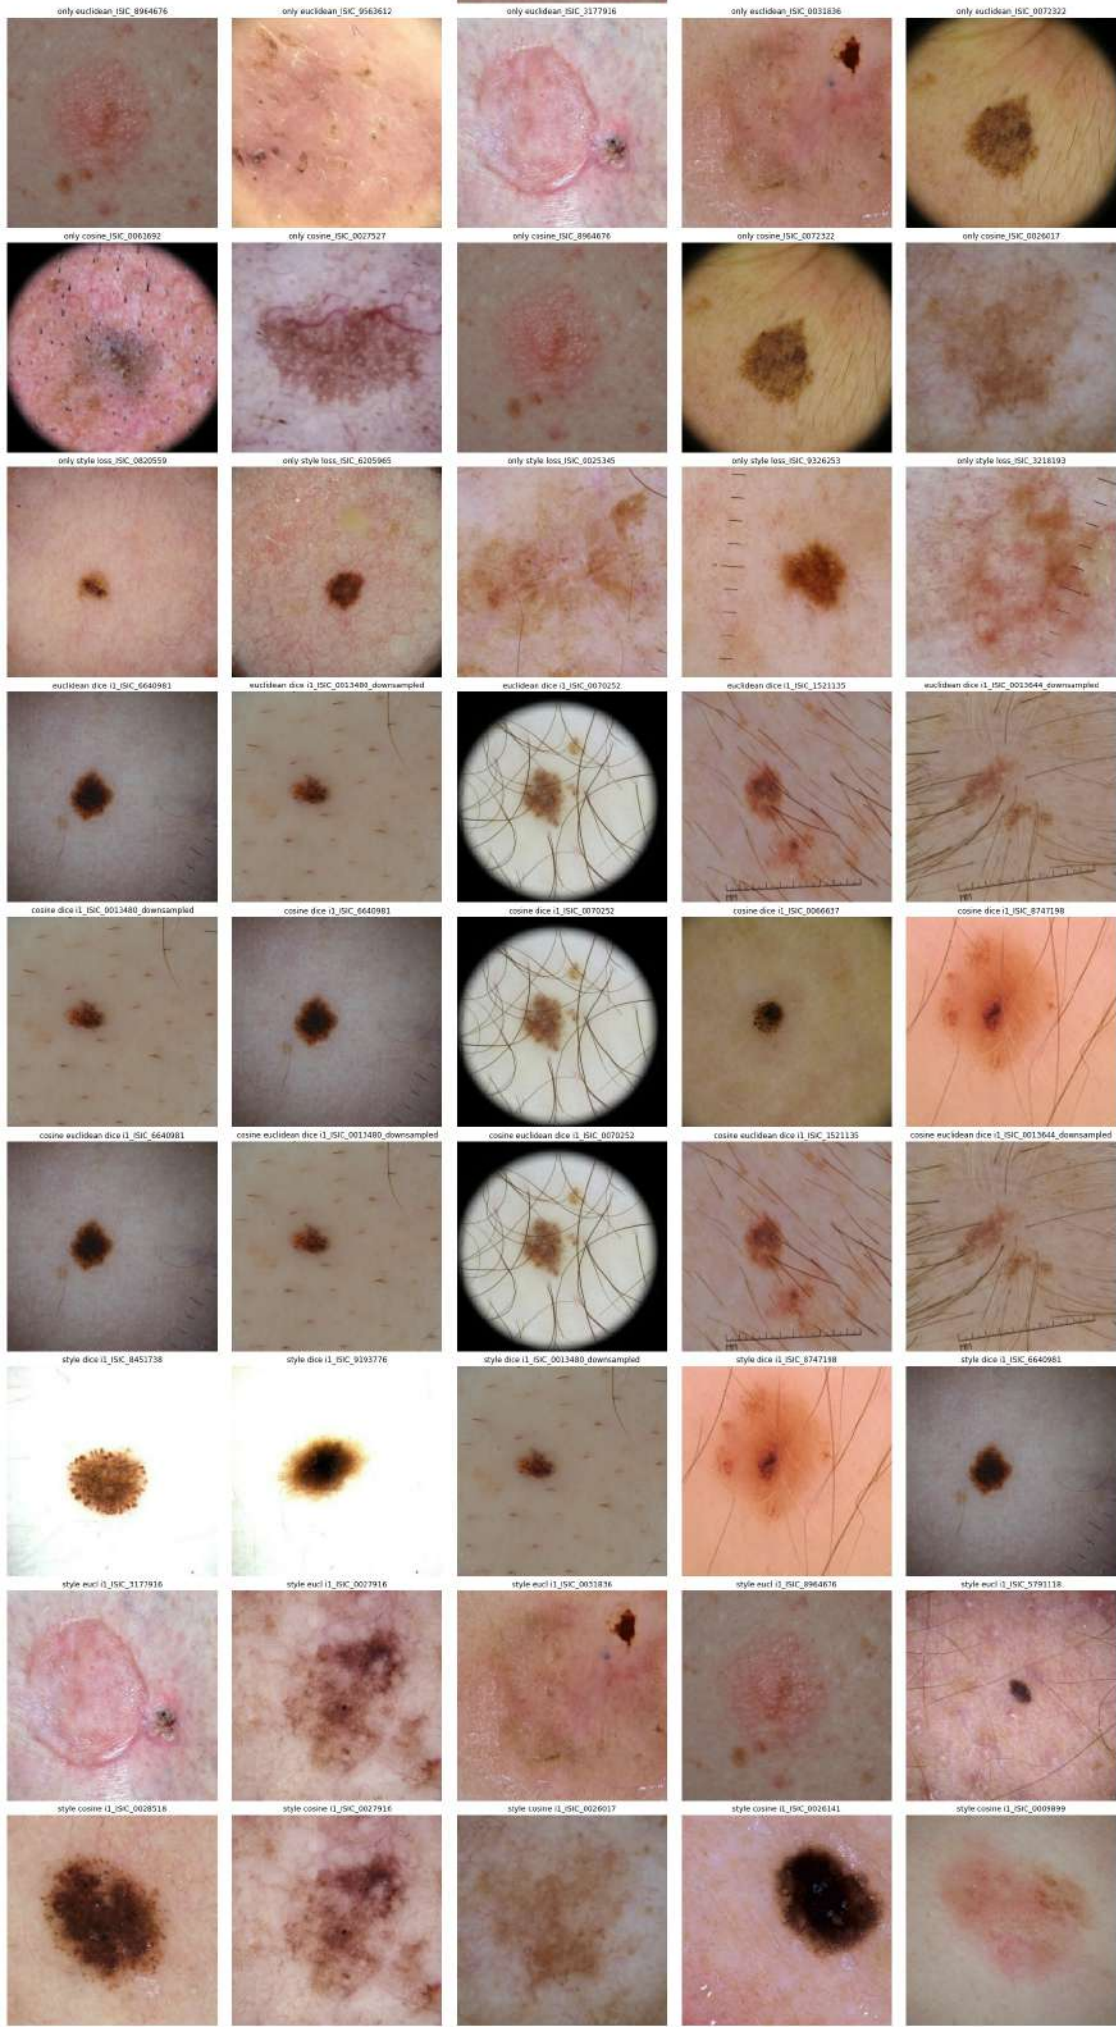

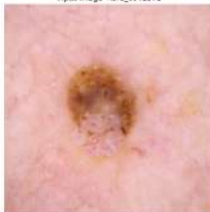

only euclidean\_JSC\_1627019      only euclidean\_JSC\_8669986      only euclidean\_JSC\_3327261      only euclidean\_JSC\_4312841      only euclidean\_JSC\_0060280

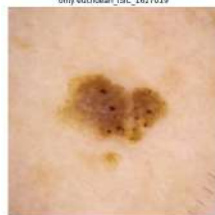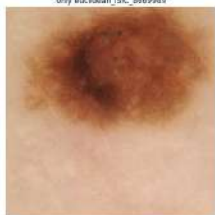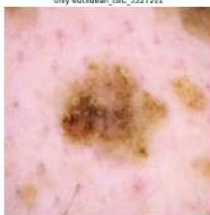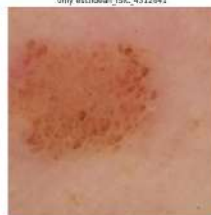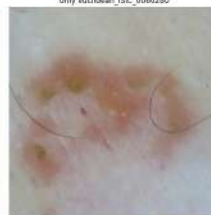

only cosine\_JSC\_3603916      only cosine\_JSC\_0026496      only cosine\_JSC\_1627019      only cosine\_JSC\_0029827      only cosine\_JSC\_0060280

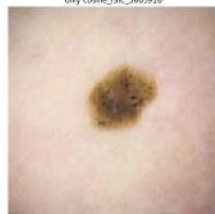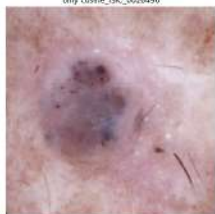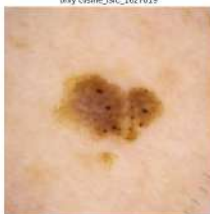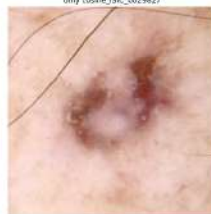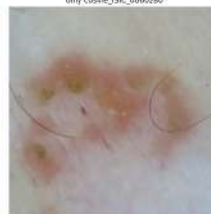

only style loss\_JSC\_0609067      only style loss\_JSC\_1880253      only style loss\_JSC\_3784838      only style loss\_JSC\_6780001      only style loss\_JSC\_0036311

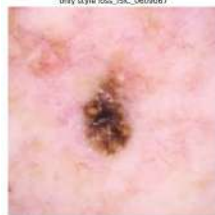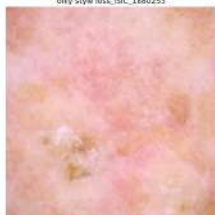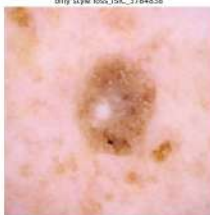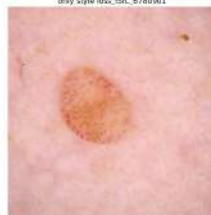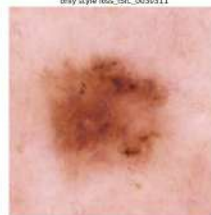

euclidean dice l1\_JSC\_9322705      euclidean dice l1\_JSC\_0033375      euclidean dice l1\_JSC\_1035480      euclidean dice l1\_JSC\_8339176      euclidean dice l1\_JSC\_0061676

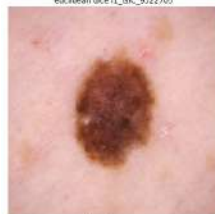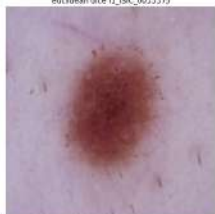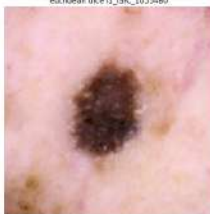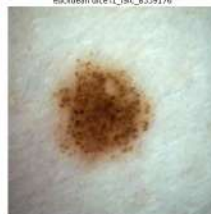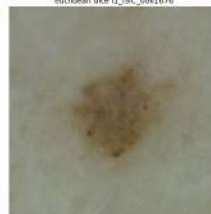

cosine dice l1\_JSC\_9322705      cosine dice l1\_JSC\_0033375      cosine dice l1\_JSC\_0069439      cosine dice l1\_JSC\_1035480      cosine dice l1\_JSC\_0065279

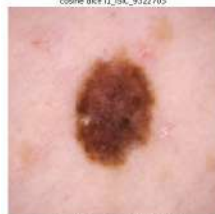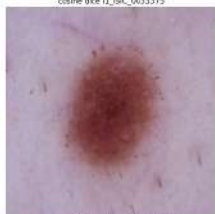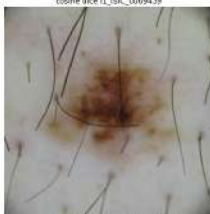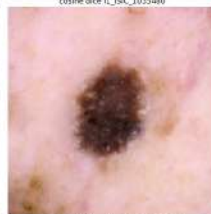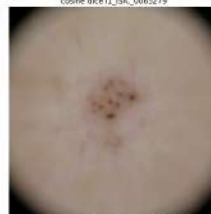

cosine euclidean dice l1\_JSC\_9322705      cosine euclidean dice l1\_JSC\_8339176      cosine euclidean dice l1\_JSC\_0033375      cosine euclidean dice l1\_JSC\_0061676      cosine euclidean dice l1\_JSC\_0054116

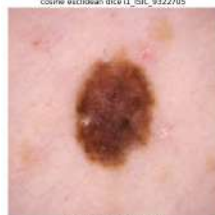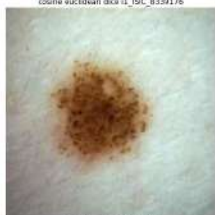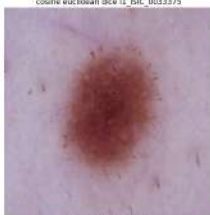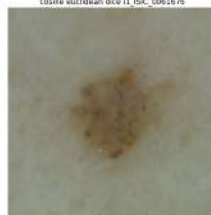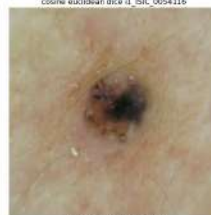

style dice l1\_JSC\_3472455      style dice l1\_JSC\_0077735      style dice l1\_JSC\_9322705      style dice l1\_JSC\_0028056      style dice l1\_JSC\_4637479

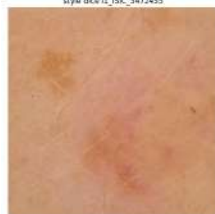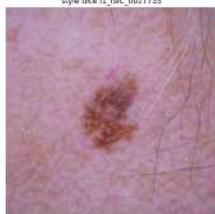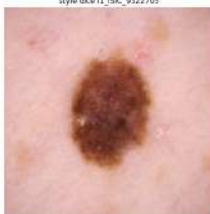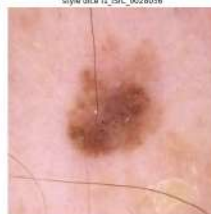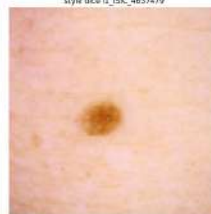

style eucl l1\_JSC\_1627019      style eucl l1\_JSC\_3327201      style eucl l1\_JSC\_8669986      style eucl l1\_JSC\_4312841      style eucl l1\_JSC\_5137911

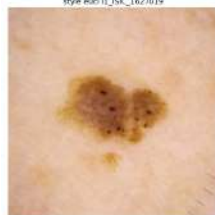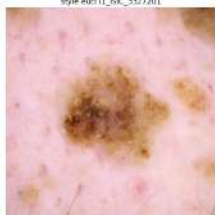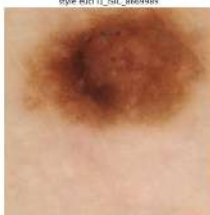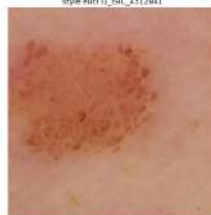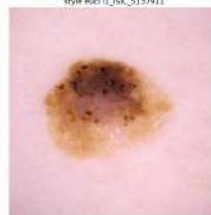

style cosine l1\_JSC\_3327201      style cosine l1\_JSC\_3427019      style cosine l1\_JSC\_0026496      style cosine l1\_JSC\_0031181      style cosine l1\_JSC\_0024569

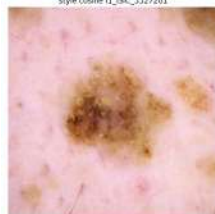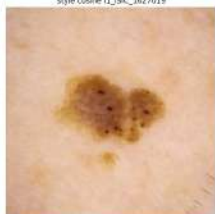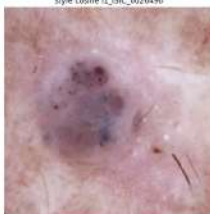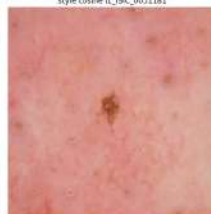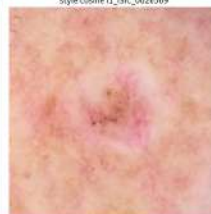

Input image - ISIC\_0746818

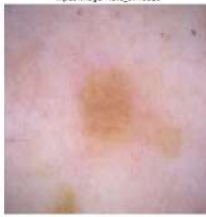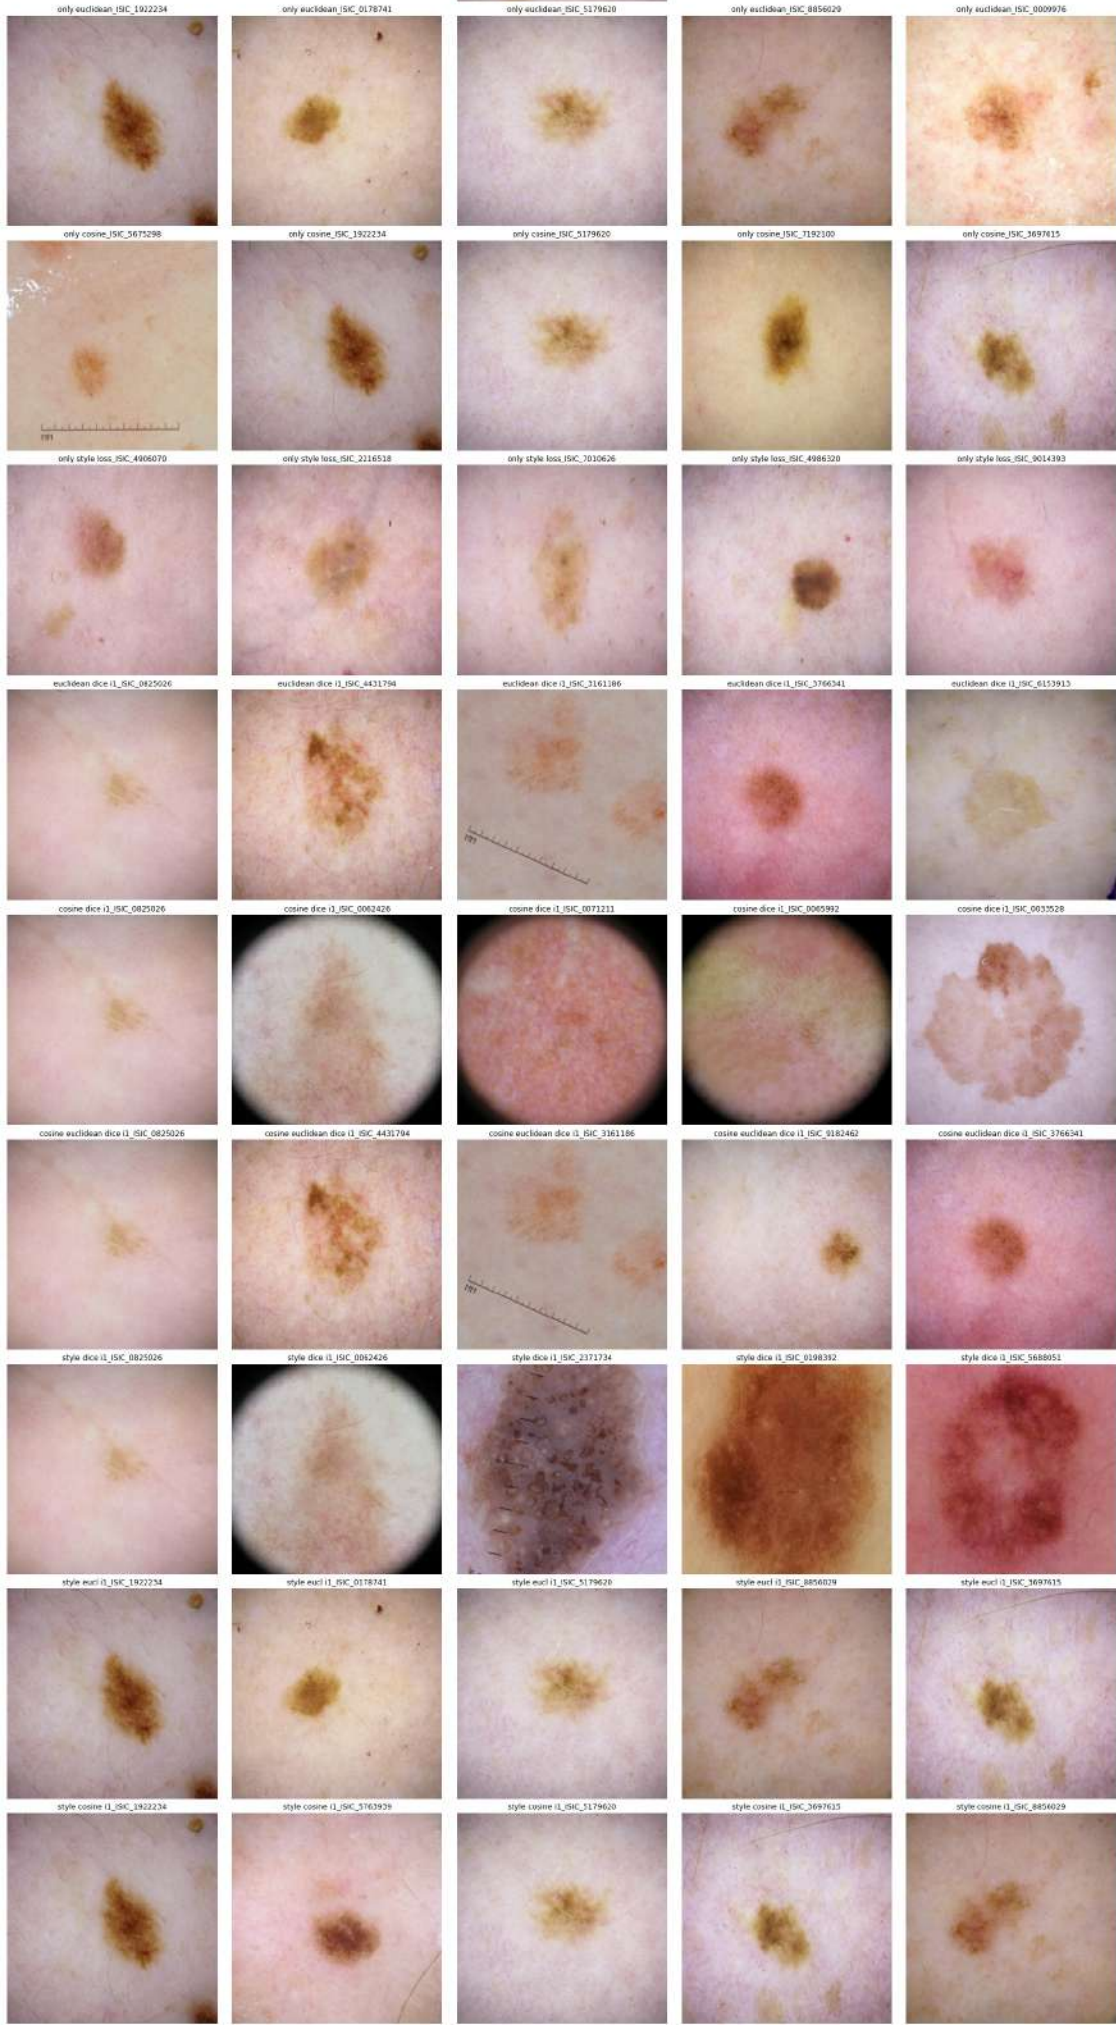

Input image - ISIC\_0758568

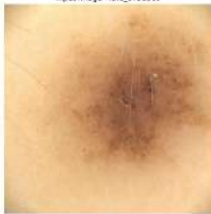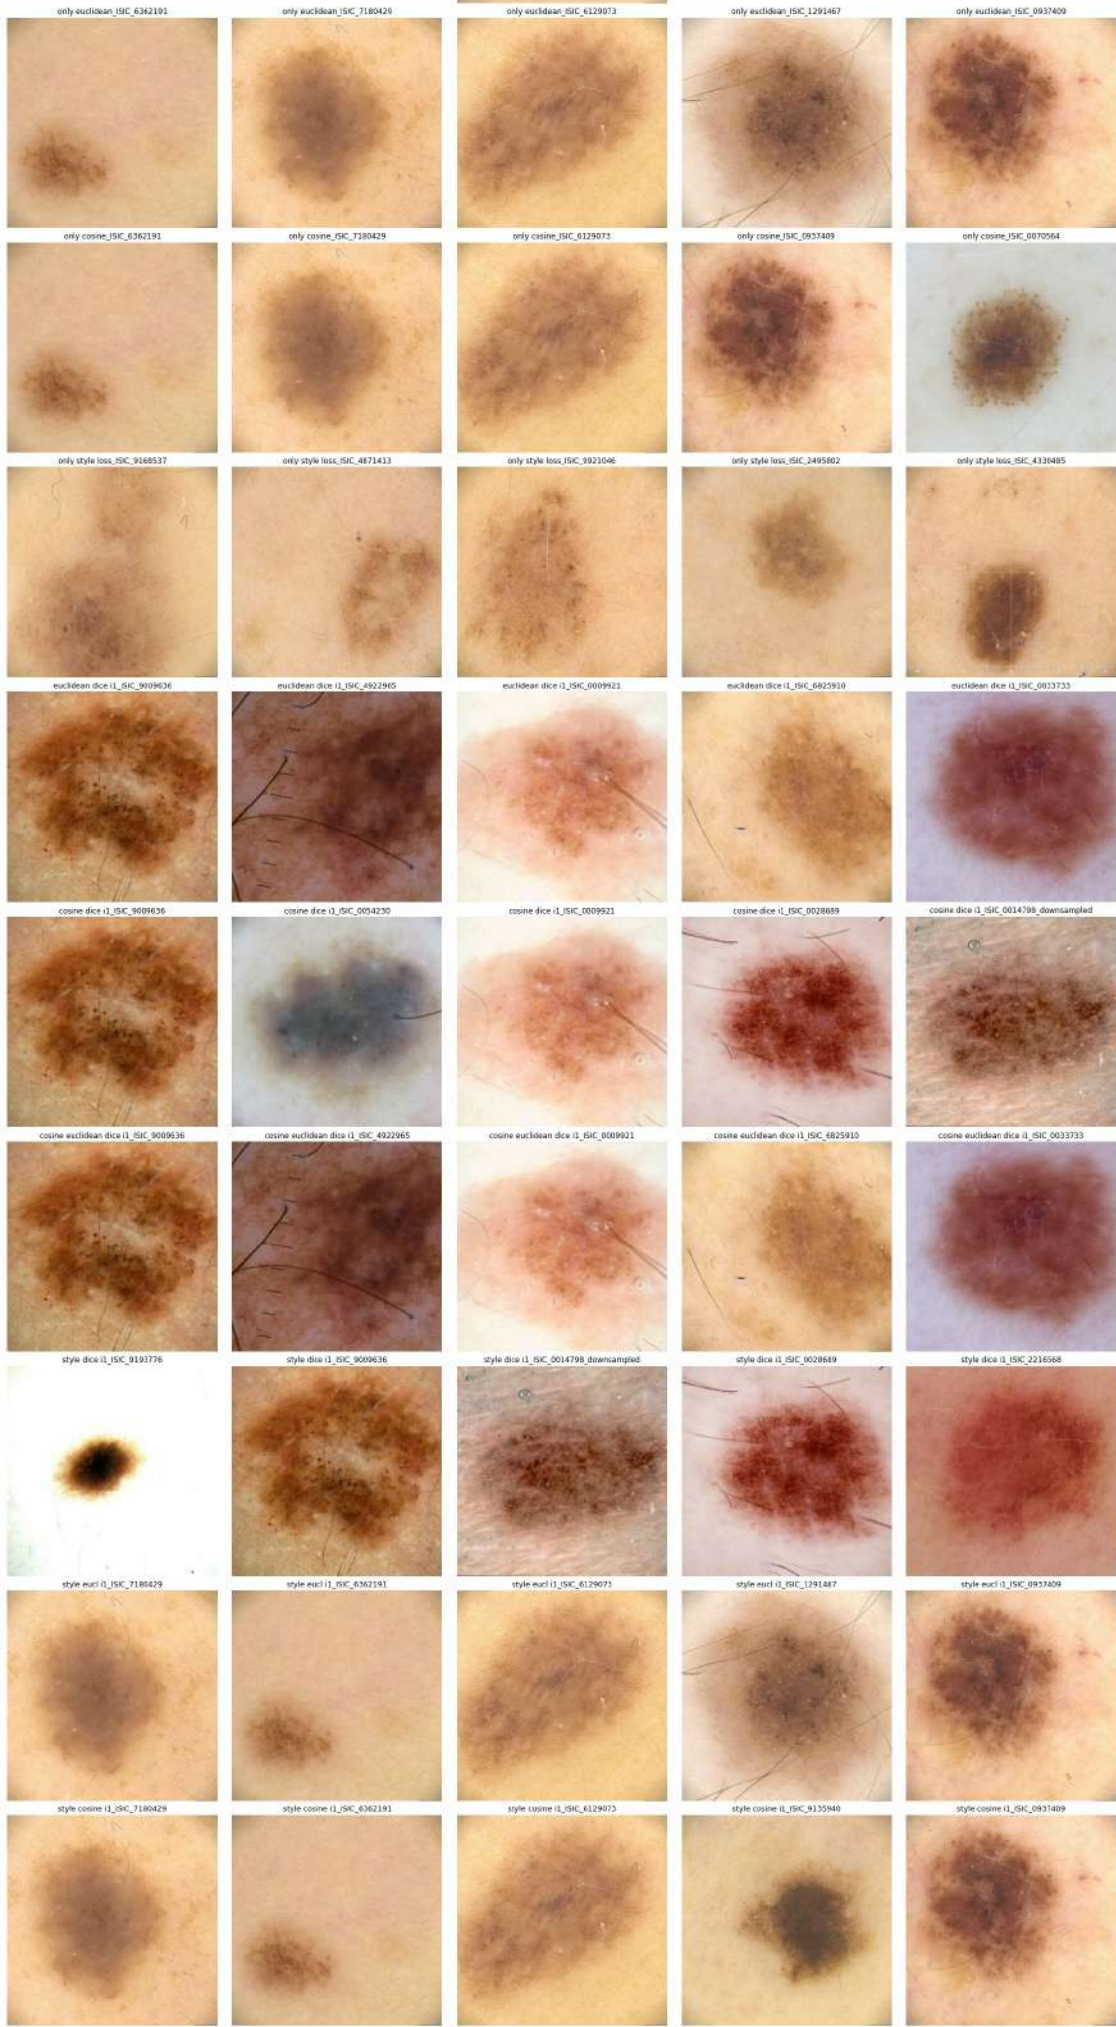

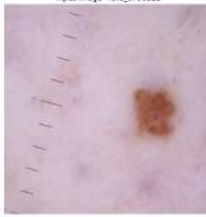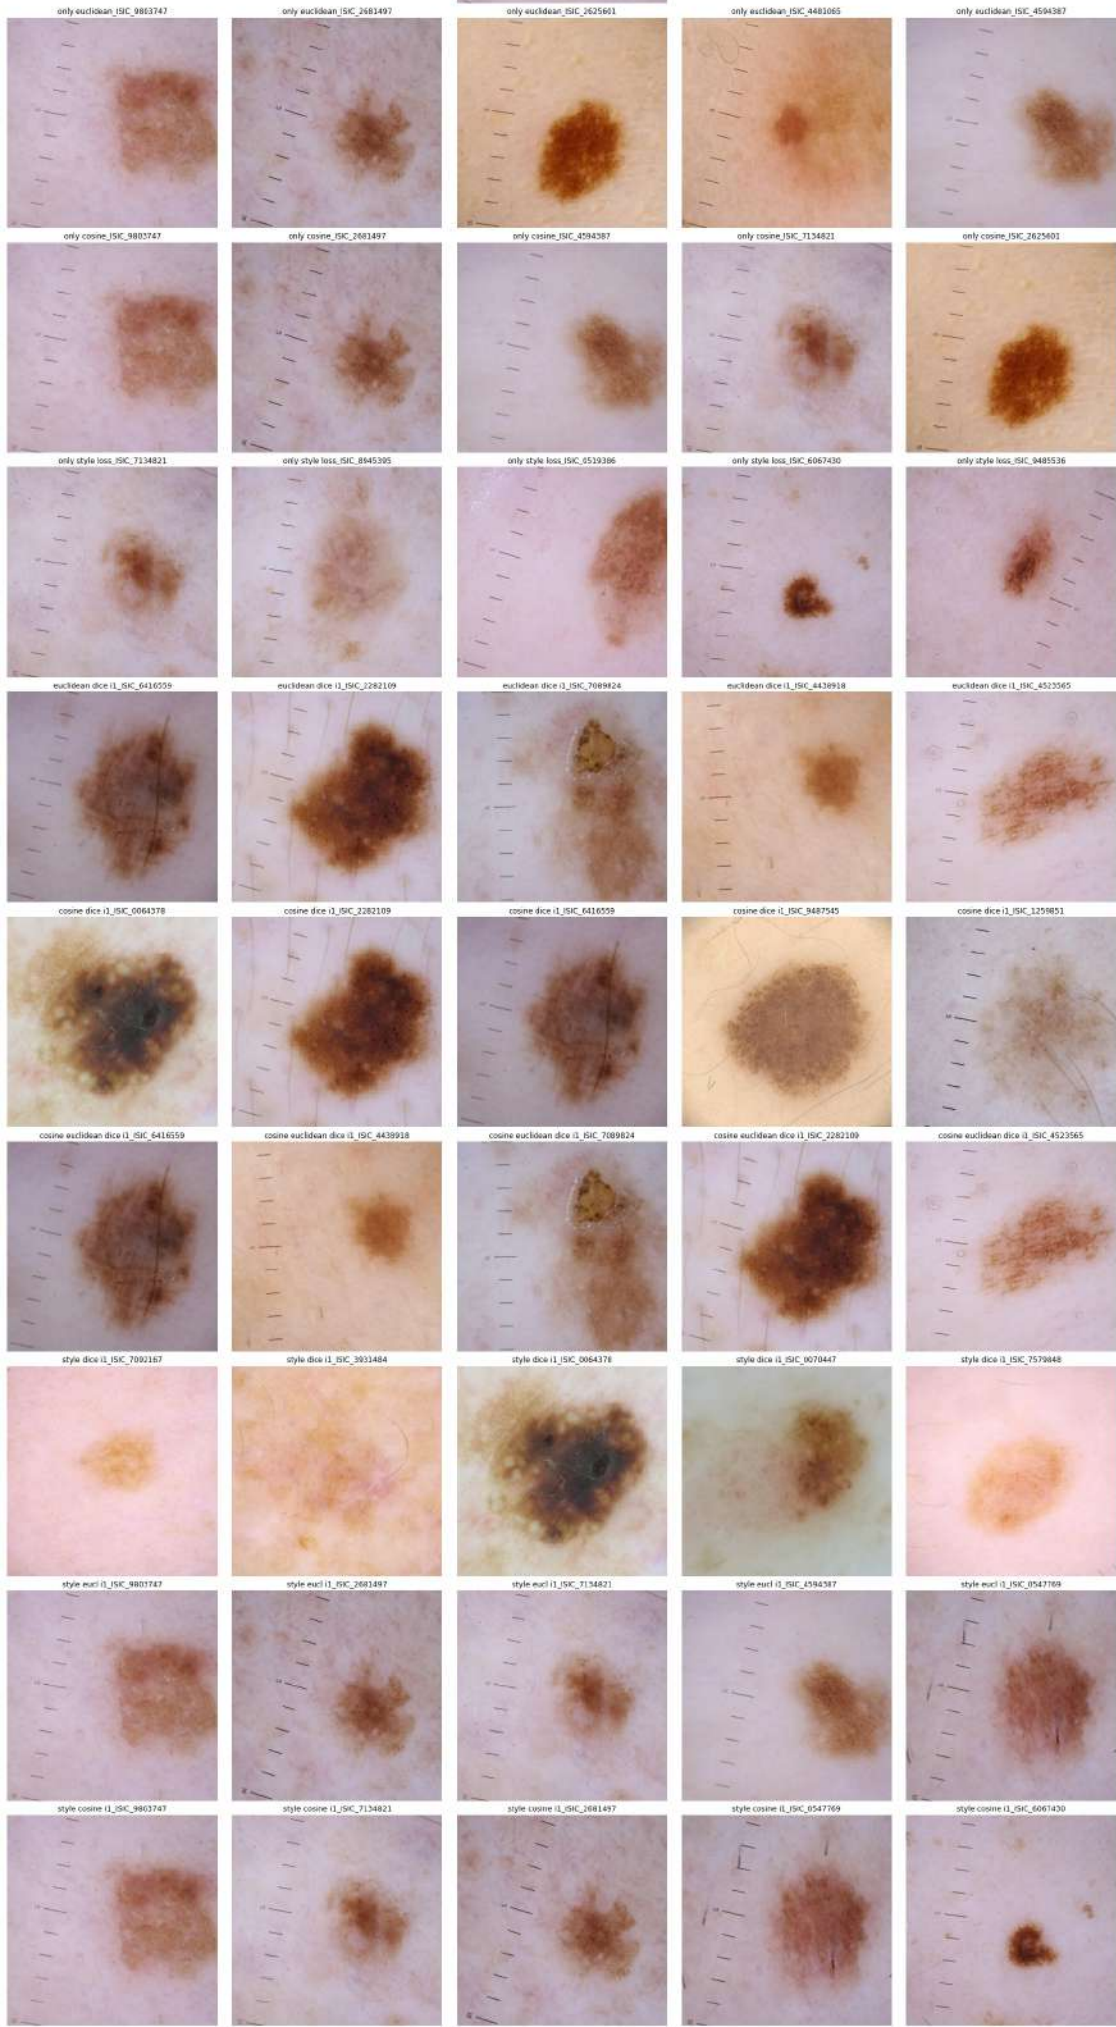

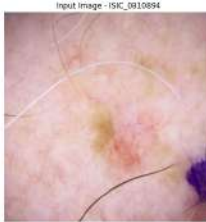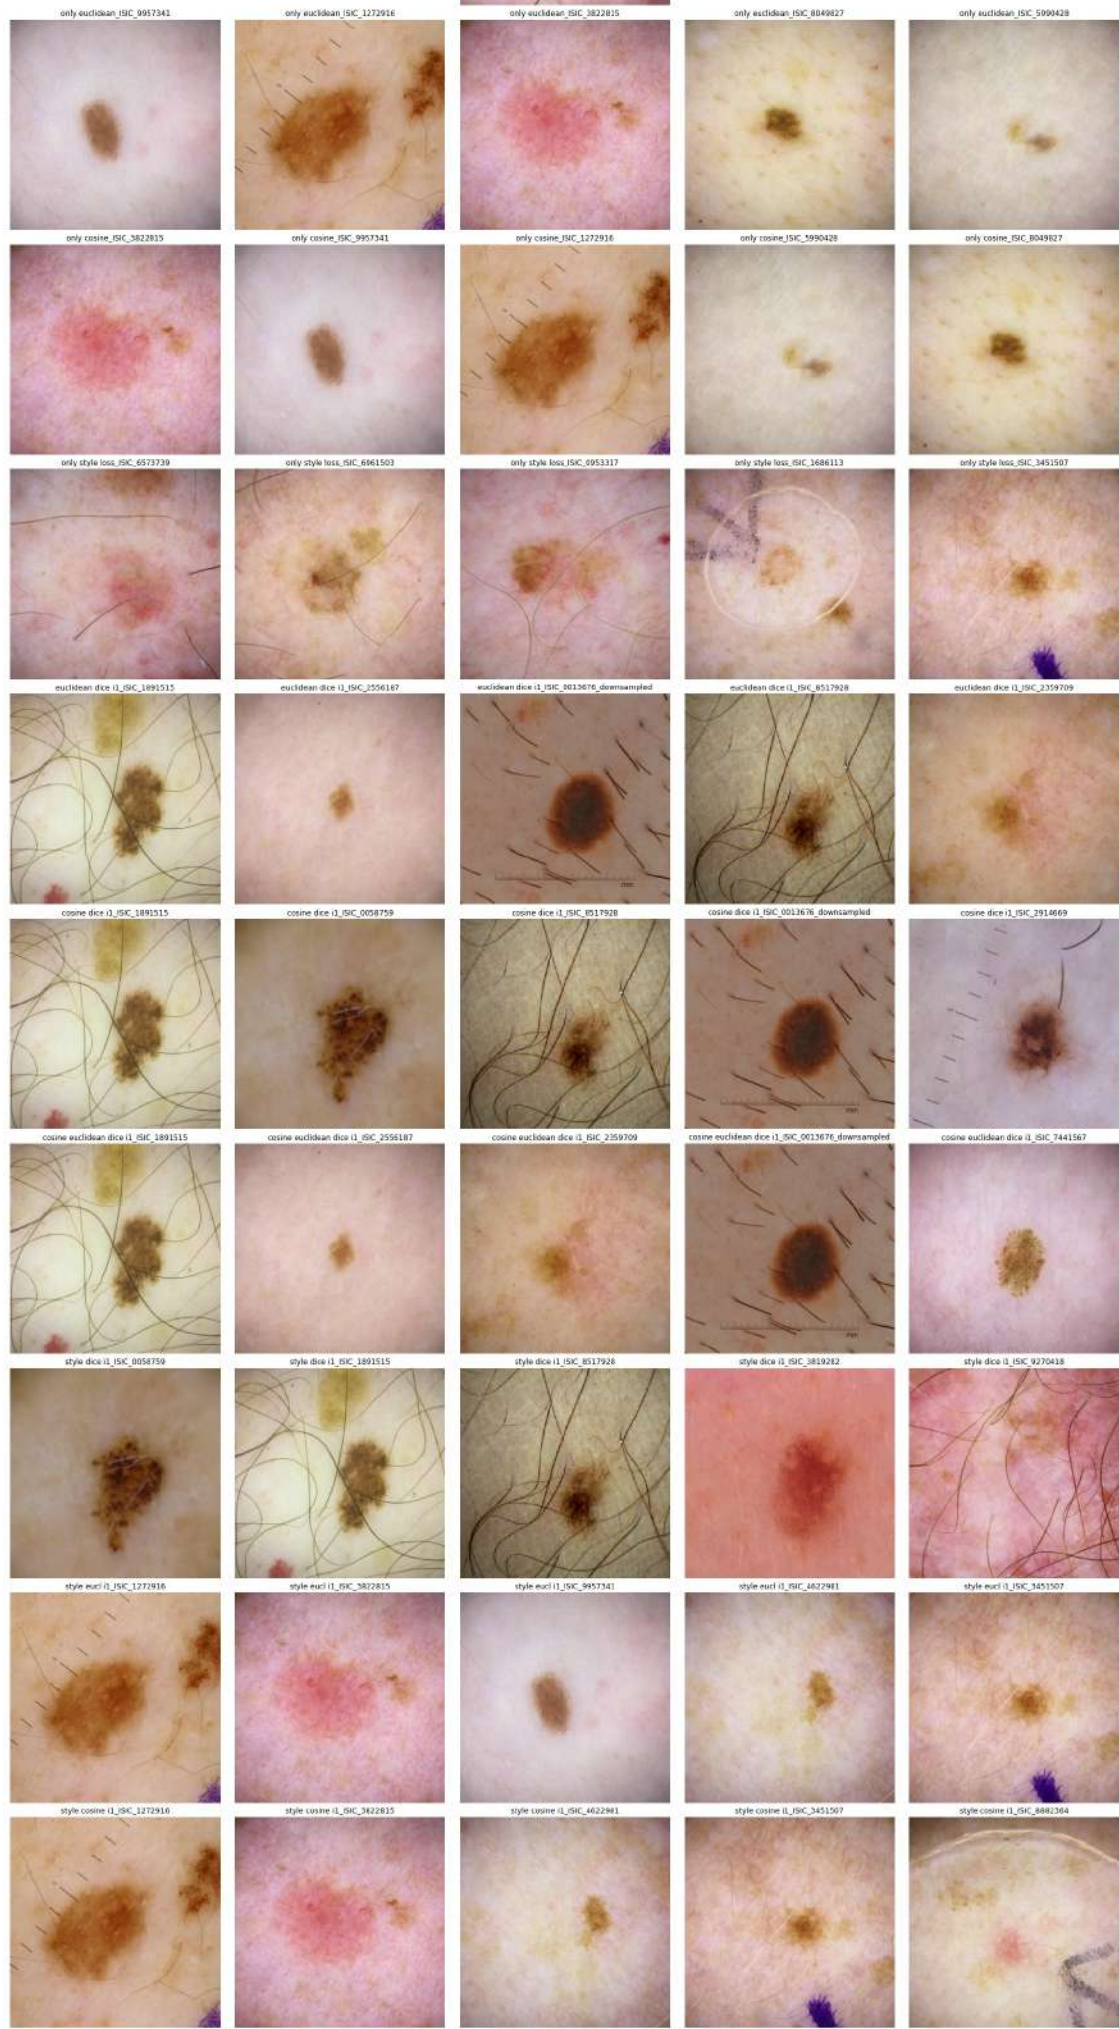

Input image - ISIC\_0018301

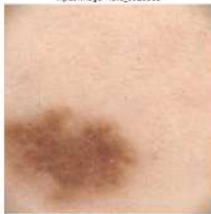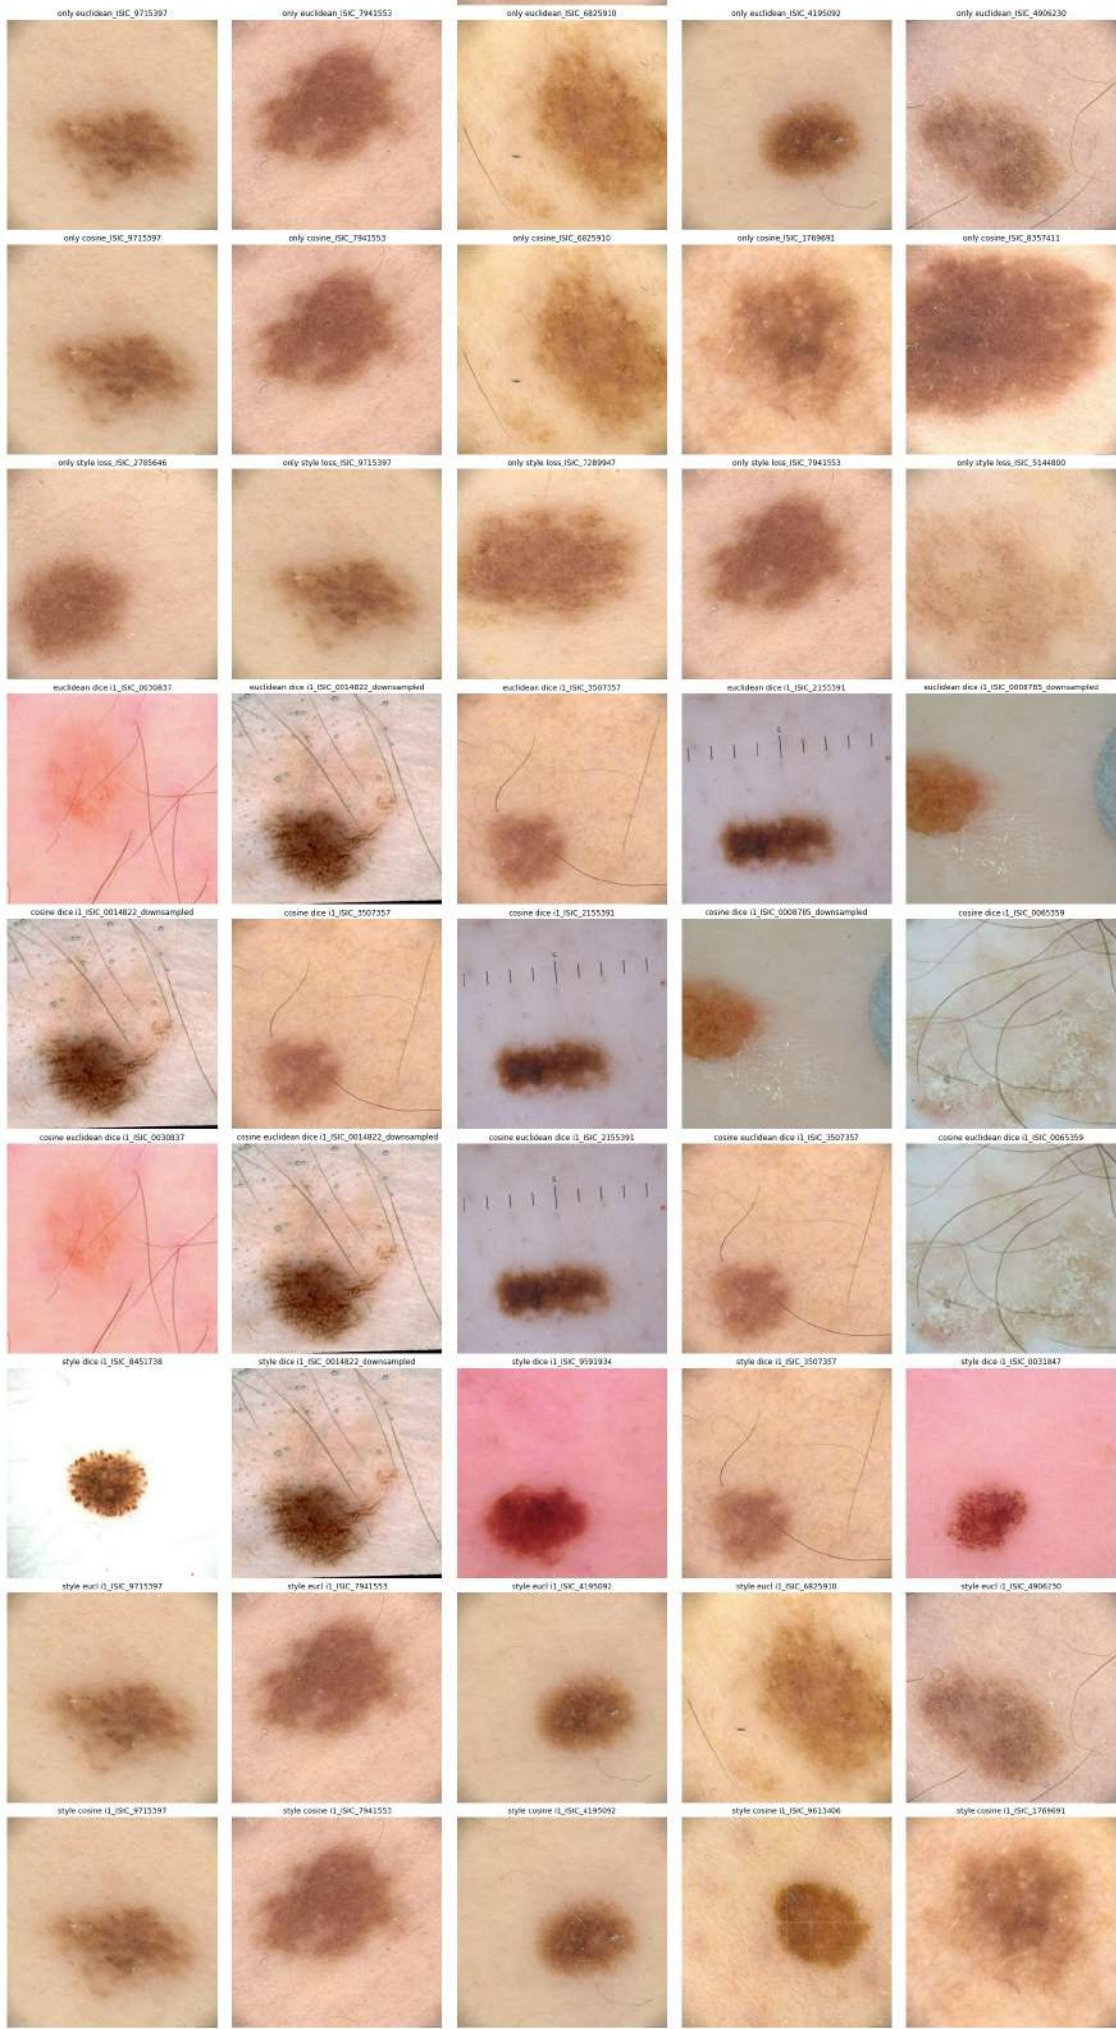

Input image - ISIC\_0843626

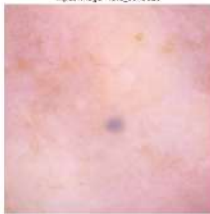

only euclidean\_ISIC\_6747026

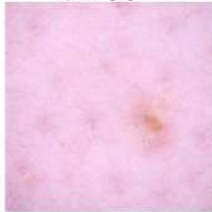

only euclidean\_ISIC\_8510945

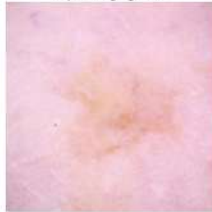

only euclidean\_ISIC\_9007813

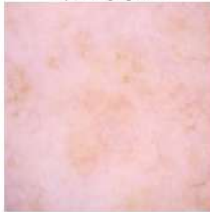

only euclidean\_ISIC\_1346695

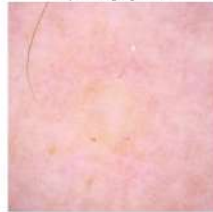

only euclidean\_ISIC\_0958562

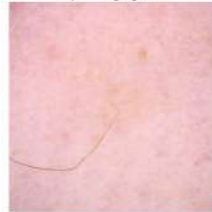

only cosine\_ISIC\_3289574

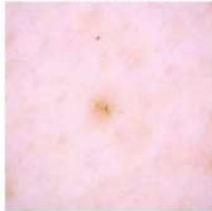

only cosine\_ISIC\_0509538

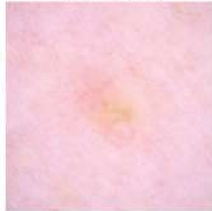

only cosine\_ISIC\_7497699

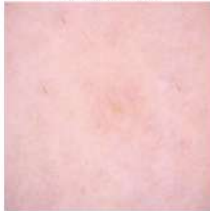

only cosine\_ISIC\_4236274

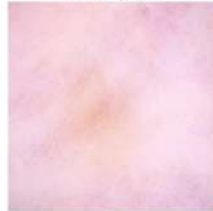

only cosine\_ISIC\_1344757

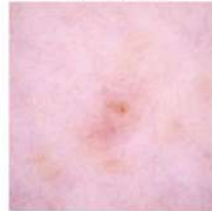

only style loss\_ISIC\_9649398

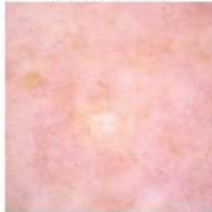

only style loss\_ISIC\_4675148

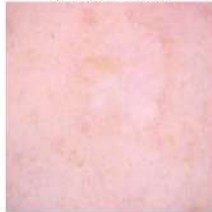

only style loss\_ISIC\_4385462

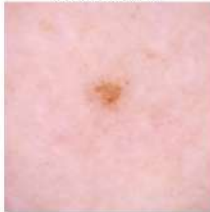

only style loss\_ISIC\_2377475

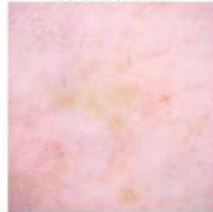

only style loss\_ISIC\_1445957

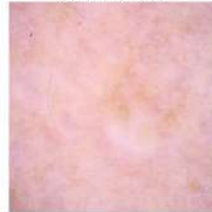

euclidean dice l1\_ISIC\_0058177

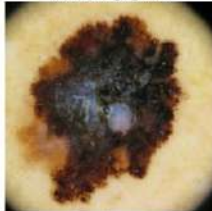

euclidean dice l1\_ISIC\_4973666

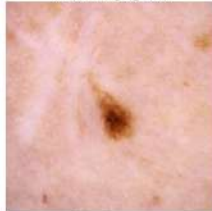

euclidean dice l1\_ISIC\_3599125

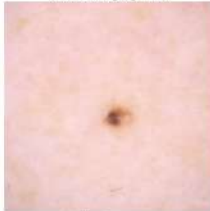

euclidean dice l1\_ISIC\_7030404

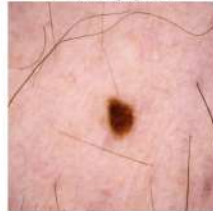

euclidean dice l1\_ISIC\_6783107

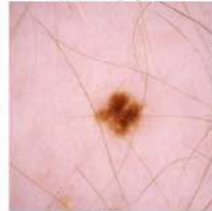

cosine dice l1\_ISIC\_4973666

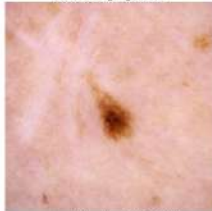

cosine dice l1\_ISIC\_3599125

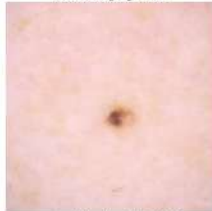

cosine dice l1\_ISIC\_8168507

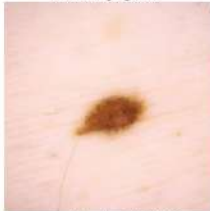

cosine dice l1\_ISIC\_8642671

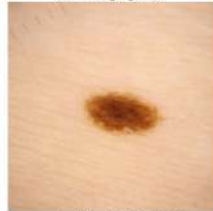

cosine dice l1\_ISIC\_3474609

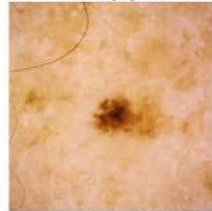

cosine euclidean dice l1\_ISIC\_0058177

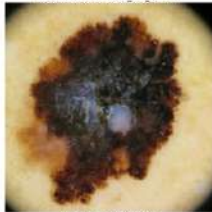

cosine euclidean dice l1\_ISIC\_4973666

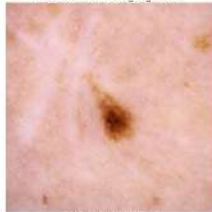

cosine euclidean dice l1\_ISIC\_3599125

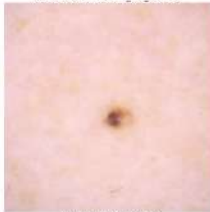

cosine euclidean dice l1\_ISIC\_7030404

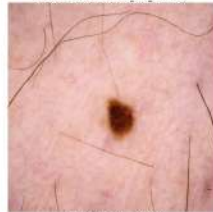

cosine euclidean dice l1\_ISIC\_6783107

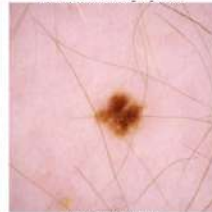

style dice l1\_ISIC\_9450306

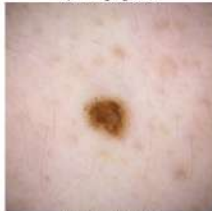

style dice l1\_ISIC\_4973666

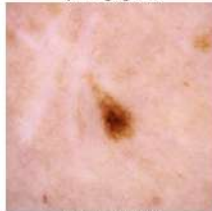

style dice l1\_ISIC\_8168507

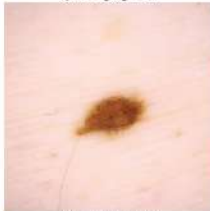

style dice l1\_ISIC\_3599125

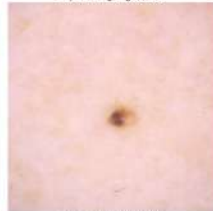

style dice l1\_ISIC\_0030858

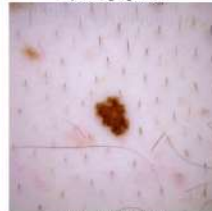

style eucl l1\_ISIC\_6747026

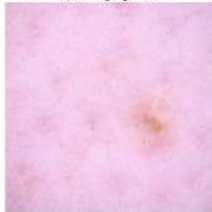

style eucl l1\_ISIC\_8510945

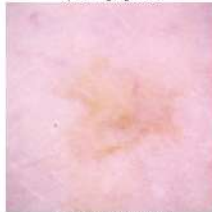

style eucl l1\_ISIC\_9007813

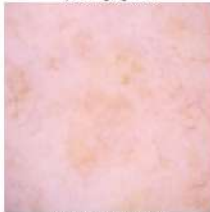

style eucl l1\_ISIC\_1346695

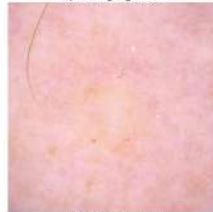

style eucl l1\_ISIC\_0958562

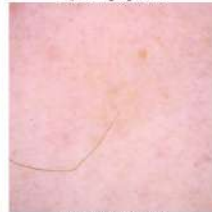

style cosine l1\_ISIC\_7497699

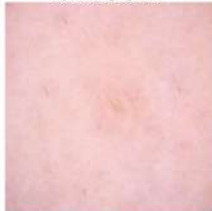

style cosine l1\_ISIC\_8330161

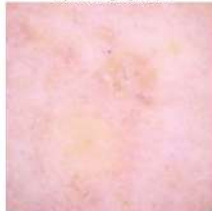

style cosine l1\_ISIC\_0509538

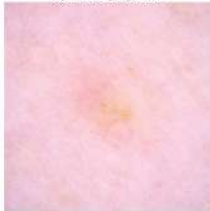

style cosine l1\_ISIC\_1344757

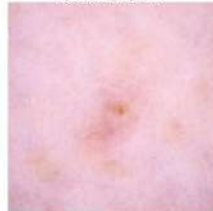

style cosine l1\_ISIC\_9007813

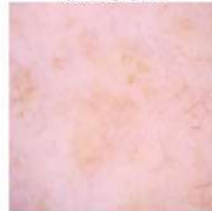

input image - ISIC\_0854582

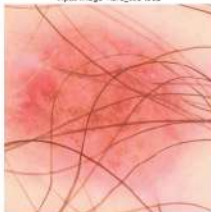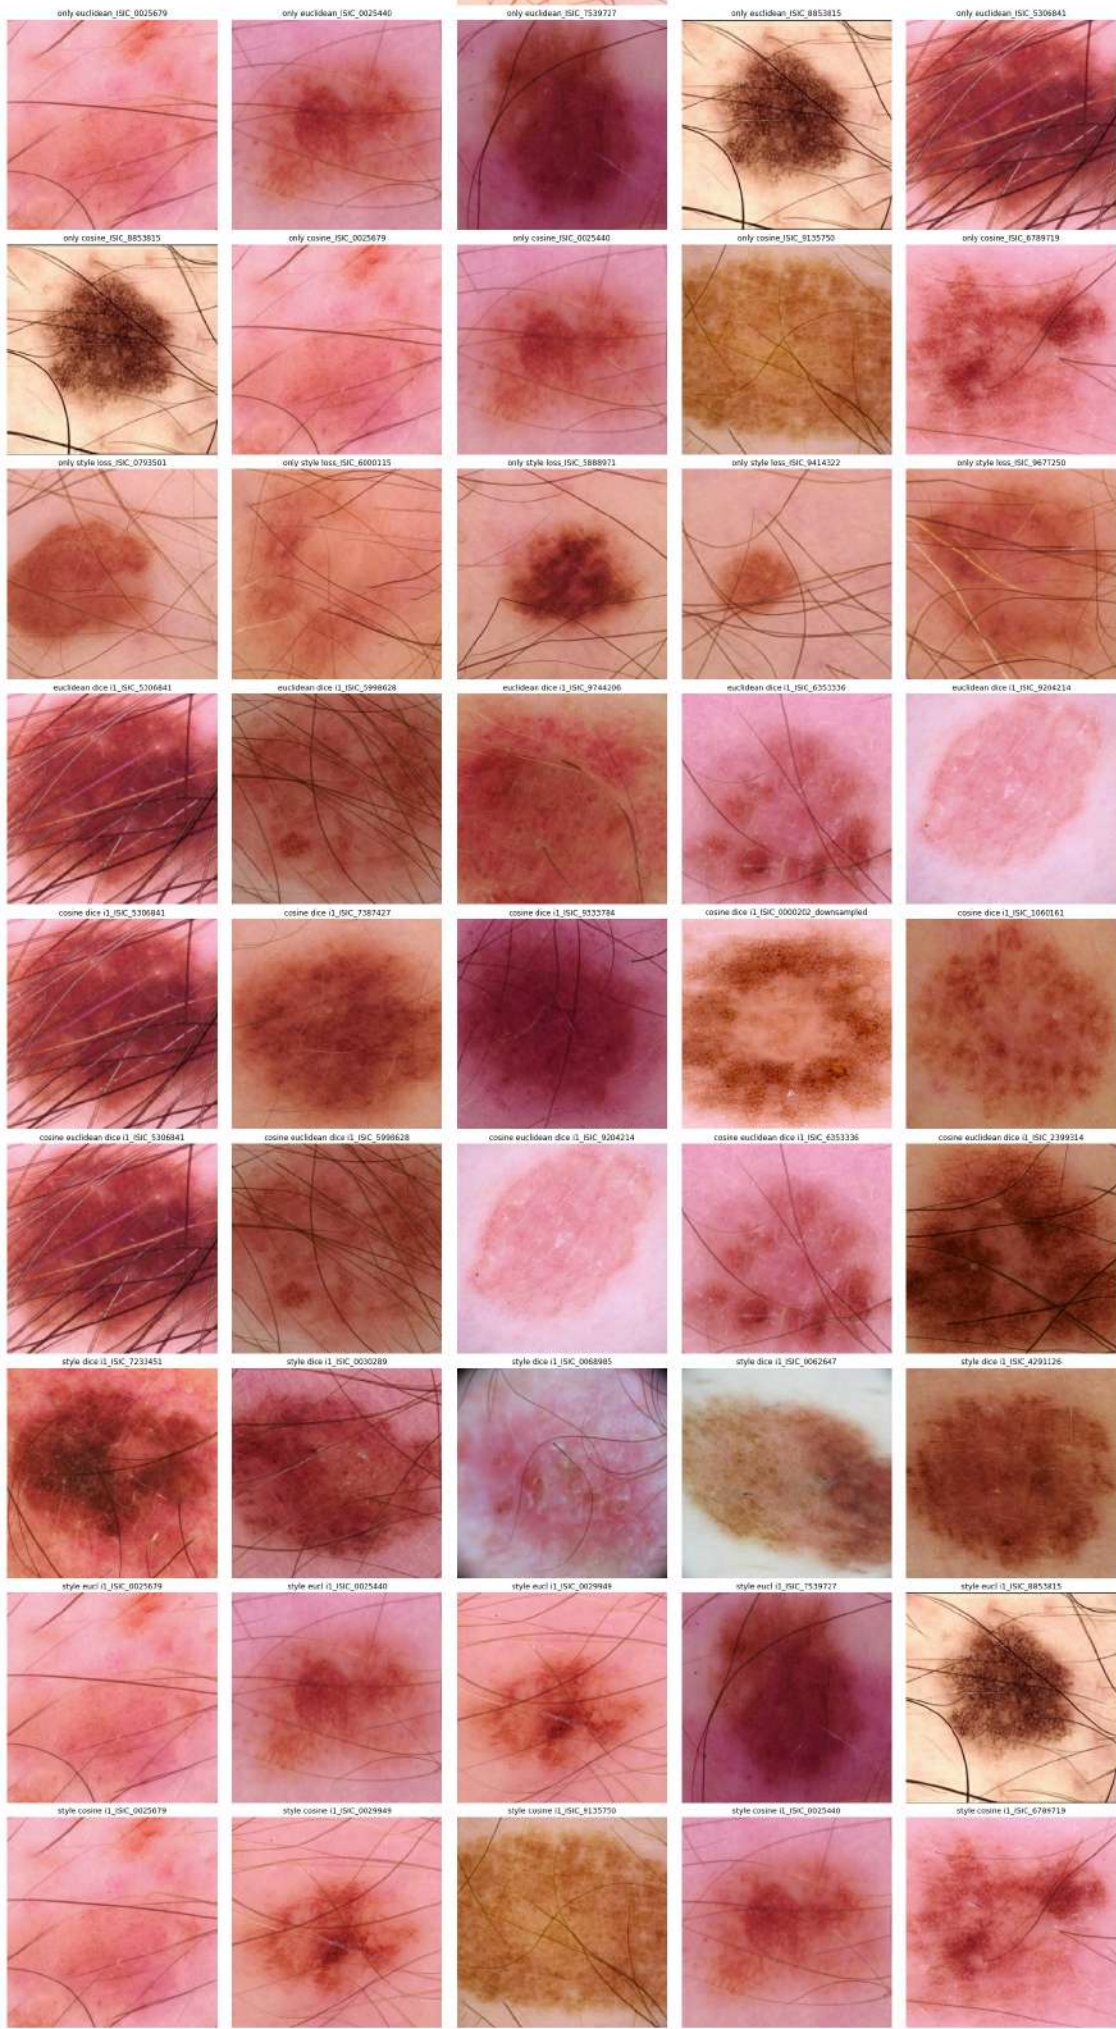

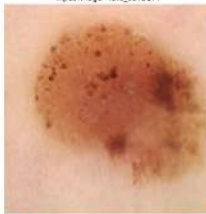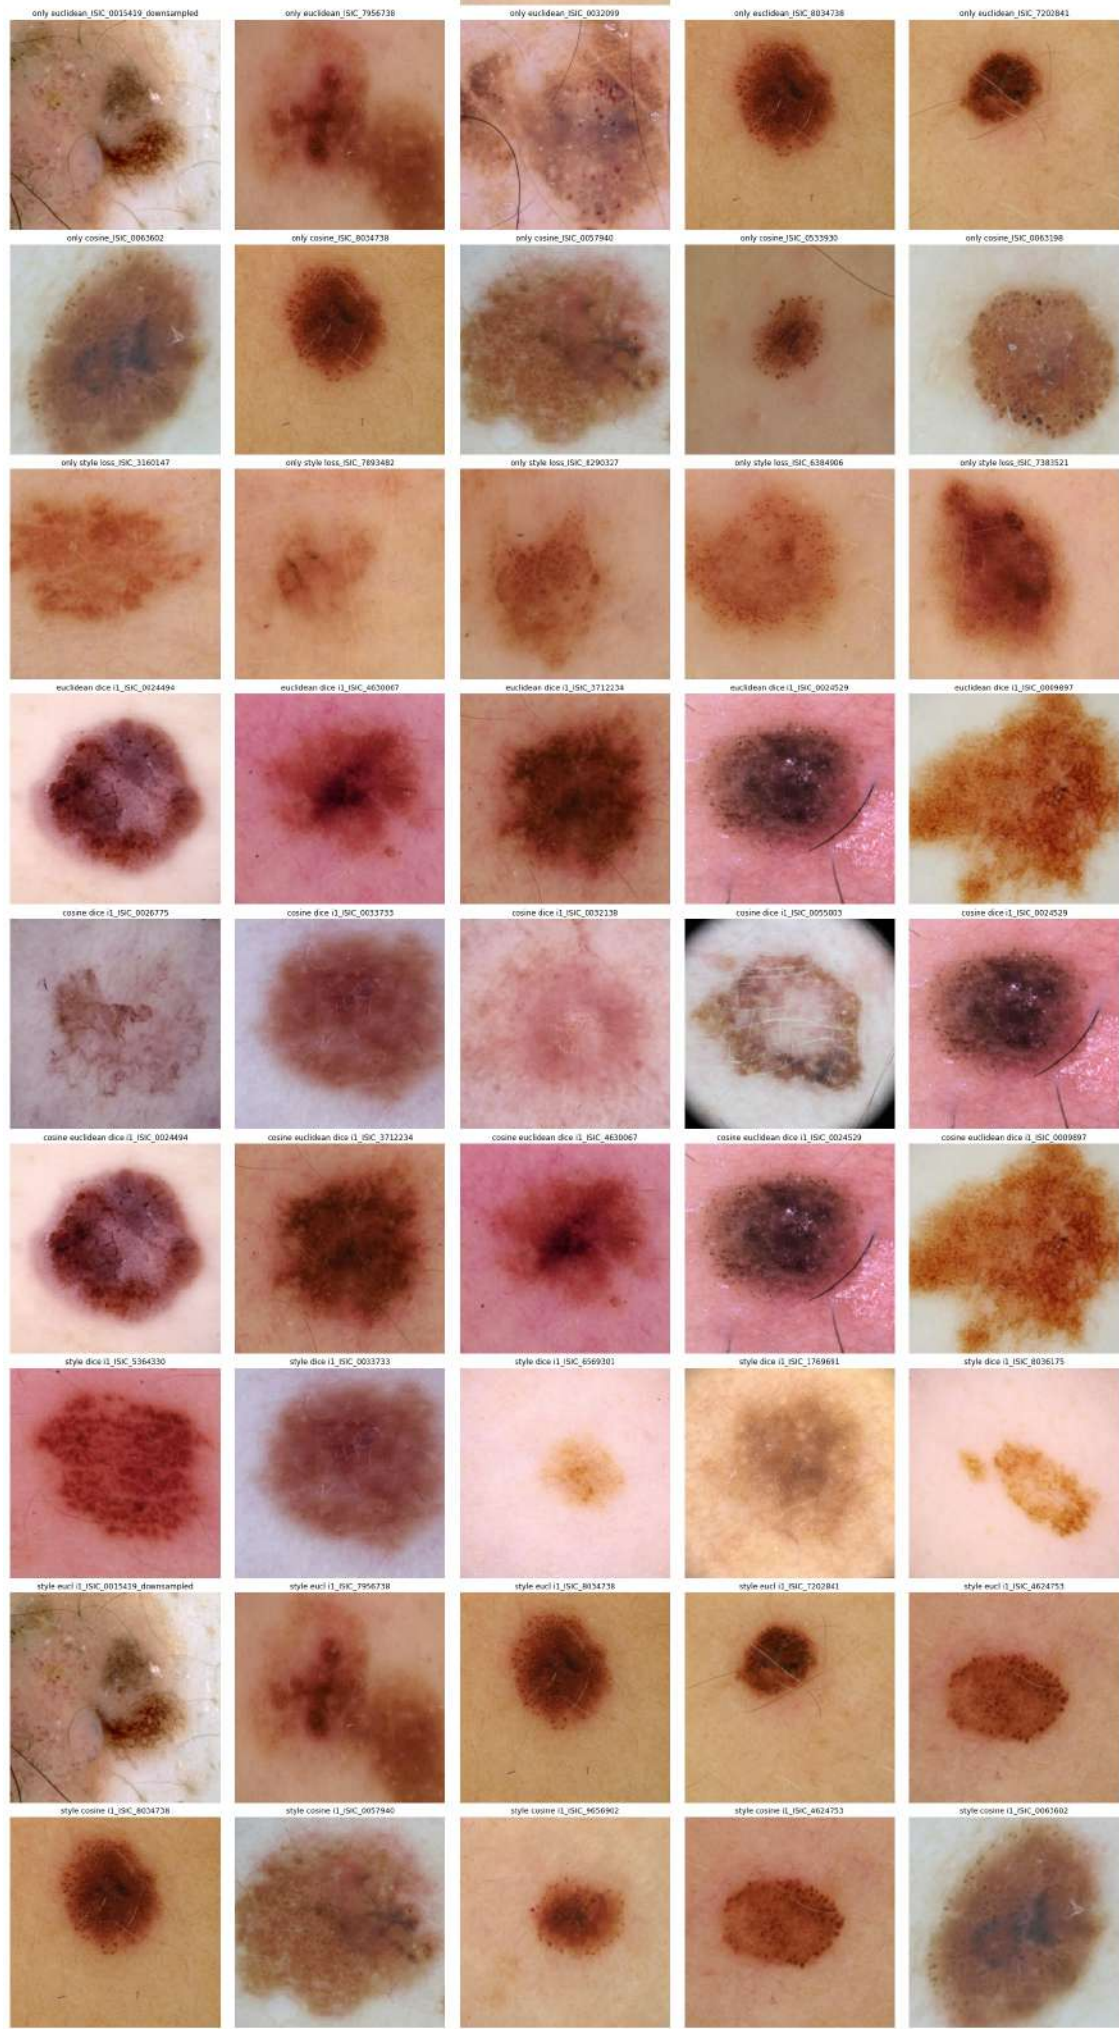

Input image - ISIC\_0896427

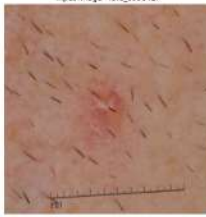

only euclidean\_ISIC\_3956937

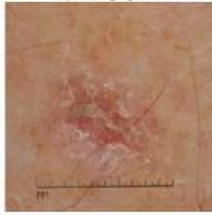

only euclidean\_ISIC\_2006443

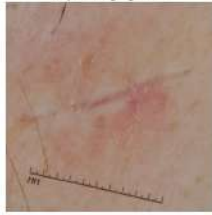

only euclidean\_ISIC\_2283111

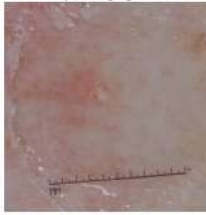

only euclidean\_ISIC\_9482039

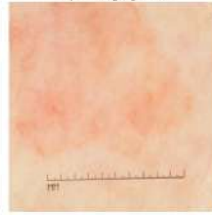

only euclidean\_ISIC\_0012240\_downsampled

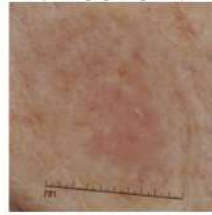

only cosine\_ISIC\_3956937

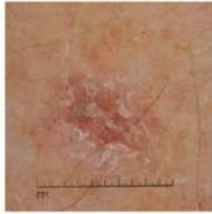

only cosine\_ISIC\_8138409

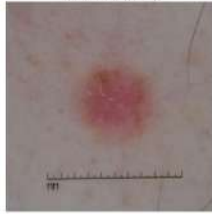

only cosine\_ISIC\_2006443

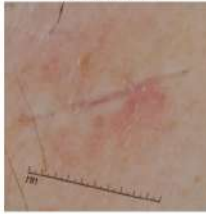

only cosine\_ISIC\_0012240\_downsampled

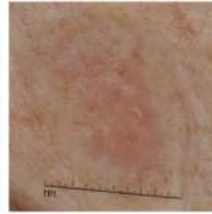

only cosine\_ISIC\_1084298

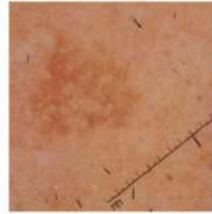

only style loss\_ISIC\_8652341

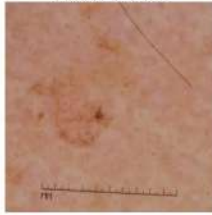

only style loss\_ISIC\_0012288\_downsampled

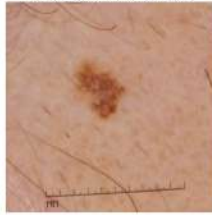

only style loss\_ISIC\_4545751

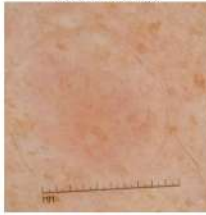

only style loss\_ISIC\_0012254\_downsampled

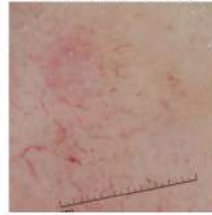

only style loss\_ISIC\_6555039

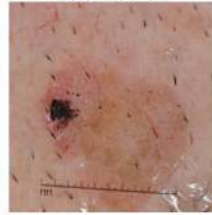

euclidean dice l1\_ISIC\_0011343

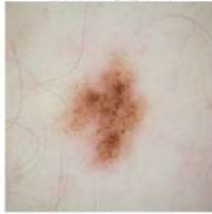

euclidean dice l2\_ISIC\_0059803

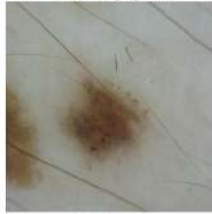

euclidean dice l1\_ISIC\_0058464

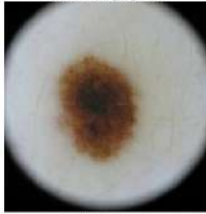

euclidean dice l1\_ISIC\_0009884

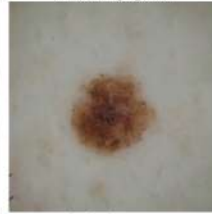

euclidean dice l1\_ISIC\_0069295

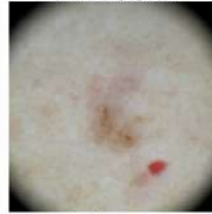

cosine dice l1\_ISIC\_0058464

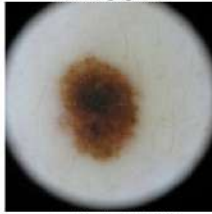

cosine dice l2\_ISIC\_0009884

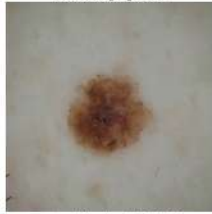

cosine dice l1\_ISIC\_0027523

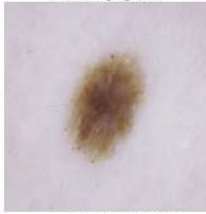

cosine dice l1\_ISIC\_0011343

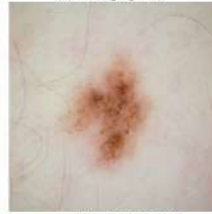

cosine dice l1\_ISIC\_0059803

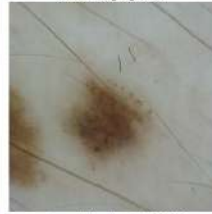

cosine euclidean dice l1\_ISIC\_0011343

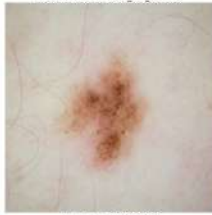

cosine euclidean dice l1\_ISIC\_0058464

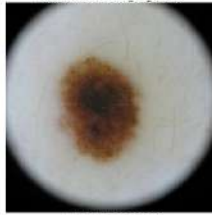

cosine euclidean dice l1\_ISIC\_0009884

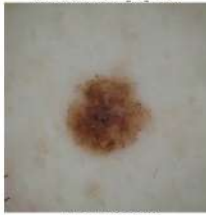

cosine euclidean dice l1\_ISIC\_0059803

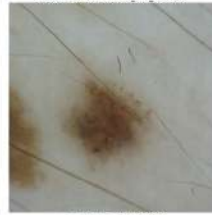

cosine euclidean dice l1\_ISIC\_0069295

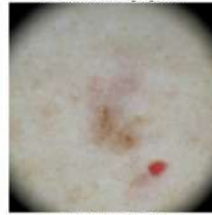

style dice l1\_ISIC\_9191776

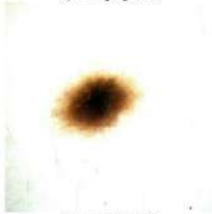

style dice l1\_ISIC\_1899522

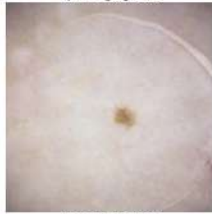

style dice l1\_ISIC\_2766031

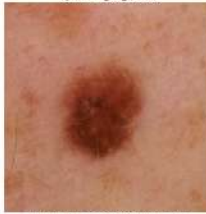

style dice l1\_ISIC\_0027523

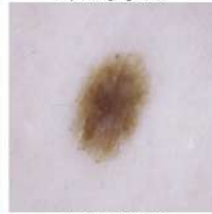

style dice l1\_ISIC\_9541491

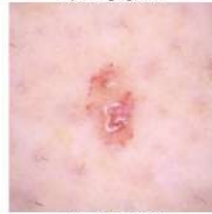

style eurl l1\_ISIC\_3956937

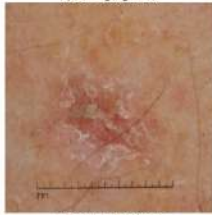

style eurl l1\_ISIC\_2006443

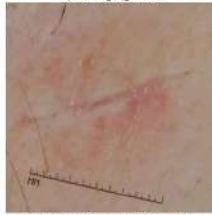

style eurl l1\_ISIC\_0012240\_downsampled

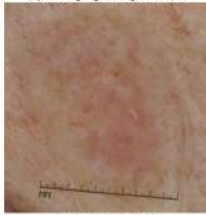

style eurl l1\_ISIC\_2283111

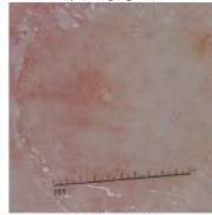

style eurl l1\_ISIC\_9649028

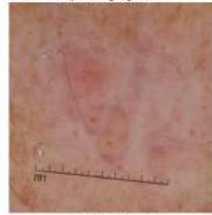

style cosine l1\_ISIC\_3956937

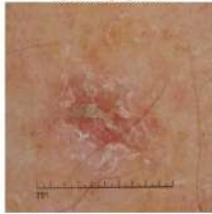

style cosine l1\_ISIC\_0012240\_downsampled

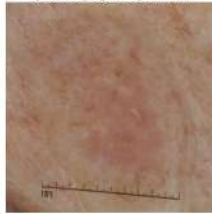

style cosine l1\_ISIC\_9649028

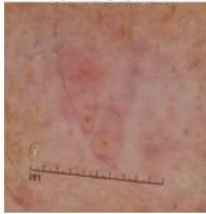

style cosine l1\_ISIC\_7186503

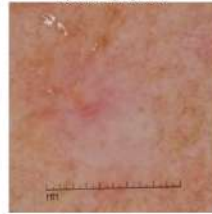

style cosine l1\_ISIC\_4545751

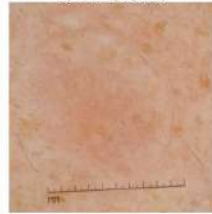

Supplement: Supplementary file 1 [file Final_results.pdf]
